# Supplementary material for: Firm Heterogeneity, Market Power and Macroeconomic Fragility
Source: arXiv:2205.03908 source file (2024-05-10)
Supplement: Supplementary file 1 [file SupplementaryMaterial.tex]

\newpage
\begin{center}
    
{\huge {Appendix B} \\\large{Supplementary Material for \\\textit{Firm Heterogeneity, Market Power and Macroeconomic Fragility} }\\ Not for Publication}
\end{center}

\raggedright
\justify

\setcounter{page}{1}
\setcounter{section}{0}
\setcounter{figure}{0}
\setcounter{table}{0}
\setcounter{lemma}{0}

\makeatletter
\@addtoreset{section}{mysection}
\makeatother

\section[No Product Differentiation]{Industry Equilibrium with $\eta=1$}\label{proofs_appendixB}

\paragraph{Equilibrium Price and Output}
Suppose that $\eta=1$. When $n$ firms produce, we have a system of $n$ first order conditions
\begin{align}
p\left[1-\left(1-\rho\right)s_{j}\right]=\dfrac{\Theta}{\gamma_{j}}
\end{align}
Dividing the first order condition of firm $j$ by that of firm $1$
we obtain
\begin{align}
 %& \dfrac{1-\left(1-\rho\right)s_{j}}{1-\left(1-\rho\right)s_{1}}=\dfrac{\gamma_{1}}{\gamma_{j}}\\
%\Leftrightarrow & 1-\left(1-\rho\right)s_{j}=\dfrac{\gamma_{1}}{\gamma_{j}}\left[1-\left(1-\rho\right)s_{1}\right]\\
%\Leftrightarrow & 
s_{j}=\dfrac{1}{\left(1-\rho\right)}\left\{ 1-\dfrac{\gamma_{1}}{\gamma_{j}}\left[1-\left(1-\rho\right)s_{1}\right]\right\} 
\end{align}
Note that
\begin{align}
  \stackrel[k=1]{n}{\sum}s_{k}=1
 %\\
%\Leftrightarrow & \stackrel[k=1]{n}{\sum}\dfrac{1}{\left(1-\rho\right)}\left\{ 1-\dfrac{\gamma_{1}}{\gamma_{k}}\left[1-\left(1-\rho\right)s_{1}\right]\right\} =1\\
%\Leftrightarrow & n-\gamma_{1}\left[1-\left(1-\rho\right)s_{1}\right]\stackrel[k=1]{n}{\sum}\dfrac{1}{\gamma_{k}}=1-\rho\\
\Rightarrow  \dfrac{n-\left(1-\rho\right)}{\stackrel[k=1]{n}{\sum}\dfrac{1}{\gamma_{k}}}=\gamma_{1}\left[1-\left(1-\rho\right)s_{1}\right]
\end{align}
Plugging the last equation into the first order condition of firm
$1$ we obtain
\begin{align}
 %& p\dfrac{n-\left(1-\rho\right)}{\sum\limits_{k=1}^{n}\dfrac{1}{\gamma_{k}}}=\Theta\\
%\Leftrightarrow &
p=\dfrac{\sum\limits_{k=1}^{n}\dfrac{1}{\gamma_{k}}}{n-\left(1-\rho\right)}\Theta
\end{align}
Total output is hence equal to 
\begin{align}
 & y=p^{-\frac{1}{1-\rho}}Y=\left[\dfrac{\sum\limits_{k=1}^{n}\dfrac{1}{\gamma_{k}}}{n-\left(1-\rho\right)}\Theta\right]^{-\frac{1}{1-\rho}}Y
\end{align}

\paragraph{Market Shares}

Plugging the previous equation into the first order condition of firm
$j$ we have
\begin{align}
% & 1-\left(1-\rho\right)s_{j}=\dfrac{n-\left(1-\rho\right)}{\sum\limits_{k=1}^{n}\dfrac{1}{\gamma_{k}}}\dfrac{1}{\gamma_{j}}\\
%\Leftrightarrow & 
s_{j}=\dfrac{1}{1-\rho}\left[1-\dfrac{n-\left(1-\rho\right)}{\sum\limits_{k=1}^{n}\dfrac{1}{\gamma_{k}}}\dfrac{1}{\gamma_{j}}\right]
\end{align}
It is easy to verify that each firm's market share decreases in the
total number of active firms. To see this, suppose that the number
of firms increases from $n$ to $n+1$. The new entrant will have
a market share
\begin{align}
s_{n+1}=\dfrac{1}{1-\rho}\left[1-\dfrac{n+1-\left(1-\rho\right)}{\sum\limits_{k=1}^{n+1}\dfrac{1}{\gamma_{k}}}\dfrac{1}{\gamma_{n+1}}\right]
\end{align}
which is non-negative provided that
\begin{equation}
\gamma_{n+1}\sum_{k=1}^{n+1}\dfrac{1}{\gamma_{k}}>n+1-\left(1-\rho\right)\label{eq:cond_mg_1}
\end{equation}
and below one given that
\begin{equation}
\gamma_{n+1}\sum_{k=1}^{n+1}\dfrac{1}{\gamma_{k}}<\dfrac{1}{\rho}\left[n+1-\left(1-\rho\right)\right]\label{eq:cond_mg_2}
\end{equation}
If we compare the market share of firm $j$ when there $n$ and $n+1$
firms in the market, we have
\begin{align}
 & s_{j}\left|_{n+1}\right.<s_{j}\left|_n\right.
%\Leftrightarrow & \dfrac{1}{1-\rho}\left[1-\dfrac{n+1-\left(1-\rho\right)}{\sum\limits_{k=1}^{n+1}\dfrac{1}{\gamma_{k}}}\dfrac{1}{\gamma_{j}}\right]<\dfrac{1}{1-\rho}\left[1-\dfrac{n-\left(1-\rho\right)}{\sum\limits_{k=1}^{n}\dfrac{1}{\gamma_{k}}}\dfrac{1}{\gamma_{j}}\right]\\
%\Leftrightarrow & \dfrac{n-\left(1-\rho\right)}{\sum\limits_{k=1}^{n}\dfrac{1}{\gamma_{k}}}<\dfrac{n+1-\left(1-\rho\right)}{\sum\limits_{k=1}^{n+1}\dfrac{1}{\gamma_{k}}}\\
%\Leftrightarrow & \left[n-\left(1-\rho\right)\right]\left(\dfrac{1}{\gamma_{n+1}}+\sum\limits_{k=1}^{n}\dfrac{1}{\gamma_{k}}\right)<\left[n+1-\left(1-\rho\right)\right]\sum\limits_{k=1}^{n}\dfrac{1}{\gamma_{k}}\\
%\Leftrightarrow & \left[n-\left(1-\rho\right)\right]\dfrac{1}{\gamma_{n+1}}<\sum\limits_{k=1}^{n}\dfrac{1}{\gamma_{k}}\\
\Leftrightarrow  \gamma_{n+1}\sum\limits_{k=1}^{n+1}\dfrac{1}{\gamma_{k}}>n-\left(1-\rho\right)
\end{align}
Note that the last condition is implied by (\ref{eq:cond_mg_1}).

\paragraph{Profits}%\label{subsec:Profits}}

When there are $n$ active firms, type $\gamma_{j}$ makes production profits
\begin{align}
\Pi\left(\gamma_{j},n,\Gamma,\Theta,Y\right) %& =\left(p-\dfrac{\Theta}{\gamma_{j}}\right)s_{j}\:y_{j} \\
 & = \underbrace{\dfrac{1}{1-\rho}\left[1-\dfrac{n-\left(1-\rho\right)}{\sum\limits_{k=1}^{n}\dfrac{1}{\gamma_{k}}}\dfrac{1}{\gamma_{j}}\right]^{2}\left[\dfrac{n-\left(1-\rho\right)}{\sum\limits_{k=1}^{n}\dfrac{1}{\gamma_{k}}}\right]^{\frac{\rho}{1-\rho}}}_{\equiv \varLambda\left(\gamma_{j},n,\Gamma\right)}\Theta^{-\frac{\rho}{1-\rho}}Y
\end{align}
\begin{lemma}
\label{lemma:(Profit-Function)} When $\eta=1$, the profit function \textup{$\Pi\left(j,n_{it},\Gamma_{i},X_{t}\right)$}
satisfies
\begin{align} 
1) & \dfrac{\partial\Pi\left(j,n_{it},\Gamma_{i},X_{t}\right)}{\partial Y_{t}}\vphantom{\vphantom{\dfrac{\dfrac{1}{1}}{\frac{_{1}}{1}}}}>0  \qquad 
2) & \dfrac{\partial\Pi\left(j,n_{it},\Gamma_{i},X_{t}\right)}{\partial n_{it}}\vphantom{\vphantom{\dfrac{\dfrac{1}{1}}{\frac{_{1}}{1}}}}<0  \quad,\;n_{it}>j \\
3) & \dfrac{\partial\Pi\left(j,n_{it},\Gamma_{i},X_{t}\right)}{\partial\gamma_{ij}}\vphantom{\dfrac{\dfrac{1}{1}}{\frac{_{1}}{1}}}>0 \qquad
4) & \dfrac{\partial\Pi\left(j,n_{it},\Gamma_{i},X_{t}\right)}{\partial\gamma_{ik}}\vphantom{\vphantom{\dfrac{\dfrac{1}{1}}{\frac{_{1}}{1}}}}<0  \quad,\;\forall k\neq j.
\end{align}
\end{lemma}
\begin{proof} [Proof of Lemma \ref{lemma:(Profit-Function)}]
We start by showing that $\Pi\left(\cdot\right)$ increases in $\gamma_{j}$
\begin{align}
 & 2\left[1-\dfrac{n-\left(1-\rho\right)}{\sum\limits_{k=1}^{n}\dfrac{1}{\gamma_{k}}}\dfrac{1}{\gamma_{j}}\right]^{-1}\left\{ -\dfrac{-\left[n-\left(1-\rho\right)\right]\left[-\left(\dfrac{1}{\gamma_{j}}\right)^{2}\right]}{\left(\sum\limits_{k=1}^{n}\dfrac{1}{\gamma_{k}}\right)^{2}}\dfrac{1}{\gamma_{j}}+\dfrac{n-\left(1-\rho\right)}{\sum\limits_{k=1}^{n}\dfrac{1}{\gamma_{k}}}\left(\dfrac{1}{\gamma_{j}}\right)^{2}\right\} + \\
 & \dfrac{\rho}{1-\rho}\left[\dfrac{n-\left(1-\rho\right)}{\sum\limits_{k=1}^{n}\dfrac{1}{\gamma_{k}}}\right]^{-1}\dfrac{-\left[n-\left(1-\rho\right)\right]\left[-\left(\dfrac{1}{\gamma_{j}}\right)^{2}\right]}{\left(\sum\limits_{k=1}^{n}\dfrac{1}{\gamma_{k}}\right)^{2}}>0\\
%\Leftrightarrow & 2\left[1-\dfrac{n-\left(1-\rho\right)}{\sum\limits_{k=1}^{n}\dfrac{1}{\gamma_{k}}}\dfrac{1}{\gamma_{j}}\right]^{-1}\left\{ -\dfrac{1}{\left(\sum\limits_{k=1}^{n}\dfrac{1}{\gamma_{k}}\right)^{2}}\dfrac{1}{\gamma_{j}}+\dfrac{1}{\sum\limits_{k=1}^{n}\dfrac{1}{\gamma_{k}}}\right\} + \\
%& \dfrac{\rho}{1-\rho}\left[\dfrac{n-\left(1-\rho\right)}{\sum\limits_{k=1}^{n}\dfrac{1}{\gamma_{k}}}\right]^{-1}\dfrac{1}{\left(\sum\limits_{k=1}^{n}\dfrac{1}{\gamma_{k}}\right)^{2}}>0\\
%\Leftrightarrow & 2\left[1-\dfrac{n-\left(1-\rho\right)}{\sum\limits_{k=1}^{n}\dfrac{1}{\gamma_{k}}}\dfrac{1}{\gamma_{j}}\right]^{-1}\left\{ -\dfrac{1}{\gamma_{j}}+\sum\limits_{k=1}^{n}\dfrac{1}{\gamma_{k}}\right\} +\dfrac{\rho}{1-\rho}\left[\dfrac{n-\left(1-\rho\right)}{\sum\limits_{k=1}^{n}\dfrac{1}{\gamma_{k}}}\right]^{-1}\dfrac{1}{\left(\sum\limits_{k=1}^{n}\dfrac{1}{\gamma_{k}}\right)^{2}}>0\\
\Leftrightarrow & 2\left[1-\dfrac{n-\left(1-\rho\right)}{\sum\limits_{k=1}^{n}\dfrac{1}{\gamma_{k}}}\dfrac{1}{\gamma_{j}}\right]^{-1}\left(\sum\limits_{k\neq j}^{n}\dfrac{1}{\gamma_{k}}\right)+\dfrac{\rho}{1-\rho}\left[\dfrac{n-\left(1-\rho\right)}{\sum\limits_{k=1}^{n}\dfrac{1}{\gamma_{k}}}\right]^{-1}>0
\end{align}
To prove points (ii) and (iii) it suffices to show that $\varLambda\left(\cdot\right)$
is decreasing in $[{n-\left(1-\rho\right)}]/\left[{\sum\limits_{k=1}^{n}\dfrac{1}{\gamma_{k}}}\right]$
\begin{align}
 & 2\left[1-\dfrac{n-\left(1-\rho\right)}{\sum\limits_{k=1}^{n}\dfrac{1}{\gamma_{k}}}\dfrac{1}{\gamma_{j}}\right]^{-1}\left(-\dfrac{1}{\gamma_{j}}\right)+\dfrac{\rho}{1-\rho}\left[\dfrac{n-\left(1-\rho\right)}{\sum\limits_{k=1}^{n}\dfrac{1}{\gamma_{k}}}\right]^{-1}<0\\
%\Leftrightarrow & \dfrac{\rho}{1-\rho}\left[1-\dfrac{n-\left(1-\rho\right)}{\sum\limits_{k=1}^{n}\dfrac{1}{\gamma_{k}}}\dfrac{1}{\gamma_{j}}\right]<2\left[\dfrac{n-\left(1-\rho\right)}{\sum\limits_{k=1}^{n}\dfrac{1}{\gamma_{k}}}\right]\dfrac{1}{\gamma_{j}}\\
%\Leftrightarrow & \dfrac{\rho}{1-\rho}<\left(2+\frac{\rho}{1-\rho}\right)\left[\dfrac{n-\left(1-\rho\right)}{\sum\limits_{k=1}^{n}\dfrac{1}{\gamma_{k}}}\right]\dfrac{1}{\gamma_{j}}\\
%\Leftrightarrow & \rho<\left(2-\rho\right)\left[\dfrac{n-\left(1-\rho\right)}{\sum\limits_{k=1}^{n}\dfrac{1}{\gamma_{k}}}\right]\dfrac{1}{\gamma_{j}}\\
\Leftrightarrow & \gamma_{j}\sum\limits_{k=1}^{n}\dfrac{1}{\gamma_{k}}<\dfrac{2-\rho}{\rho}\left[n-\left(1-\rho\right)\right]
\end{align}
The last condition is implied by (\ref{eq:cond_mg_2}).
\end{proof}

\section{Derivations: General Equilibrium}\label{sec:GEderivations}

\subsection{Aggregate TFP \label{subsec:Aggregate-TFP} }
Aggregate TFP is given by
\begin{equation}
\Phi\left(\mathbf{\Gamma},\mathbf{N}_{t}\right)=\left[\sum_{i=1}^{I}\left(\sum_{j=1}^{n_{it}}\omega_{ijt}^{\eta}\right)^{\frac{\rho}{\eta}}\right]^{\frac{1}{\rho}}\left(\sum_{i=1}^{I}\sum_{j=1}^{n_{it}}\dfrac{\omega_{ijt}}{\tau_{ijt}}\right)^{-1},\label{eq:agg_tfp}
\end{equation}
where
\begin{align}
\omega_{ijt}\coloneqq\left[\sum_{k=1}^{n_{it}}\left(\dfrac{\mu_{ikt}}{\tau_{ikt}}\right)^{\frac{\eta}{1-\eta}}\right]^{\frac{\eta-\rho}{\eta}\frac{1}{1-\rho}}\left(\dfrac{\tau_{ijt}}{\mu_{ijt}}\right)^{\frac{1}{1-\eta}}.
\end{align}

\subsection{Factor Prices and Factor Shares \label{subsec:Factor-Prices} }
We can aggregate firms' best responses, given by equation (\ref{eq:firm_FOC}), to find an expression for the aggregate factor cost index. Given a $\left(I\times M\right)$
matrix of productivity draws $\mathbf{A}_{t}$ and a vector of active firms $\mathbf{N}_{t} \equiv \left\{ n_{it}\right\}_{i=1}^{I}$, the equilibrium factor cost index is equal to
\begin{equation}
\Theta\left(\mathbf{A}_{t},\mathbf{N}_{t}\right)=\left\{ \sum_{i=1}^{I}\left[\sum_{j=1}^{n_{it}}\left(\dfrac{\tau_{ijt}}{\mu_{ijt}}\right)^{\frac{\eta}{1-\eta}}\right]^{\frac{1-\eta}{\eta}\frac{\rho}{1-\rho}}\right\} ^{\frac{1-\rho}{\rho}}.
\end{equation}

The aggregate factor share $\Omega\left(\cdot\right) = \left(W_{t}\,L_{t} + R_{t}\,K_{t} \right)/Y_{t} $ is equal to
\begin{equation}
\Omega\left(\mathbf{A}_{t},\mathbf{N}_{t}\right) = \dfrac{\Theta\left(\mathbf{A}_{t},\mathbf{N}_{t}\right)}{\Phi\left(\mathbf{A}_{t},\mathbf{N}_{t}\right)} .
\end{equation}

\subsection{Asymmetric Equilibrium\label{subsec:Asymmetric Equilibrium}}

When
\begin{align}
\overline{K}\left(\Gamma,n\right) <  K < \underline{K}\left(\Gamma,n+1\right)
\end{align}
there will be an asymmetric equilibrium at time $t+1$:
some industries will contain $n$ firms, whereas some industries will
contain $n+1$ firms. The fraction of industries with $n+1$ will
be pinned down by a zero profit condition for the marginal entrant
in an industry with $n+1$ firms
\begin{align}
\varLambda\left(\Gamma,\gamma_{n+1},n+1\right)\Theta^{-\frac{\rho}{1-\rho}}Y=c_{i}
\end{align}

The equilibrium is characterized by 4 variables: 
the fraction of the industries
with $n+1$ firms ($\eta$), aggregate output ($Y$), aggregate productivity ($\Phi$) and the aggregate cost index ($\Theta$). These 4 variables are pinned down by the following 4 equations

\begin{align}
Y=\Phi\left[\left(1-\alpha\right)\Theta\right]^{\frac{1-\alpha}{\nu+\alpha}}K^{\alpha\frac{1+\nu}{\nu+\alpha}}\\
\Phi=\dfrac{\left\{ \left(1-\eta\right)\left[\dfrac{n-\left(1-\rho\right)}{\sum\limits_{k=1}^{n}\dfrac{1}{\gamma_{1k}}}\right]^{\frac{\rho}{1-\rho}}+\eta\left[\dfrac{n+1-\left(1-\rho\right)}{\sum\limits_{k=1}^{n+1}\dfrac{1}{\gamma_{2k}}}\right]^{\frac{\rho}{1-\rho}}\right\} ^{\frac{1}{\rho}}}{\left(1-\eta\right)\left[\dfrac{n-\left(1-\rho\right)}{\sum\limits_{k=1}^{n}\dfrac{1}{\gamma_{1k}}}\right]^{\frac{1}{1-\rho}}\left(\sum\limits_{k=1}^{n}\dfrac{s_{1k}}{\gamma_{1k}}\right)+\eta\left[\dfrac{n+1-\left(1-\rho\right)}{\sum\limits_{k=1}^{n+1}\dfrac{1}{\gamma_{2k}}}\right]^{\frac{1}{1-\rho}}\left(\sum\limits_{k=1}^{n+1}\dfrac{s_{2k}}{\gamma_{2k}}\right)\vphantom{\left[\dfrac{\dfrac{\sum\limits_{k}^{n}\dfrac{1}{\gamma}}{1}}{\dfrac{\sum\limits_{k}^{n}\dfrac{1}{\gamma}}{1}}\right]}}\\
\Theta=\left\{ \left(1-\eta\right)\left[\dfrac{n-\left(1-\rho\right)}{\sum\limits_{k=1}^{n}\dfrac{1}{\gamma_{k}}}\right]^{\frac{\rho}{1-\rho}}+\eta\left[\dfrac{n+1-\left(1-\rho\right)}{\sum\limits_{k=1}^{n+1}\dfrac{1}{\gamma_{k}}}\right]^{\frac{\rho}{1-\rho}}\right\} ^{\frac{1-\rho}{\rho}}\vphantom{\left[\dfrac{\dfrac{\sum\limits_{k}^{n}\dfrac{1}{\gamma}}{1}}{\dfrac{\sum_{k}^{n}\dfrac{1}{\gamma}}{1}}\right]}\\
\varLambda\left(\Gamma,\gamma_{n+1},n+1\right)\Theta^{-\frac{\rho}{1-\rho}}Y=c_{i}
\end{align}

$s_{1k}$ is the market share of firm $k$ in an industry with $n$ firms, whereas $s_{2k}$ is the market share of firm $k$ in an industry with $n+1$ firms. They are defined in Appendix
\ref{proofs_appendixB}.

\section{The Baseline Model}\label{appendix:baseline-model}

\subsection*{Comparative Statics with $\uparrow \gamma_{1}$ and $\leftrightarrow \gamma_{2}$ (mean-increasing spread)}
\begin{figure}[H]
\centering{}
\hspace{-0.2cm}
 \includegraphics*[scale=0.475]{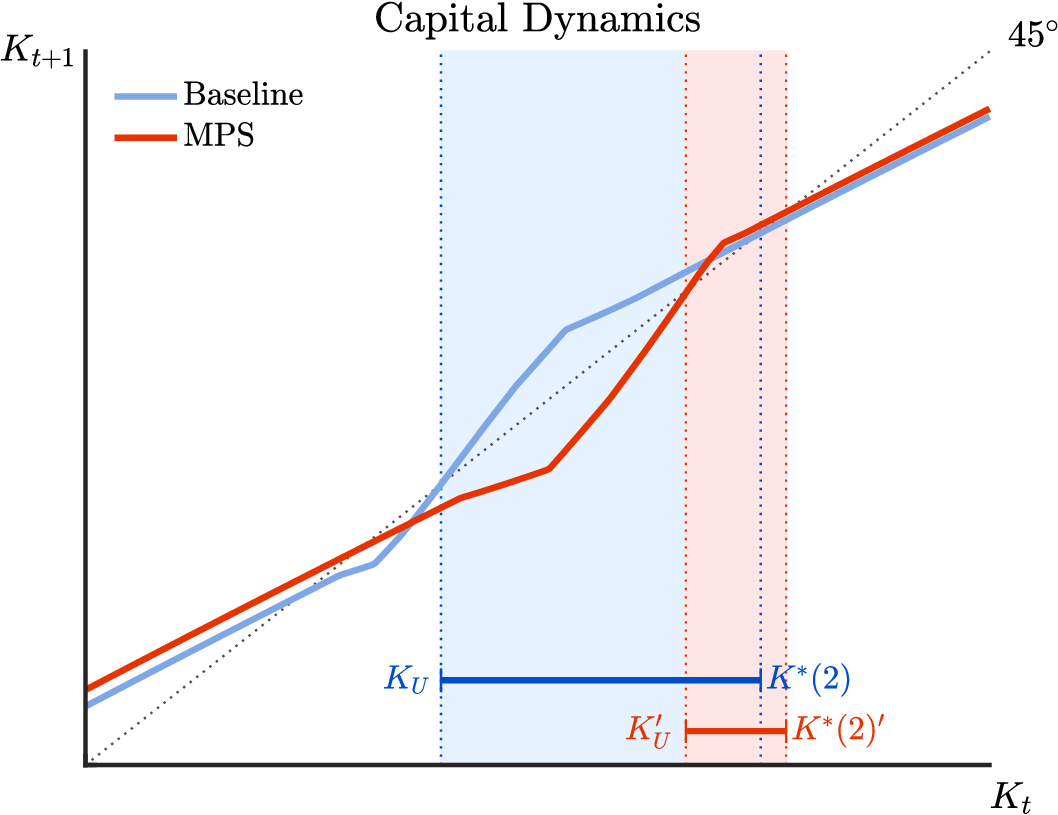}
 \hspace{0.4cm}
 \includegraphics*[scale=0.475]{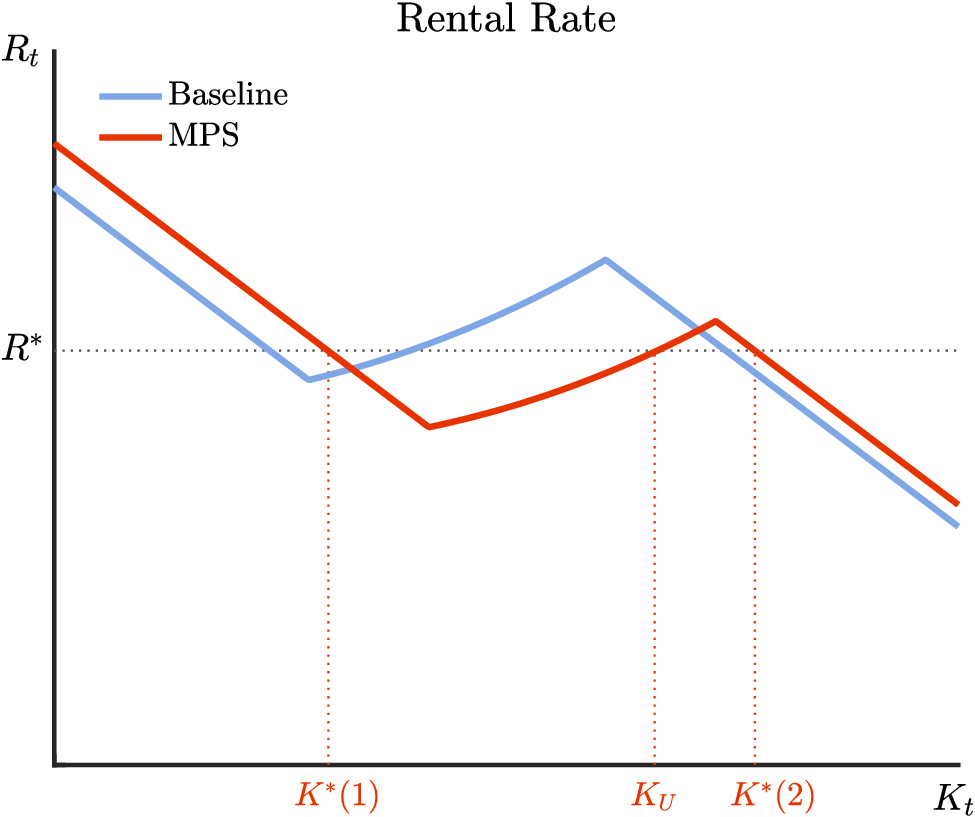}
\caption{Law of Motion and Rental Rate Map \label{fig:Law-of-Motion-MIS}
\protect \\ {This example features two stable steady states and an unstable one. We use $\psi \, = \, 1 \,$,  $\rho \, = \, 3/4 \,$, $\eta \, = \, 1 \,$, $\alpha \, = \, 1/3 \,$, $\delta \, = \, 1 \,$, $\nu \, = \, 2/5 \,$ and $ c_{i} \, = \, 0.015 \,$.}} 
\end{figure}

\subsection*{Steady-State Multiplicity}
\begin{figure}[H]
\centering{}
\hspace{-0.2cm}
 \includegraphics*[scale=0.475]{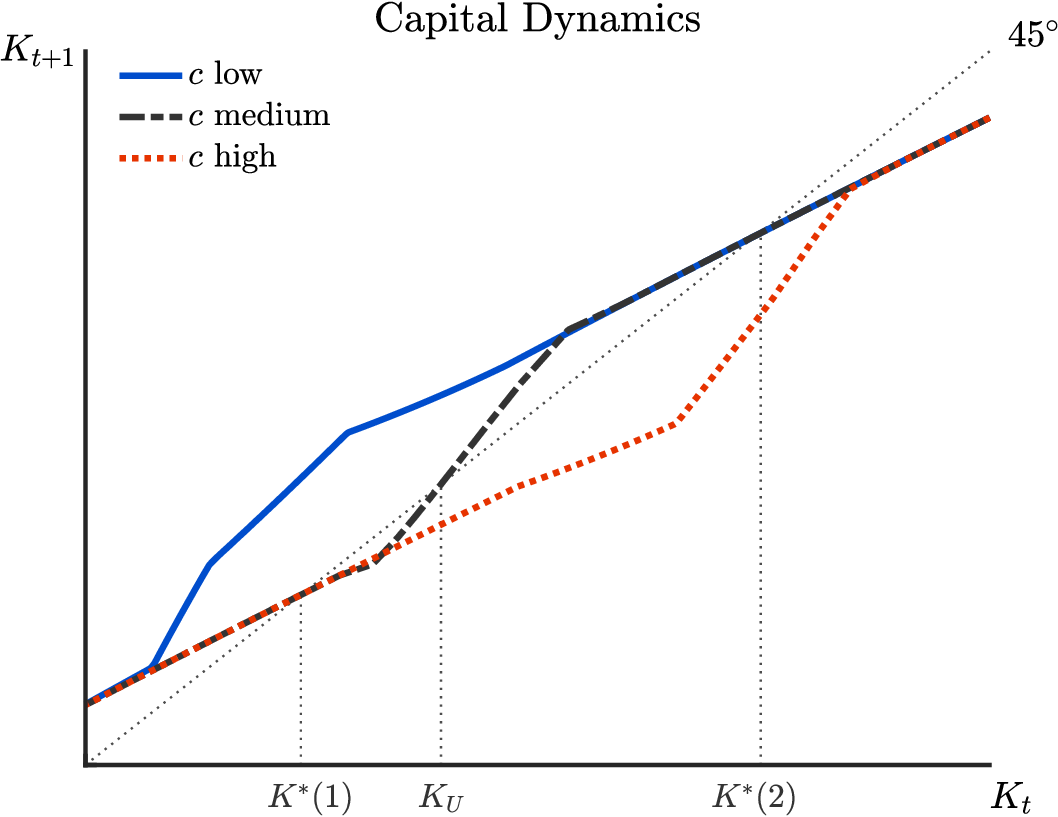}
 \hspace{0.4cm}
 \includegraphics*[scale=0.475]{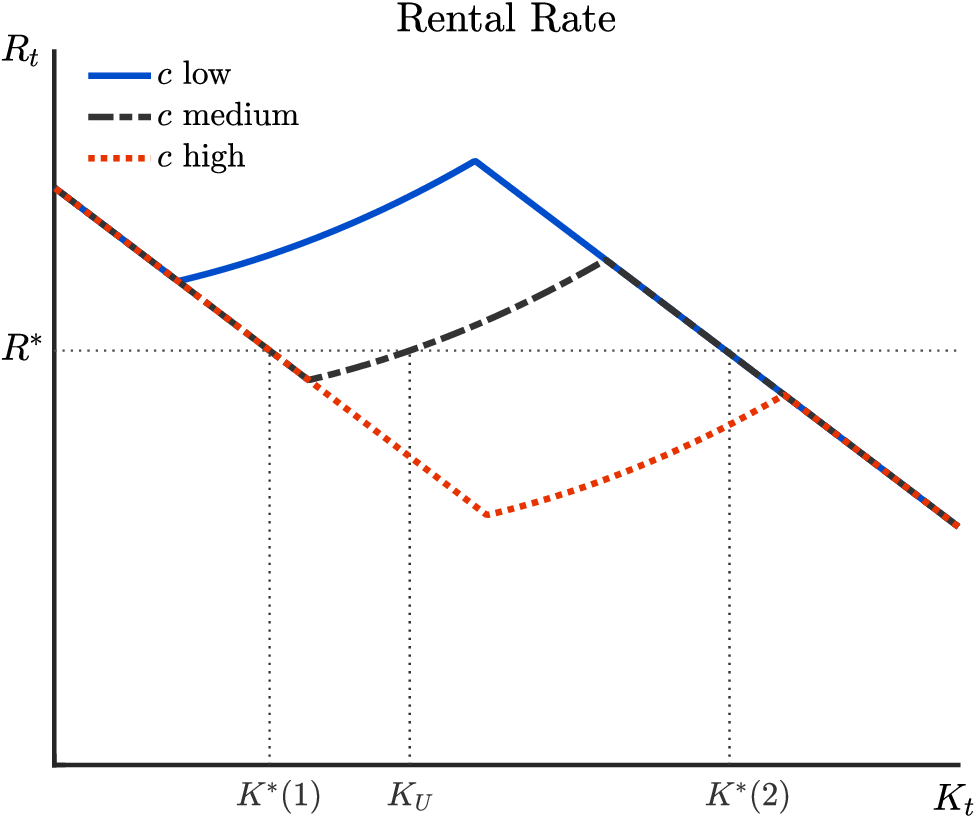}
\caption{Law of Motion and Rental Rate Map \label{fig:Law-of-Motion-existence}
\protect \\ {This example features two stable steady states and an unstable one. We use $\psi \, = \, 1 \,$,  $\rho \, = \, 3/4 \,$, $\eta \, = \, 1 \,$, $\alpha \, = \, 1/3 \,$, $\delta \, = \, 1 \,$ and $\nu \, = \, 2/5 $.}} 
\end{figure}

\section{The Quantitative Model \label{sec:Quantitative-Model}}

\subsection{Calibration \label{subsec:Calibration} }

\paragraph{Steady-State}

We perform three different calibrations of our model \textendash{} to match the average level of markups and its dispersion in 1975, 1990 and in 2007. We need to calibrate five technology parameters: the elasticity of substitution $\sigma_{I}$ and $\sigma_{G}$ (which are time-invariant), the log-normal standard deviation $\lambda$, the fixed production cost $c$ and the fraction of industries with zero fixed cost $f_{comp}$ (which are allowed to vary over time).

We start by specifying a grid with possible values for $\sigma_{I}$ and $\sigma_{G}$. Then, for each pair $\left(\sigma_{I} , \sigma_{G}\right)$, we specify a triplet $\left(\lambda, c, f_{comp} \right)$, as well as a grid with values for the aggregate capital stock $K$. We then compute the aggregate equilibrium for each parameter combination $\left(\sigma_{I}, \sigma_{G}, \lambda, c, f_{comp} \right)$
and for each value $K$.\footnote{Aggregate TFP $e^{z_{t}}$ is assumed to be constant and equal to one.} We start by assuming that all firms are active, so that there are $N$ firms in each of the $I$ industries. We compute the aggregate equilibrium using equations (\ref{eq:agg_tfp}) and (\ref{eq:agg_cost}). We then compute the profits net of the fixed cost that each firm makes
\[
\left(p_{ijt} - \dfrac{\Theta_{t}}{\tau_{ijt}} \right)\:y_{ijt} - c_{i}
\]
and identify the firm with the largest negative value. We exclude this firm and recompute the aggregate equilibrium. We repeat this iterative procedure until all firms have non-negative profits (net of the fixed production cost). If equilibrium multiplicity arises, this algorithm allows us to consistently select the equilibrium that features the largest number of  firms.

For each triplet $\left(\lambda, c, f_{comp} \right)$, we then have the general equilibrium computed for all possible capital values. The steady-state(s) of our economy correspond to the value(s) of $K$ for with the rental rate $R_{t}$ is equal to $\dfrac{1}{\beta}-\left(1-\delta\right)$. 

When multiple steady-states arise (as in the 1990 and 2007 economies), we compute model moments in the highest steady-state.

\paragraph{Data Definitions}

For the sales weighted-average markup, we use the series computed by \cite{LEU}. 
The authors calculate price-cost markups for the universe of public firms, using data from COMPUSTAT. The markup of a firm $j$ in a 2-digit NAICS sector $s$ at time $t$ is calculated as
\[
\mu_{sjt} = \xi_{st} \cdot \dfrac{\textrm{sale}_{sjt}}{\textrm{cogs}_{sjt}}
\]
where $ \xi_{st}$ is the elasticity of sales to the total variable input bundle, $\textrm{sale}_{sjt}$ is sales and $\textrm{cogs}_{sjt}$ is the cost of the goods sold, which measures total variable costs.

% To measure markup dispersion, we compute the standard deviation of markups within 2-digit NAICS sectors. Treating $ \xi_{st}$ as constant within a sector $s$ and time $t$, we can measure markup dispersion within this sector as

% \[
% \textrm{sd}_{s}\left[\textrm{log}\left(\mu_{sjt}\right)\right] = \textrm{sd}_{s}\left[\textrm{log}\left(\dfrac{\textrm{sale}_{sjt}}{\textrm{cogs}_{sjt}}\right)\right]
% \]

% We calculate this measure for all 23 sectors (2-digit NAICS). We then compute an average across all such sectors, weighted by the sector sales. Figure \ref{fig:Markup-Dispersion} shows the evolution of this measure.

% In our model, we compute the standard deviation of (log) markups across all firms in the economy, i.e. we do not compute it industry by industry. We think of an industry in our model as a market at the possible level of disaggregation (e.g. 10-digit NAICS). We cannot however observe data at such a fine level of disaggregation \textendash{} first because most data sets only provide industry information at the 6-digit, second because many large firms are multi-product an operate in different markets. We hence think of our final good $Y_t$ as one big-sector.

% \begin{figure}[H]
% \centering{}%
% \includegraphics*[scale=0.6]{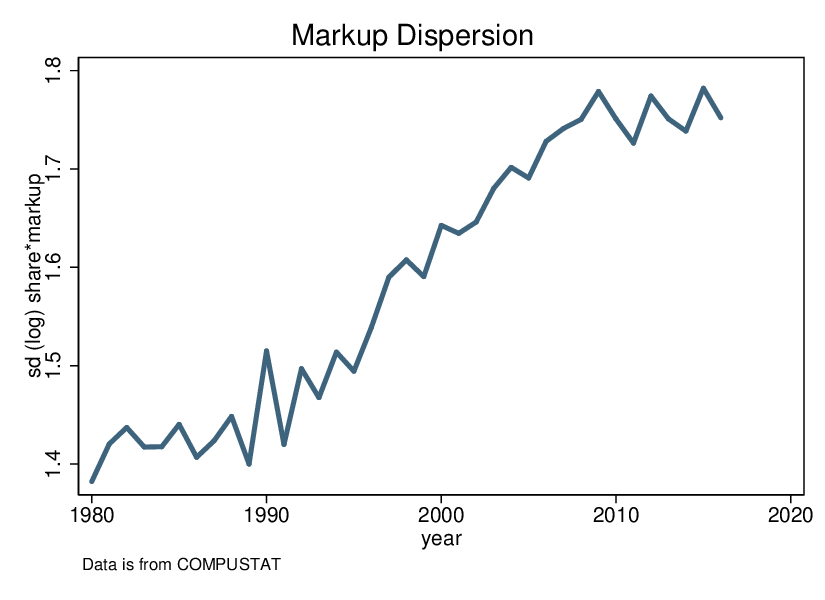}\tabularnewline
% \caption{Markup Dispersion\protect \\ {Note: \small{} the figure shows the evolution of markup dispersion computed from COMPUSTAT data for 2-digit industries.}
% \label{fig:Markup-Dispersion}}
% \end{figure}

\subsection{Solution Algorithm for the Dynamic Optimization Problem}

We now explain the algorithm we use for the dynamic optimization problem of the representative household. We take the calibrated parameters $\left(\lambda, c \right)$ and form a grid for aggregate capital with $n_K = 70 $ points. This grid is centered around the highest steady-state $K^{\text{ss}}_H$, with a lower-bound $0.5 \times K^{\text{ss}}_H$ and upper bound $1.5 \times K^{\text{ss}}_H$. We also form a grid for aggregate TFP, $A$. We use Tauchen's algorithm with $n_A = 11$ points, autocorrelation parameter $\phi_A$ and standard deviation for the innovations $\sigma_{\varepsilon}$ (the last two parameters are calibrated, as explained in the main text). We compute the aggregate equilibrium for each value of $K$ and $A$. 

We next compute a numerical approximation for the household policy function, by iterating on the Euler equation. We start by making a guess for the savings rate
\[
s\left(X_t\right) \coloneqq \dfrac{C\left(X_t\right) }{Y\left(X_t\right) }
\]
for every combination of the vector of state-variables $X_t \coloneqq \left(K_t, A_t\right)$. Given a guess $s^{\left(n\right)}\left(X_{t}\right) \; \forall X_t$ for the savings rate, we use the Euler equation to obtain a new guess $s^{\left(n+1\right)}\left(X_{t}\right)$ as follows
\begin{comment}
\[
\dfrac{1}{C_{t}-\dfrac{L_{t}^{1+\nu}}{1+\nu}}=\mathbb{E}_{t}\left\{ \dfrac{\beta\left[R_{t+1}+\left(1-\delta\right)\right]}{C_{t+1}-\dfrac{L_{t+1}^{1+\nu}}{1+\nu}}\right\} 
\]
\end{comment}

{\footnotesize
\[
\begin{array}{rl}
 & \dfrac{1}{\left(1-s^{\left(n+1\right)}\left(X_{t}\right)\right)Y\left(X_{t}\right)-\dfrac{W\left(X_{t}\right)^{\left(1+\nu\right)/\nu}}{1+\nu}}=\mathbb{E}_{t}\left\{ \dfrac{\beta\left[R\left(X_{t+1}\right)+\left(1-\delta\right)\right]}{\left(1-s^{\left(n\right)}\left(X_{t+1}\right)\right)Y\left(X_{t+1}\right)-\dfrac{W\left(X_{t+1}\right)^{\left(1+\nu\right)/\nu}}{1+\nu}}\right\} \\[8ex]
\Leftrightarrow & s^{\left(n+1\right)}\left(X_{t}\right)=1-\dfrac{1}{Y\left(X_{t}\right)}\left\{ \dfrac{W\left(X_{t}\right)^{\left(1+\nu\right)/\nu}}{1+\nu}+\left[\mathbb{E}_{t}\left\{ \dfrac{\beta\left[R\left(X_{t+1}\right)+\left(1-\delta\right)\right]}{\left(1-s^{\left(n\right)}\left(X_{t+1}\right)\right)Y\left(X_{t+1}\right)-\dfrac{W\left(X_{t+1}\right)^{\left(1+\nu\right)/\nu}}{1+\nu}}\right\} \right]^{-1}\right\}.
\end{array}
\]
}
We iterate on this procedure until

\[
\left|s^{\left(n+1\right)}\left(X_{t}\right)- s^{\left(n\right)}\left(X_{t}\right) \right| \; < \;  \epsilon \quad \forall X_t .
\]

\subsection{Business Cycle Moments \label{subsec:business_cycle_moments}}

\begin{table}[H]
\setlength{\tabcolsep}{0.4cm}  
\begin{center}
\begin{tabular}{lccccc} 		\thickhline
\\[-2ex]
& Output & Consumption & Investment & Hours & TFP \\ \thickhline
\\[-2ex]
& \multicolumn{4}{c}{Correlation with Output} \\
\\[-2ex]
Data: 1947-2019 & 1.00 & 0.95 & 0.76 & 0.67 & 0.71 \\[0.25ex]
Model: 1975 calibration & 1.00 & 0.99 & 0.92 & 1.00 & 0.83 \\[0.25ex]
Model: 1990 calibration & 1.00 & 1.00 & 0.96 & 1.00 & 0.88 \\[0.25ex]
Model: 2007 calibration & 1.00 & 1.00 & 0.96 & 1.00 & 0.89  \\ 
\\
& \multicolumn{4}{c}{Standard Deviation Relative to Output} \\
\\[-2ex]
Data: 1947-2019 & 1.00 & 0.90 & 2.04 & 0.98 & 0.95 \\[0.25ex]
Model: 1975 calibration & 1.00 & 0.95 & 1.54 & 0.74 & 0.25 \\[0.25ex]
Model: 1990 calibration & 1.00 & 0.97 & 1.23 & 0.78 & 0.17 \\[0.25ex]
Model: 2007 calibration & 1.00 & 0.98 & 1.20 & 0.79 & 0.15  \\ 
\\[-2ex]\thickhline
\end{tabular} \end{center}
\caption{Business Cycle Moments. All variables are in logs. Data variables are in per capita terms (except TFP) and in deviation from a linear trend computed over 1947-2007.} \label{tab:business_cycle_moments}
\end{table}

Table \ref{tab:business_cycle_moments} shows some business cycle moments for our two calibrated economies, as well as their data counterparts.
To be consistent with our interpretation that the US economy transitioned to a lower steady-state after 2008, all data variables are in deviation from a linear trend computed over 1947-2007. This fact explains the large empirical correlation between consumption and output. 
Comparing our two calibrated economies, we see that both economies display the same correlations of consumption and hours with output. The 2007 economy displays, however, a significantly lower correlation of investment with output. %This is explained by the fact the investment appears to be more volatile in the 2007 economy.

\subsection{Aggregate Productivity \label{subsec:agg_TFP}}

\subsubsection*{Average Firm Level TFP}

\begin{figure}[H]
\centering
\includegraphics*[scale=0.8]{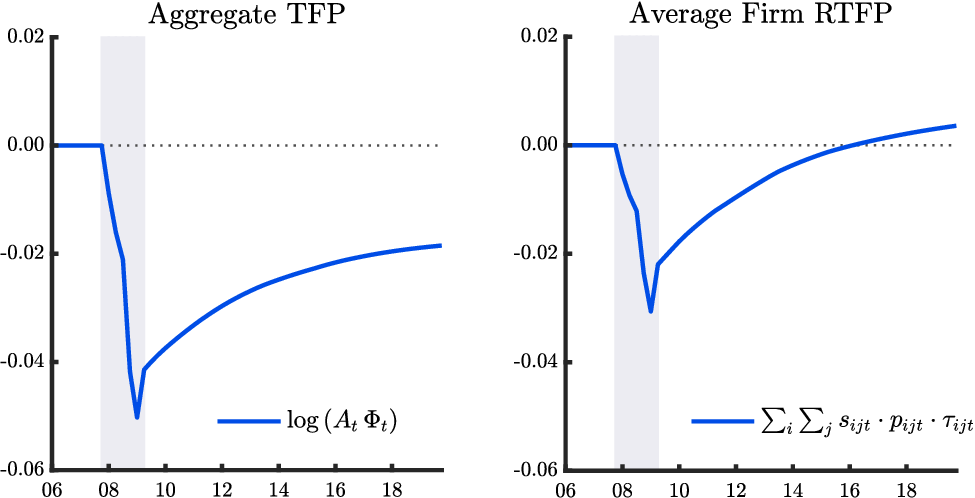}\caption{Aggregate TFP versus Average Firm Level TFP \protect \\
{Note: \small{}The left panel shows aggregate TFP. The right panel shows a sales-weighted average of firm level revenue TFP $p_{ijt}\cdot\tau_{ijt}$.
\label{fig:TFP_Model_transition}}}
\end{figure}

Figure \ref{fig:TFP_Model_transition} reports a sales-weighted average of firm level revenue TFP. A similar pattern emerges if one uses physical TFP instead.

\subsubsection*{Dispersion in Industry Output}

\begin{figure}[H]
\centering
\includegraphics*[scale=0.5]{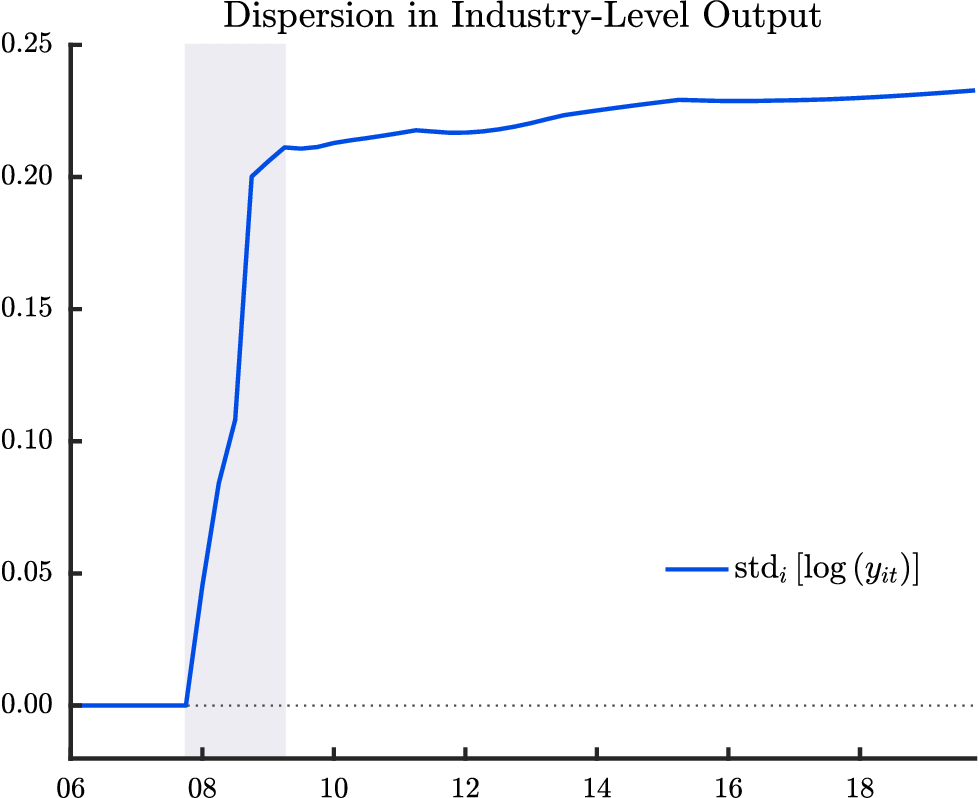}\caption{Dispersion in $\log\left(y_{it}\right)${\small{} \label{fig:output_dispersion_transition}}}
\end{figure}

%\subsection{The Great Recession}
% \subsection{Welfare \label{subsec:welfare_GR}}
% \begin{figure}[H]
% \centering
% \includegraphics*[scale=0.7]{input/GR_welfare_model}\caption{The great recession and its aftermath: welfare \label{fig:GR_welfare_model}}
% \end{figure}

\section{The 1990 Recession \label{sec:90_recession}}

\subsubsection*{The response in the 1990 economy}

\begin{figure}[H]
\begin{minipage}[b]{.5\linewidth}
\centering{}\includegraphics*[scale=0.5]{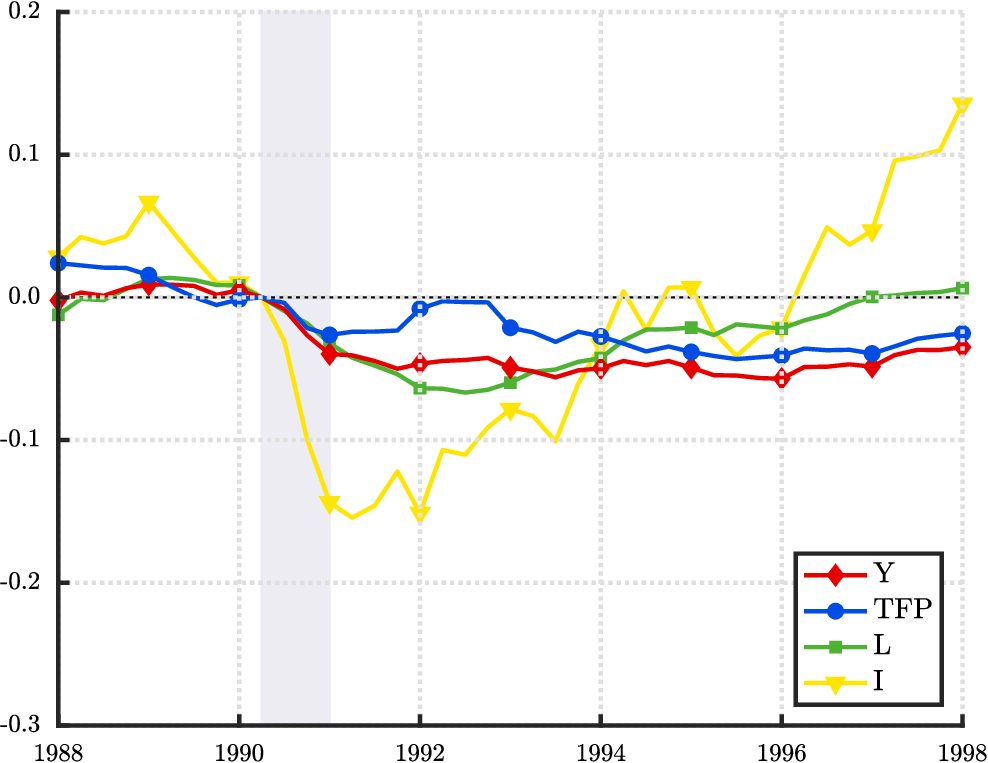}\subcaption{1990-1991 recession (data) \label{fig:data_90_recession}}
\end{minipage}
\begin{minipage}[b]{.5\linewidth}
\centering{}\includegraphics*[scale=0.5]{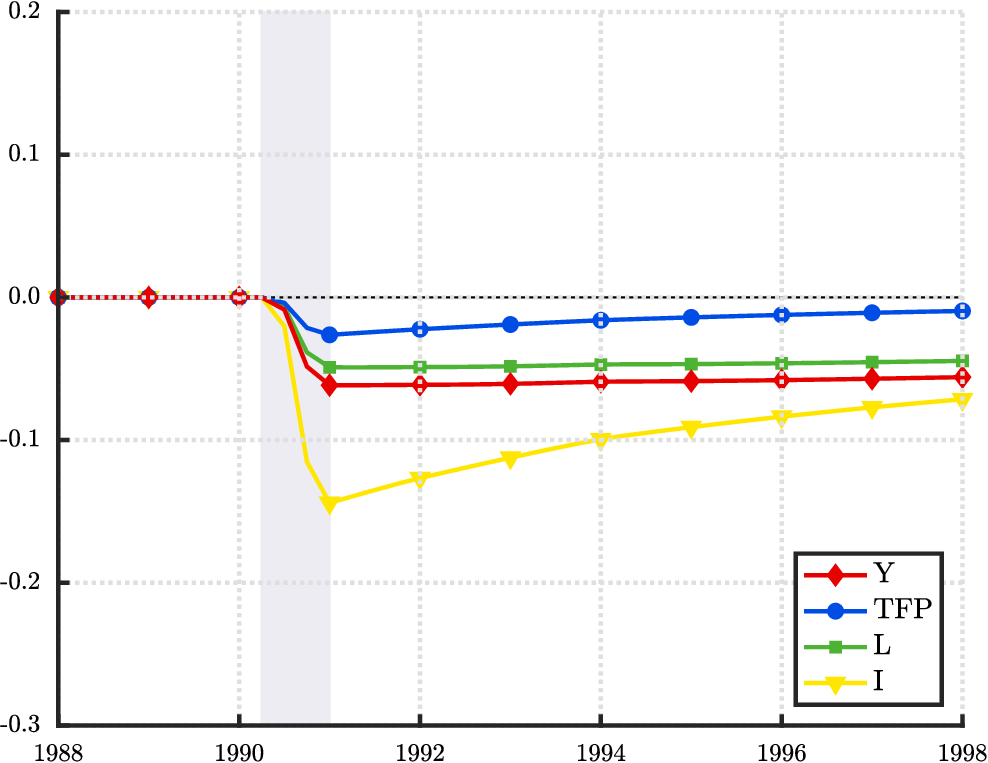}\subcaption{The 1990-1991 shock in the 1990 model \label{fig:85_model_82_crisis}}
\end{minipage}
\caption{The 1990-1991 recession \label{fig:90_crisis}}
\end{figure}

\subsubsection*{The response in the 2007 economy}

\begin{figure}[H]
\centering{}\includegraphics*[scale=0.65]{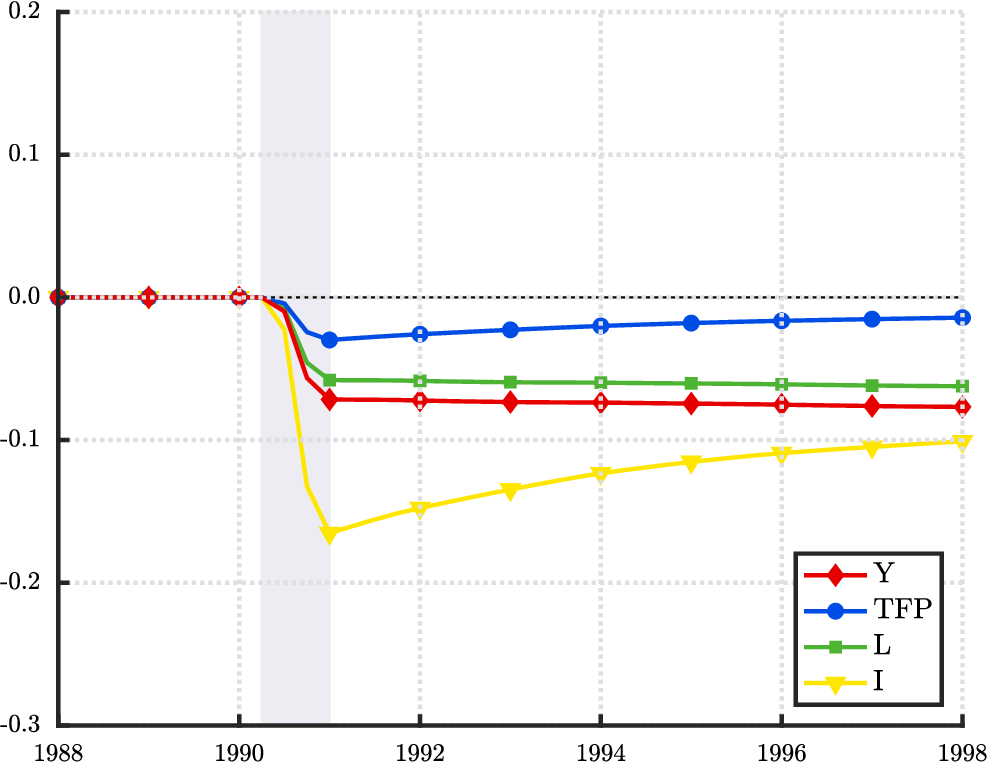}
\caption{The 1990-1991 shock in the 2007 model
\label{fig:07_model_90_crisis}}
\end{figure}

\section{Number of Firms per Sector}
\label{sec:numberfirms}
\begin{figure}[H]
\begin{centering}
\includegraphics*[scale=0.9]{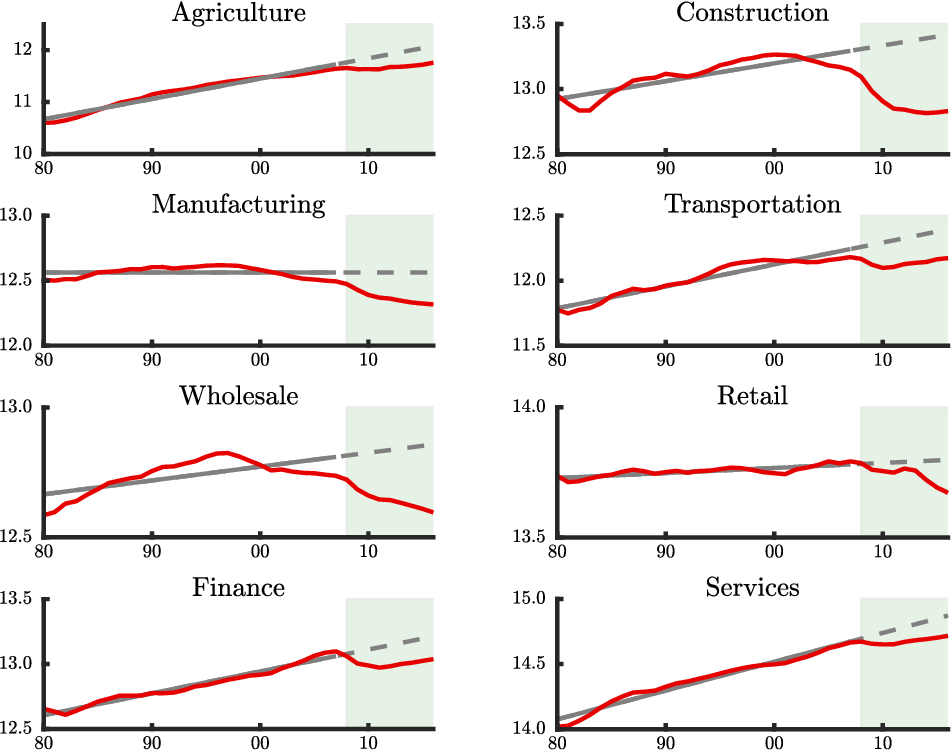} 
\par\end{centering}
\caption{\textbf{Number of Firms per Sector: 1980-2018}\protect \\
{\small{}Each panel shows the number of firms with at least one employee in each sector (in logs). For
each series, the dashed grey line shows a linear trend computed over the 1980-2007 period. Data is from the US Business Dynamics Statistics\label{fig:nfirms_sector}}}
\end{figure}

% \section{Size Dispersion} \label{sec:std_log_ms}
% \begin{figure}[H]
% \centering{}%
% \includegraphics*[scale=0.7]{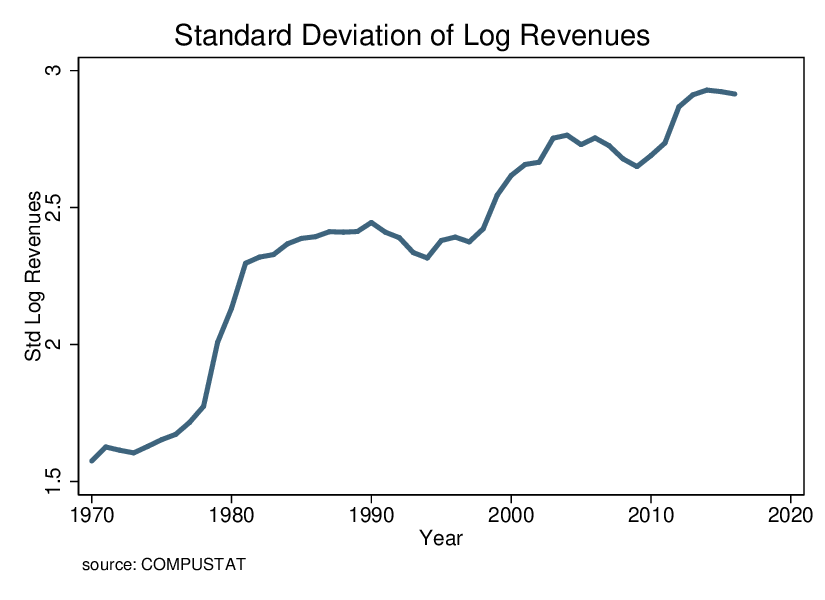}\tabularnewline
% \caption{Standard Deviation of Log Revenues \\ This figure shows the standard deviation of log revenues (COMPUSTAT item SALE), computed on a yearly basis, for all firms in COMPUSTAT.
% \label{fig:std_log_ms}}
% \end{figure}

\section{Fixed Costs}\label{sec:fixed_costs_data}
\begin{figure}[H]
\centering{}%
\includegraphics*[scale=0.7]{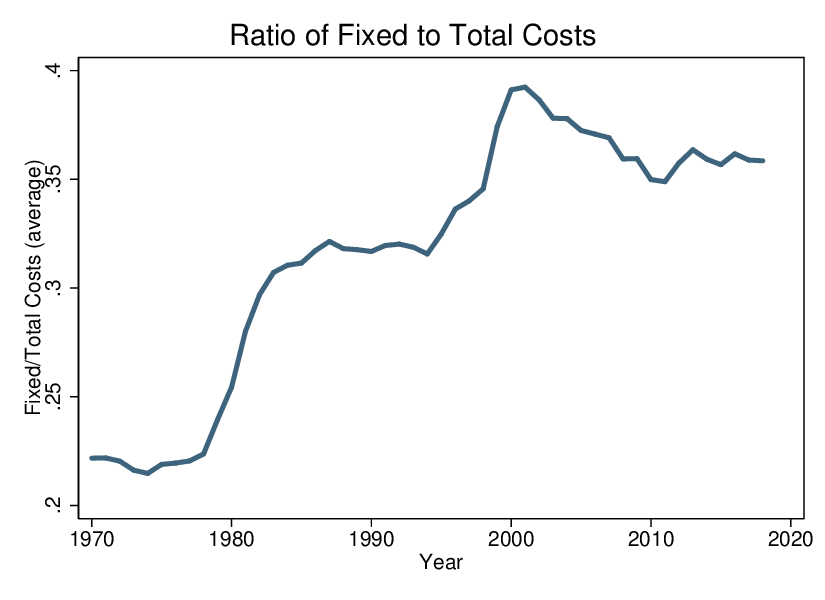}\tabularnewline
\caption{Ratio of fixed to total costs \\ This figure shows the average ratio of fixed to total costs for COMPUSTAT firms. Following \cite{GW}, we define fixed costs as the sum of `Selling, General and Administrative Expenses' (COMPUSTAT item XSGA), `Advertising Expenses'
(Compustat item XAD) and `R\&D Expenditures'  (Compustat item XRD). Total costs are the sum of fixed costs and variable costs, where the latter correspond to the `Cost of Goods Sold' (Compustat item COGS).
\label{fig:fixed_total_costs}}
\end{figure}

\section{Robustness: Variable Fixed Costs} \label{sec:var_fixed_costs}

We assume that, each period, a fixed amount $c_f$ of firms' output is lost
\begin{align*}
    c_f=k_c^\alpha l_c^{1-\alpha}
\end{align*}

Given these assumptions, firms need to pay a per per period fixed cost
\[
\Theta_{t} \cdot c_f
\]
where $\Theta_{t} $ is the factor price index.

Denoting by $L_{yt}$ and $K_{yt}$ the aggregate stocks of labor and capital used in the production, we have the following market clearing conditions for labor and capital
\begin{align*}
    L_{t} = L_{yt} + N^{c}_{t} \cdot l_c \\
    K_{t} = K_{yt} + N^{c}_{t} \cdot k_c
\end{align*}
where $N^{c}$ denotes the number of firms incurring $c_f$. Note that the optimal mix of $l_c$ and $k_c$ chosen by each individual firm satisfies
\begin{align*}
    \dfrac{k_c}{l_c} = \dfrac{K_{yt}}{L_{yt}}
\end{align*}

\subsubsection*{Calibration}
Parameters not reported are as in the baseline calibration (Table \ref{tab:parameter_values}).
\begin{table}[ht!]
\setlength{\tabcolsep}{0.2cm} \begin{center} \resizebox{16cm}{3.7cm} {  \begin{tabular}{lccccl}
\thickhline
\\[-1ex]
{\large Description} & {\large Parameter} & \multicolumn{3}{c}{{\large Value}} & {\large Source/Target} \\[1ex] \thickhline
\\[-1ex]
[A.1] Calibrated Parameters: Fixed \\ \\[-1ex]
\hline
\\[-1ex]
Between-industry ES & $\sigma_{I}$ & \multicolumn{3}{c}{1.33} & Sales-weighted average markup\\
\\[-1ex]
Within-industry ES & $\sigma_{G}$ & \multicolumn{3}{c}{12.5} & Sales-weighted average markup \\
\\[-1ex]
Persistence of $z_t$  & $\rho_{z}$ & \multicolumn{3}{c}{0.950} & Autocorrelation of log $Y_t$ \\
\\[-1ex]
Standard deviation of $\varepsilon_t$ & $\sigma_{\varepsilon}$ & \multicolumn{3}{c}{0.003} & Standard deviation of log $Y_t$ \\ 
\\[-1ex] \hline
\\[-1ex]
[A.2] Calibrated Parameters: Variable & & 1975 & 1990 & 2007 & \\ \\[-1ex] \hline
\\[-1ex]
Fraction of industries with $c_{i}>0$ & $f$ & 0.105 & 0.140 & 0.130 &  Emp share concentrated industries \\
\\[-1ex]
Standard deviation of $\gamma_{ij}$ & $\lambda$ & 0.193 & 0.252 & 0.304 & Std log market share \\
\\[-1ex]
Fixed cost ($\times 10^{-4}$) & $c$ & 3.03 & 5.66 & 7.82 & Average ratio fixed/total costs \\
\\[-1ex]
\thickhline
\end{tabular}  
} \end{center}
\caption{Parameter Values\label{tab:parameter_values_vfc}}
\end{table}

\begin{table}[ht]
\setlength{\tabcolsep}{0.25cm}  
\begin{center}
\resizebox{16cm}{3.7cm} {
\begin{tabular}{lcccccccc} 		\thickhline 
\\[-2ex]
& \multicolumn{2}{c}{1975} & & \multicolumn{2}{c}{1990} & & \multicolumn{2}{c}{2007} \\
\\[-1ex] 
& Data & Model & & Data & Model & & Data & Model \\ \hline  
\\[-1ex] 
Sales-weighted average markup & 1.28 & 1.26 & & 1.37 & 1.38 & & 1.46 & 1.44 \\
\\[-1ex]
Std log revenues & 1.67 & 1.74 & & 2.47 & 2.36 & & 2.79 & 2.92 \\
\\[-1ex]
Average fixed to total cost ratio & 0.244 & 0.259 & & 0.355 & 0.390 & & 0.414 & 0.420 \\
\\[-1ex]
Emp share \textit{concentrated} industries & - & 0.067 & & - & 0.072 & & 0.063 & 0.060 \\
\\[-1ex] \hline 
\\[-1ex]
Autocorrelation log GDP  &  &  & &  &  & & 0.978* & 0.976 \\
\\[-1ex]
Standard deviation log GDP &  &  & &  &  & & 0.061* & 0.056 \\
\\[-1ex]
\thickhline
\\[-1ex]
\multicolumn{6}{l}{*computed over 1947:Q1-2019:Q4} \\
\end{tabular}} \end{center}
\caption{Targeted moments and model counterparts\label{tab:targeted_moments_vfc}}
\end{table}

\subsubsection*{Ergodic Distributions}

\begin{figure}[H]
\hspace{-1cm}
\begin{minipage}[b]{.33\linewidth}
\centering\includegraphics*[scale=0.325]{input/hist_1975_vfc.eps}\subcaption{1975} \label{fig:y_dist_1975_vfc}
\end{minipage}%
\begin{minipage}[b]{.33\linewidth}
\centering\includegraphics*[scale=0.325]{input/hist_1990_vfc.eps}\subcaption{1990} \label{fig:y_dist_1990_vfc}
\end{minipage}
\begin{minipage}[b]{.33\linewidth}
\centering\includegraphics*[scale=0.325]{input/hist_2007_vfc.eps}\subcaption{2007} \label{fig:y_dist_2007_vfc}
\end{minipage}
\caption{Ergodic distribution of output \protect \\ {Note: \small{}\small{} This figure shows the distribution of log output for the 1975, 1990 and the 2007 economies. We simulate each economy for 10,000,000 periods and plot output in deviation from the high steady state.}} \label{fig:businesscycle_vfc}
\end{figure}

\subsubsection*{The 2008 Crisis}

\begin{figure}[H]
\begin{minipage}[b]{.33\linewidth}
\centering{}\includegraphics*[scale=0.325]{input/GR_transition_1975_vfc.eps}\subcaption{1975 Model \label{fig:GR_1975_vfc}}
\end{minipage}%
\begin{minipage}[b]{.33\linewidth}
\centering{}\includegraphics*[scale=0.325]{input/GR_transition_1990_vfc.eps}\subcaption{1990 Model \label{fig:GR_1990_vfc}}
\end{minipage}
\begin{minipage}[b]{.33\linewidth}
\centering{}\includegraphics*[scale=0.325]{input/GR_transition_2007_vfc.eps}\subcaption{2007 Model \label{fig:GR_2007_vfc}}
\end{minipage}
\caption{The \textit{great recession} in the 1975, 1990 and 2007 models \protect \\ {Note: \small{}The 2007 model is subjected to a sequence of six quarter shocks $\left\{\varepsilon_{t}\right\}$ to match the dynamics of aggregate TFP in the data between 2008Q1:2009Q2. This sequence of shocks is then fed in the 1975 and 1990 economies.}}
\end{figure}
