# Supplementary material for: Firm Heterogeneity, Market Power and Macroeconomic Fragility
Source: arXiv:2205.03908 source file (2024-05-10)
Supplement: Supplementary file 2 [file appendix_A.tex]

\setcounter{figure}{0}
\setcounter{table}{0}
\setcounter{lemma}{0}
\setcounter{prop}{0}
\setcounter{cor}{0}

\begin{center}
    
{\Huge {Appendix A} }
\end{center}

\section{Data Appendix \label{sec:Data-Appendix}}

% \begin{figure}[ht!]
% \begin{minipage}[t]{.5\linewidth}
% \includegraphics*[scale=0.5]{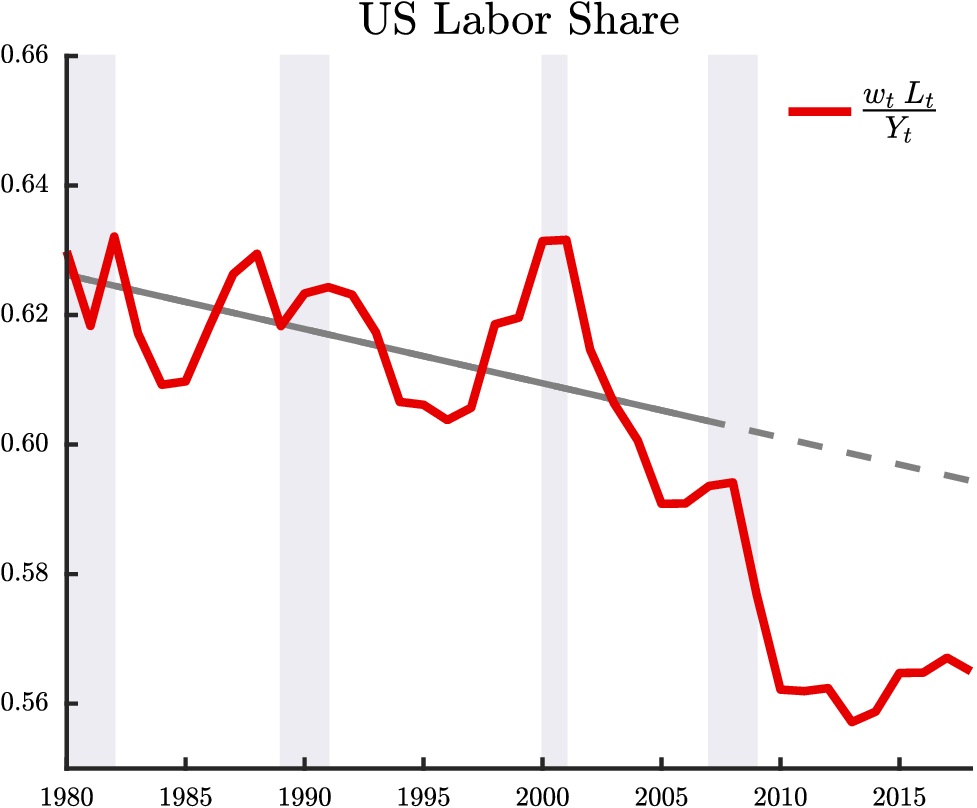}\subcaption{\textbf{Labor Share of the US Business Sector}} \label{fig:labor_share}
% \end{minipage}%
% \hspace{0.5cm}
% \begin{minipage}[t]{.5\linewidth}
% \includegraphics*[scale=0.5]{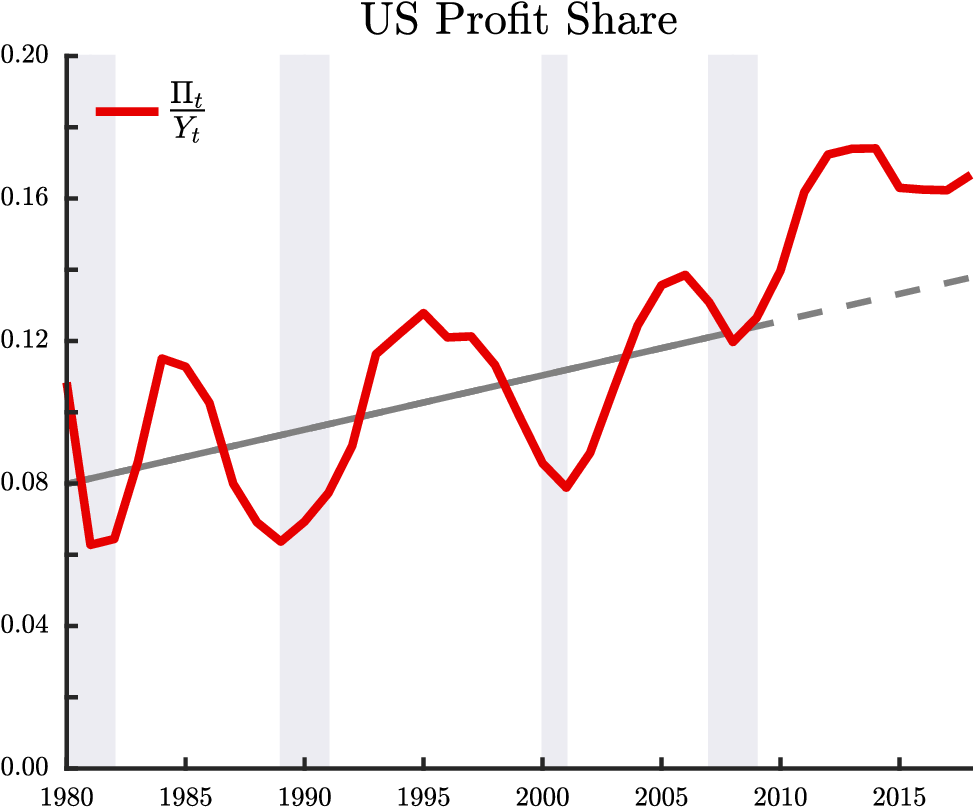}\subcaption{\textbf{Profit Share of the US Business Sector}} \label{fig:profit_share}
% \end{minipage}
% \caption{Labor and Profit Shares of the US Business Sector (1980-2018) \protect \\  {Note: \small{} The left panel shows the evolution of the labor share (see Appendix \ref{sec:alternative-labor-share} for alternative definitions of the labor share). The right panel shows a 3-year moving average the aggregate profit share, constructed as the ratio of aggregate profits to gross value added (see Appendix \ref{subsec:Agg-Profit-Share} for details). The linear trends are computed for the pre-crisis period 1980-2007.}} 
% \label{fig:labor_profit_shares_figure}
% \end{figure}

\begin{figure}[ht!]
\centering{}\includegraphics*[scale=0.7]{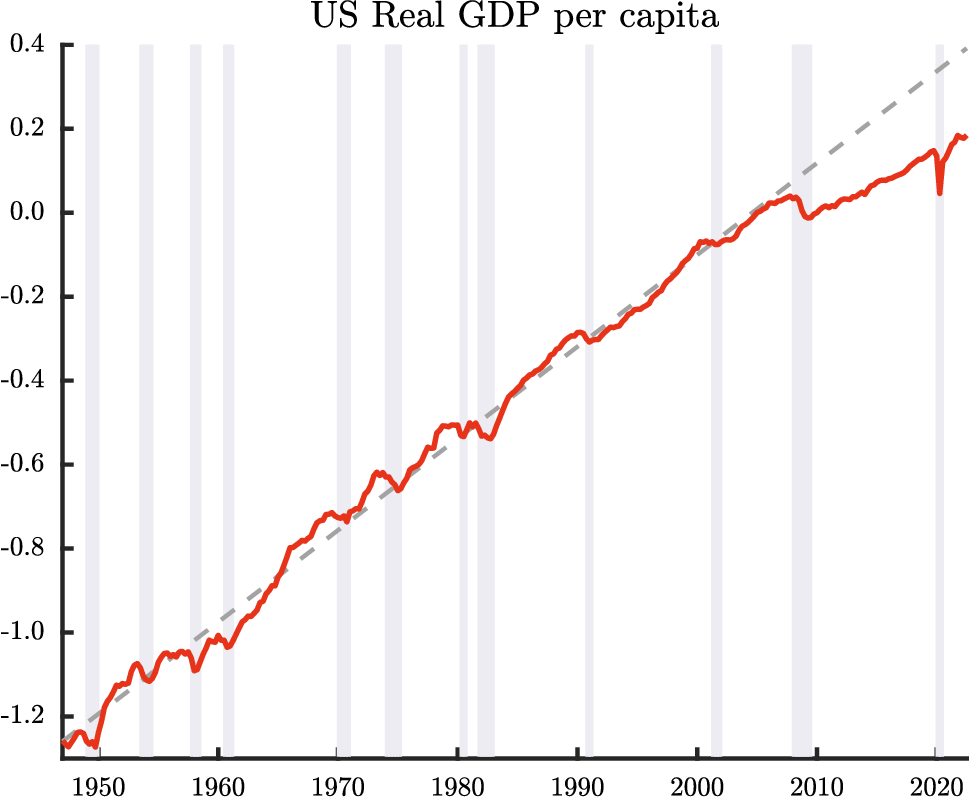}
\caption{The \textit{Great Deviation} \protect \\ {Note: \small{} This figure shows real GDP per capita (from BEA). The series is in logs, undetrended and centered around 2007. The linear trend is computed for the 1947-2007 period.}} 
\label{fig:great_deviation_figure}
\end{figure}

\paragraph{Data Definition}% \label{subsec:data-Definitions}}

Table \ref{tab:data_sources} provides information on all the data sources used in Section \ref{sec:aggregatefacts}.

\begin{table}[ht!]
\setlength{\tabcolsep}{0.25cm} \begin{center} \begin{tabular}{cc} \thickhline
\\[-2ex]
{\large Variable} & {\large Source} \\ [0.5ex] \thickhline
\\[-1ex]
Real GDP & BEA \textendash{} NIPA Table 1.1.3 (line 1)  \\[0.75ex]
Real Personal Consumption Expenditures & BEA \textendash{} NIPA Table 1.1.3 (line 2) \\[0.75ex]
Real Gross Private Domestic Investment & BEA \textendash{} NIPA Table 1.1.3 (line 7) \\[0.75ex]
Total Hours & BLS \textendash{} Nonfarm Business sector: Hours of all persons \\[0.75ex]
Aggregate TFP & \cite{F}: Raw Business Sector TFP \\[0.75ex]
Population & BEA \textendash{} NIPA Table 2.1 (line 40) \\ [1.5ex]
\thickhline
\end{tabular}  
\end{center}
\caption{Data sources}
\label{tab:data_sources}
\end{table}

\paragraph{Aggregate Profit Share }%\label{subsec:Agg-Profit-Share}}

The aggregate profit share is computed as
\[
\text{profit share}_{t} \; = \; 1 \; - \; \text{labor share}_{t} \; - \; \underbrace{\dfrac{ R_{t}\cdot\textrm{K}_{t} \: - \: \textrm{DEP}_{t}}{\textrm{VA}_{t}}}_{\text{capital share}}
\]
where $\text{labor share}_{t}$ is the labor share of the US business sector (from BLS),
$\textrm{VA}_{t}$ is the total value added of the US business sector (NIPA Table 1.3.5, line 2). $\textrm{K}_{t}$ is the value of private fixed assets (including intangibles) of the US business sector (NIPA Table 6.1, line 1 - line 9 - line 10) and $\textrm{DEP}_{t}$ is depreciation (NIPA Table 6.4, line 1 - line 9 - line 10). Finally, $\textrm{R}_{t}$ is the required rate of return. We follow \cite{ERW} and compute it as the difference between Moody's Seasoned BAA Corporate Bond Yield and a 5-year moving average of past CPI inflation (from BLS, used as a proxy for expected inflation).

\paragraph{Industry-level Labor Share }%\label{subsec:ind_labor_share}}

We obtain data on the labor share at the industry level from the BLS `Labor Productivity and Costs' (LPC) database. We calculate the labor share as the ratio of `Labor compensation' to `Value of Production'. Note that this ratio gives the share of labor compensation in total revenues, and not in value added.\footnote{This ratio coincides with the `Labor cost share' provided by the BLS. This variable is, however, available just for a restricted number of industries.}

\section{General Framework}\label{appendix:generalframework}
In this section we provide a taxonomy of the possible mechanisms behind multiplicity in our economy. We then provide to prove an intermediate lemma used in Proposition \ref{propcompstatexrc} and conclude by specifying three Remarks to exemplify the effect of heterogeneity on the fragility of the economy.

We start by noting that a necessary condition for multiplicity of steady states is that $\exists K^{*}: R_K(K^{*})>0$. It follows that the necessary condition can be rewritten as \\$\exists K^{*}: \left(\partial / \partial K\right) \Omega(\Lambda,n(\Lambda, K^{*}))\Phi(\Lambda,n(\Lambda, K^{*}))  F_{K}(K^{*}, L(\Lambda, n, K^{*}) ) > 0$.
There are three main mechanisms underlying the possible locally increasing returns to capital. 

\paragraph{Average Firm TFP} In an economy with heterogeneous technologies and no love for variety, aggregate TFP can be written as a weighted average of firm-level productivities. The weights will depend on market shares. Average firm-level TFP can be increasing in $K$ if a larger capital favors a reallocation towards more productive types. 

\paragraph{Love for Variety} In models with product differentiation, aggregate TFP typically increases in the number of available varieties. This reflects the fact that utility/welfare are themselves increasing in the number of available goods (i.e. there is \textit{love for variety}).
Take for simplicity an economy where firms operate with the same level of productivity $\gamma_{ij}=\gamma$, but with possibly different fixed costs $c_{ij}$. Each firm produces a differentiated good. A larger capital stock $K$ can increase the incentives for the entry of new firms/goods, thereby making $\Phi$ (weakly) increasing in $K$. Examples of papers highlighting this channel as a source of multiple equilibria/steady-states include \cite{ST_unemp}.\footnote{Without relying on multiple equilibria or multiple steady-states, \cite{CJ2} and \cite{BGM} show that a combination of imperfect competition with endogenous entry can generate endogenous amplification and persistence of aggregate fluctuations.}

\paragraph{Market Power} In models featuring imperfect competition and variable markups, changes in the number of active players can have an impact on the distribution of income across factors of production and oligopoly rents. Take for example an economy where firms have identical fixed costs $c_{ij} = c$ but possibly different productivities $\pi_{ij}$. Assume further that firms enter sequentially in reverse order of productivity. If profit levels are increasing in the aggregate capital stock $k$ (for a given set of players), a larger capital stock will result in a larger number of firms and lower markups. Lower markups in turn translate in a higher factor share $\Omega$. This can establish a positive relationship between $\Omega$ and $k$. Examples of papers highlighting this channel as a source of multiple equilibria/steady-states include \cite{MP}, \cite{CCR}, \cite{GZ} and \cite{J}. 

%\paragraph{Endogenous Labor Supply} An elastic labor supply is another force that can counterbalance decreasing returns to capital. Note, however, that this channel alone is not enough to make $F_{K}(\cdot)$ increasing in $K$: if labor supply is infinitely elastic, $F_{L}(\cdot)$ and $F_{K}(\cdot)$ will be constant; but for finite elasticities, $F_{K}(\cdot)$ needs to be decreasing in $K$.\footnote{ Since $F\left(K,L\right)$ is homogeneous of degree one, its partial derivatives are homogeneous of degree zero. This implies that they are solely functions of the capital-labor ratio $K/L$: $F_{L}(K,L)$ increases in $K/L$, whereas $F_{K}(K,L)$ decreases in $K/L$. Therefore, $F_{K}(K,L)$ cannot increase when $F_{L}(K,L)$ increases (and vice-versa).
%It is however possible that both $F_{K}(K,L)$ and $F_{L}(K,L)$ are constant. This happens is labor supply is infinitely elastic and the economy exhibits constant $K/L$.}
%However, if some of the other channels described above (e.g. higher TFP or lower markups) is active and has a positive effect on the equilibrium wage, endogenous labor supply will provide an amplification mechanism to such channel. To sum up, an elastic labor supply provides an additional mechanism that can counterbalance decreasing returns, but is not enough to make $F_{K}(K,L)$ increasing in $K$. 

Let us consider some special cases. The first remark discusses a mean-preserving spread to the distribution of idiosyncratic productivities in an economy with a fixed set of producers (i.e. no adjustment along the extensive margin). More precisely, we consider special case of mean-preserving spread in the transformation is monotonically increasing away from the median in the set of active producers.\footnote{For example, we consider going from $\Pi$ to $\tilde{\Pi}_{\gamma,S_{\Pi}}=\left(1+\gamma\cdot S_{\Pi}\right)\circ\Pi$, with $\gamma>0$, $S_\Pi$ monotonically decreasing within a row and row-wise zero-sum, and $\circ$ denoting the Hadamard product.  For a similar approach see \cite{herrendorf2000ruling}.}
%\begin{align*}
%    \tilde{\Pi}_{\gamma,S_\Pi}=\left(1+\gamma\cdot S_\Pi\right)\circ\Pi
%\end{align*}
We then consider a marginal change in $\gamma$.

\begin{remark}[\textbf{Allocative efficiency}]\label{fixedfirms} 
In an economy with a fixed set of active producers, a technological shift $ d \lambda $ increases fragility if 
\begin{align}
    \Omega_{\lambda}(\Lambda,n)\Phi(\Lambda,n)+\Omega(\Lambda,n)\Phi_{\lambda}(\Lambda,n)<0 &\quad \text{for }  K=\{\mathcal{K}_{n},\mathcal{K}_{n+1}\}, \text{n even}.
\end{align}

\end{remark}
Suppose for example that we consider a mean-preserving spread to the distribution of idiosyncratic productivities. Assume further that markups and market shares are both positive functions of productivities. If market shares are an non-decreasing function of productivities, then the second term is non-negative. To see this note that a mean-preserving spread, fixing the market share distribution, implies that the average productivity increases. Additionally the positive relationship between productivities and market share implies a reallocation from low to high productivity firms, reinforcing the increase in aggregate productivity. Secondly, if markups are themselves non-decreasing in market shares, then the first term is always non-positive. This result comes from the reallocation effect. As large firms become larger, they compress output to extract higher rents. In doing so they compress the factor share. Therefore fragility increases if the anti-competitive effect (first term) dominates the efficiency gains (second term) from increasing the dispersion of firm-level productivity. Through the lens of the taxonomy the first term in Remark \ref{fixedfirms} represents the market power channel, while the second term is the average firm TFP channel.

We are also interested in exploring the consequences of an increase in fixed costs. To simplify the exposition, suppose that the economy only contains one industry type $\left(I=1\right)$, that all producers have identical productivity and there is no love for variety. In that case, aggregate productivity $\Phi$ is fixed and changes in the equilibrium rental rate will only happen through the aggregate factor share $\Omega$.

\begin{remark} [\textbf{Market power}] \label{fixedaggTFP}
Consider an economy with one industry type $\left(I=1\right)$, identical producers and no love for variety. This economy will feature constant aggregate TFP, which we normalize to $\Phi(\Lambda,n)=\Phi$. Furthermore, because firms are identical, larger fixed costs only affect the aggregate factor share through changes in the mass of active firms, i.e. $\Omega_{\lambda}(\Lambda,n)=0$.
Therefore, in this economy a larger fixed cost generates greater fragility if 
\begin{align}
    \Omega_{n}(\Lambda,n) n_{\lambda}\left(\Lambda,k\right)<0  &\quad \text{for }  k=\{\mathcal{K}_{n},\mathcal{K}_{n+1}\}, \text{n even}.
\end{align}
\end{remark}
First, note that the aggregate factor share should be non-decreasing in the aggregate mass of firms, i.e. $\Omega_{n}(\Lambda,n) \geq 0$. As firms exit due to the higher fixed cost the surviving firms increase their market shares. In doing so they are able to increase their markups and compress the factor share. Second, the aggregate mass of firms should must be non-increasing in fixed costs $n_{\lambda}(\Lambda,k) \leq 0$. This effect comes from firms being unable to cover the increased fixed costs and exiting. Therefore, larger fixed costs should generate increase fragility. 

We also consider an economy with a constant markups and factor shares, to highlight how changes in the mass of firms can affect aggregate TFP.

\begin{remark} [\textbf{Love for variety}]\label{loveforvariety}
Consider an economy with constant markups and aggregate factor share $\Omega(\Lambda,n)=\Omega$. A technological shift $ d \lambda $ increases fragility if 
\begin{align}
\Phi_{\lambda}(\Lambda,n)+\Phi_{n}(\Lambda,n)n_{\lambda}\left(\Lambda,k\right)<0 &\quad \text{for }  k=\{\mathcal{K}_{n},\mathcal{K}_{n+1}\}, \text{n even}.
\end{align}
\end{remark}
Suppose for example that we consider a mean-preserving spread to idiosyncratic productivities. In that case, if there is a reallocation towards more productive firms, we have $\Phi_{\lambda}(\Lambda,n) \geq 0$, as well as  $\Phi_{n}(\Lambda,n) \geq 0$ (love for variety) and $n_{\lambda}(\Lambda,n) \leq 0$ (if less productive firms are driven out of the market). If the second effect dominates (i.e. loss in number of varieties is stronger than the increase in average technical efficiency), fragility increases.

\section{The Quantitative Model \label{sec:Quantitative-Model}}

\subsection{Calibration \label{subsec:Calibration} }

\paragraph{Steady-State}

We perform two different calibrations of our model \textendash{} to match the average level of markups and its dispersion in 1985 and in 2007. We need to calibrate three technology parameters: the Pareto tail $\lambda$, the fixed production cost $c$ and the fraction of industries with zero fixed cost $f_{comp}$.

We specify a grid of possible candidates for $\lambda$, $c$ and $f_{comp}$. We also specify a grid with values for the aggregate capital stock $K$. We then compute the aggregate equilibrium for each parameter combination $\left(\lambda, c, f_{comp} \right)$
and for each value $K$.\footnote{Aggregate TFP $e^{z_{t}}$ is assumed to be constant and equal to one.} We start by assuming that all firms are active, so that there are $M$ firms in each of the $I$ industries. We compute the aggregate equilibrium using equations (\ref{eq:agg_tfp}) and (\ref{eq:agg_cost}). We then compute the profits net of the fixed cost that each firm makes
\[
\left(p_{ijt} - \dfrac{\Theta_{t}}{\tau_{ijt}} \right)\:y_{ijt} - c_{i}
\]
and identify the firm with the largest negative value. We exclude this firm and recompute the aggregate equilibrium. We repeat this iterative procedure until all firms have non-negative profits (net of the fixed production cost). For most parameter combinations, our model admits a unique equilibrium. However, if equilibrium multiplicity arises, this algorithm allows us to consistently select the equilibrium that features the largest number of  firms.

For each triplet $\left(\lambda, c, f_{comp} \right)$, we then have the general equilibrium computed for all possible capital values. The steady-state(s) of our economy correspond to the value(s) of $K$ for with the rental rate $R_{t}$ is equal to $\dfrac{1}{\beta}-\left(1-\delta\right)$. 

Given our interpretation that the US economy was in a competition regime in both 1985 and 2007, we compute model moments in the highest steady-state.

\paragraph{Data Definitions}

For the sales weighted-average markup, we use the series computed by \cite{LEU}. 
The authors calculate price-cost markups for the universe of public firms, using data from COMPUSTAT. The markup of a firm $j$ in a 2-digit NAICS sector $s$ at time $t$ is calculated as
\[
\mu_{sjt} = \xi_{st} \cdot \dfrac{\textrm{sale}_{sjt}}{\textrm{cogs}_{sjt}}
\]
where $ \xi_{st}$ is the elasticity of sales to the total variable input bundle, $\textrm{sale}_{sjt}$ is sales and $\textrm{cogs}_{sjt}$ is the cost of the goods sold, which measures total variable costs.

% To measure markup dispersion, we compute the standard deviation of markups within 2-digit NAICS sectors. Treating $ \xi_{st}$ as constant within a sector $s$ and time $t$, we can measure markup dispersion within this sector as

% \[
% \textrm{sd}_{s}\left[\textrm{log}\left(\mu_{sjt}\right)\right] = \textrm{sd}_{s}\left[\textrm{log}\left(\dfrac{\textrm{sale}_{sjt}}{\textrm{cogs}_{sjt}}\right)\right]
% \]

% We calculate this measure for all 23 sectors (2-digit NAICS). We then compute an average across all such sectors, weighted by the sector sales. Figure \ref{fig:Markup-Dispersion} shows the evolution of this measure.

% In our model, we compute the standard deviation of (log) markups across all firms in the economy, i.e. we do not compute it industry by industry. We think of an industry in our model as a market at the possible level of disaggregation (e.g. 10-digit NAICS). We cannot however observe data at such a fine level of disaggregation \textendash{} first because most data sets only provide industry information at the 6-digit, second because many large firms are multi-product an operate in different markets. We hence think of our final good $Y_t$ as one big-sector.

% \begin{figure}[H]
% \centering{}%
% \includegraphics*[scale=0.6]{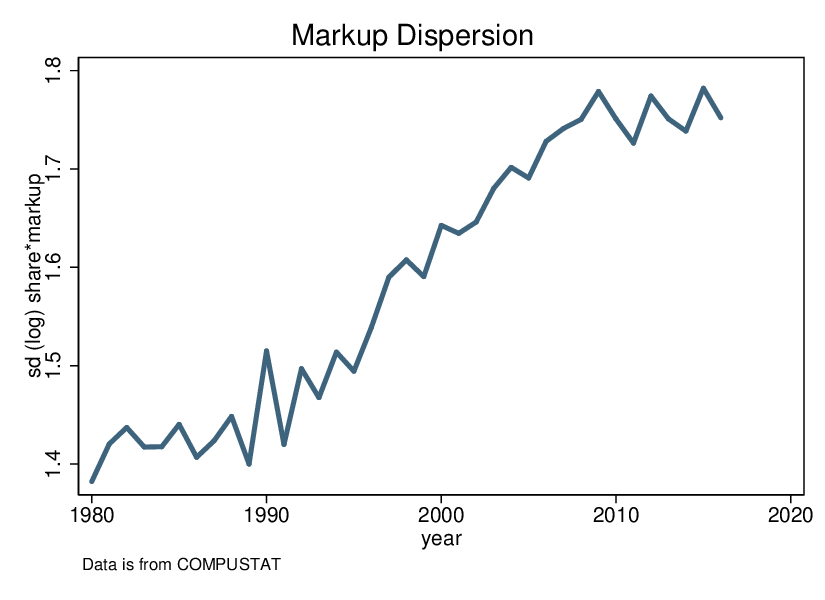}\tabularnewline
% \caption{Markup Dispersion\protect \\ {Note: \small{} the figure shows the evolution of markup dispersion computed from COMPUSTAT data for 2-digit industries.}
% \label{fig:Markup-Dispersion}}
% \end{figure}

\subsection{Solution Algorithm for the Dynamic Optimization Problem}

We now explain the algorithm we use for the dynamic optimization problem of the representative household. We take the calibrated parameters $\left(\lambda, c \right)$ and form a grid for aggregate capital with $n_K = 70 $ points. This grid is centered around the highest steady-state $K^{\text{ss}}_H$, with a lower-bound $0.5 \times K^{\text{ss}}_H$ and upper bound $1.5 \times K^{\text{ss}}_H$. We also form a grid for (log) aggregate TFP, $z$. We use Tauchen's algorithm with $n_z = 11$ points, autocorrelation parameter $\phi_Z$ and standard deviation for the innovations $\sigma_{\varepsilon}$ (the last two parameters are calibrated, as explained in the main text). We compute the aggregate equilibrium for each value of $K$ and $z$. 

We next compute a numerical approximation for the household policy function, by iterating on the Euler equation.

\subsection{Business Cycle Moments \label{subsec:business_cycle_moments}}

\begin{table}[H]
\setlength{\tabcolsep}{0.4cm}  
\begin{center}
\begin{tabular}{lccccc} 		\thickhline
\\[-2ex]
& Output & Consumption & Investment & Hours & TFP \\ \thickhline
\\[-2ex]
& \multicolumn{4}{c}{Correlation with Output} \\
\\[-2ex]
Data: 1947-2019 & 1.00 & 0.95 & 0.76 & 0.67 & 0.71 \\
Model: 1985 calibration & 1.00 & 1.00 & 0.96 & 1.00 & 0.34 \\
Model: 2007 calibration & 1.00 & 1.00 & 0.94 & 1.00 & 0.53  \\ 
\\
& \multicolumn{4}{c}{Standard Deviation Relative to Output} \\
\\[-2ex]
Data: 1947-2019 & 1.00 & 0.90 & 2.04 & 0.98 & 0.95 \\
Model: 1985 calibration & 1.00 & 0.95 & 1.19 & 0.78 & 0.09 \\
Model: 2007 calibration & 1.00 & 0.95 & 1.27 & 0.78 & 0.10  \\ 
\\[-2ex]\thickhline
\end{tabular} \end{center}
\caption{Business Cycle Moments. All variables are in logs. Data variables are in per capita terms (except TFP) and in deviation from a linear trend computed over 1947-2007.} \label{tab:business_cycle_moments}
\end{table}

Table \ref{tab:business_cycle_moments} shows some business cycle moments for our two calibrated economies, as well as their data counterparts.
To be consistent with our interpretation that the US economy transitioned to a lower steady-state after 2008, all data variables are in deviation from a linear trend computed over 1947-2007. This fact explains the large empirical correlation between consumption and output. 
Comparing our two calibrated economies, we see that both economies display the same correlations of consumption and hours with output. The 2007 economy displays, however, a significantly lower correlation of investment with output. %This is explained by the fact the investment appears to be more volatile in the 2007 economy.

\subsection*{Aggregate Productivity \label{subsec:agg_TFP}}

\subsubsection*{Average Firm Level TFP}

\begin{figure}[H]
\centering
\includegraphics*[scale=0.8]{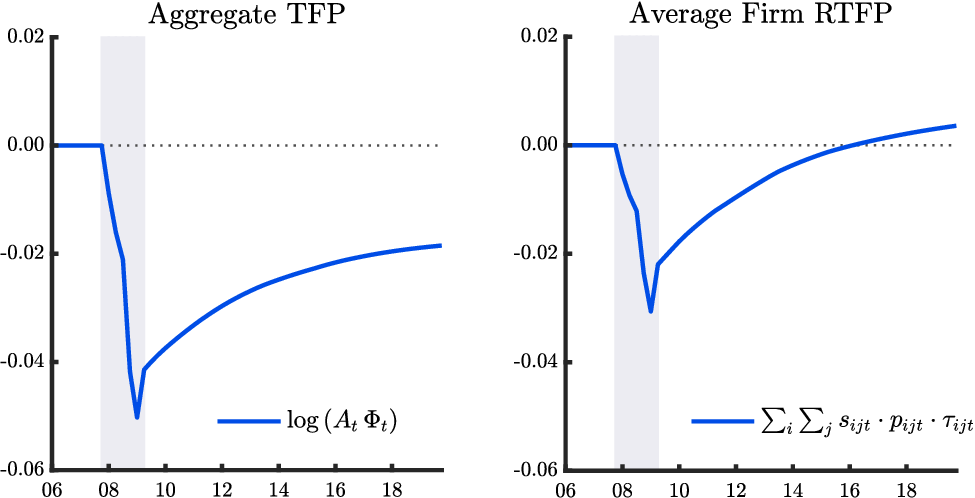}\caption{Aggregate TFP versus Average Firm Level TFP \protect \\
{Note: \small{}The left panel shows aggregate TFP. The right panel shows a sales-weighted average of firm level revenue TFP $p_{ijt}\cdot\tau_{ijt}$.
\label{fig:TFP_Model_transition}}}
\end{figure}

Figure \ref{fig:TFP_Model_transition} reports a sales-weighted average of firm level revenue TFP. A similar pattern emerges if one uses physical TFP instead.

\subsubsection*{Dispersion in Industry Output}

\begin{figure}[H]
\centering
\includegraphics*[scale=0.5]{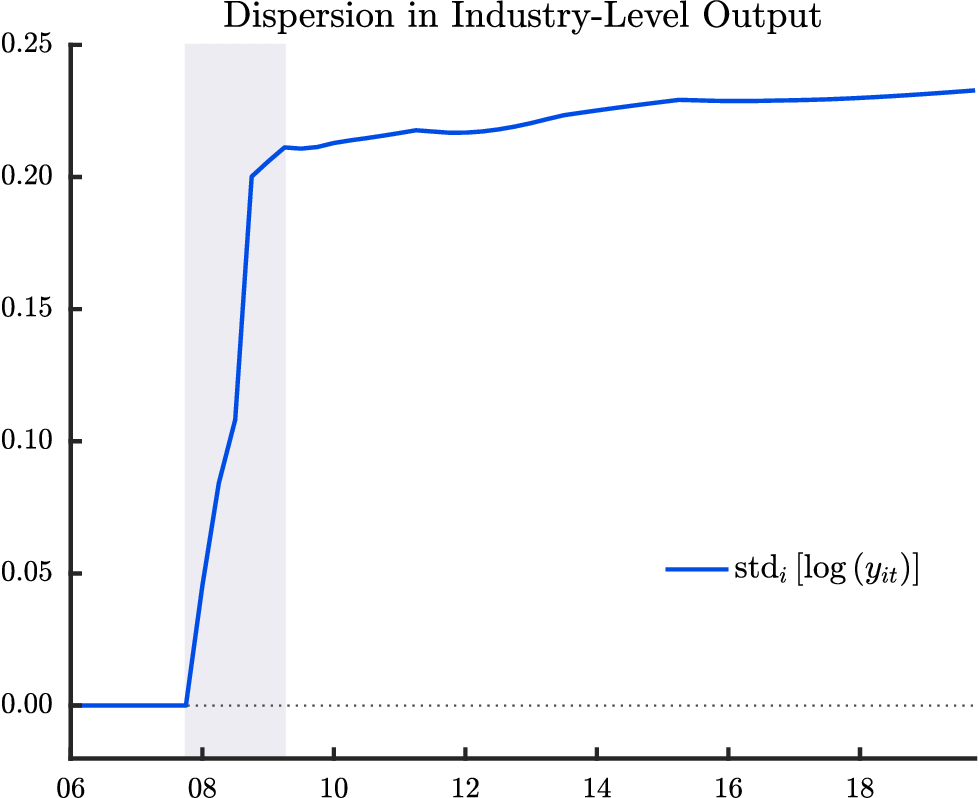}\caption{Dispersion in $\log\left(y_{it}\right)${\small{} \label{fig:output_dispersion_transition}}}
\end{figure}

%\subsection{The Great Recession}
% \subsection{Welfare \label{subsec:welfare_GR}}
% \begin{figure}[H]
% \centering
% \includegraphics*[scale=0.7]{input/GR_welfare_model}\caption{The great recession and its aftermath: welfare \label{fig:GR_welfare_model}}
% \end{figure}

\section{The 1981-1982 Recession \label{sec:82_recession}}

\subsubsection*{The response in the 1985 economy}

\begin{figure}[H]
\begin{minipage}[b]{.5\linewidth}
\centering{}\includegraphics*[scale=0.5]{input/data_82_recession.eps}\subcaption{1981-1982 recession (data) \label{fig:data_82_recession}}
\end{minipage}
\begin{minipage}[b]{.5\linewidth}
\centering{}\includegraphics*[scale=0.5]{input/1982_recession_1985_model.eps}\subcaption{The 1981-1982 shock in the 1985 model \label{fig:85_model_82_crisis}}
\end{minipage}
\caption{The 1981-1982 recession \label{fig:82_crisis}}
\end{figure}

\subsubsection*{The response in the 2007 economy}

\begin{figure}[H]
\centering{}\includegraphics*[scale=0.65]{input/1982_recession_2007_model.eps}
\caption{The 1981-1982 shock in the 2007 model
\label{fig:07_model_82_crisis}}
\end{figure}

\section{Policy Evaluation \label{sec:policy-evaluation}}

\begin{figure}[H]
\centering{}\includegraphics*[scale=0.5]{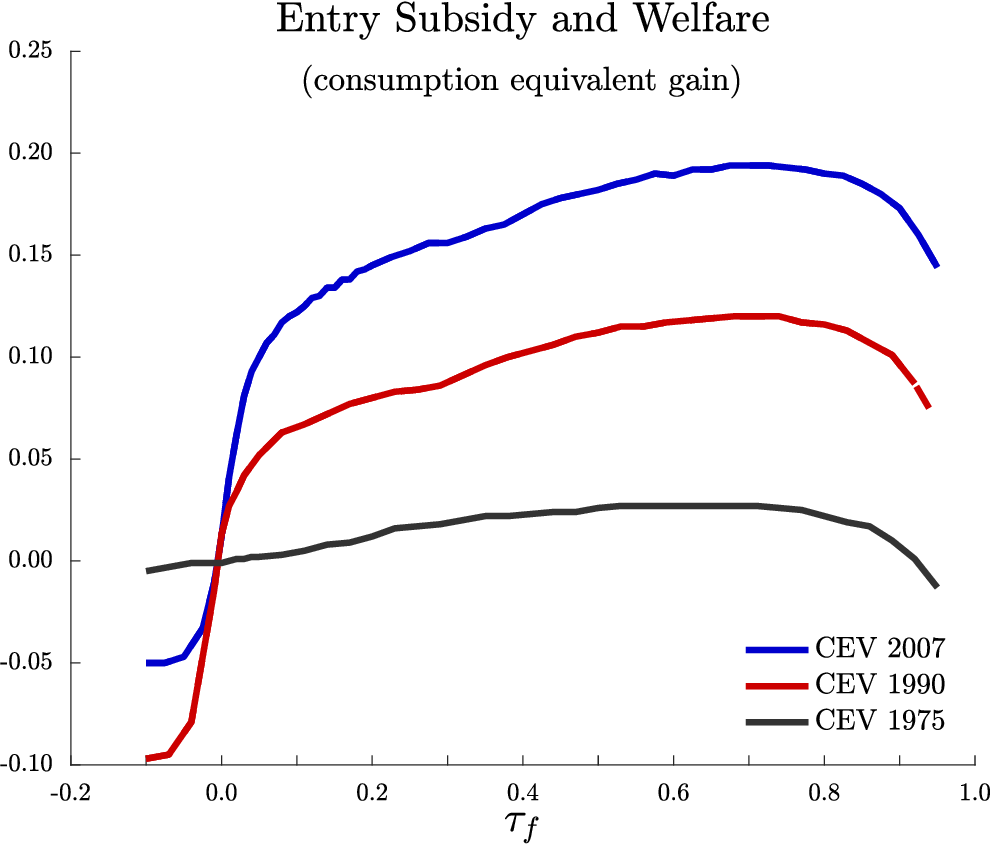}
\caption{Welfare: consumption equivalent gain
\label{fig:welfare_tau}}
\end{figure}
\raggedright Note: the figure shows the welfare impact (in consumption equivalent gains) of an entry subsidy equal to a fraction $\tau_f$ of fixed costs. For each level of  $\tau_f$, we simulate the economy 100,000 times and calculate average welfare.

\section{Regression Tables \label{sec:reg-tables}}

\begin{table}[H]
\setlength{\tabcolsep}{0.1cm}  \begin{center}
\scalebox{.8}{\begin{tabular}{lcccc} 				\thickhline
			\\[-2ex]
			 & (1) & (2) & (3) & (4) \\
			 \\[-1.5ex]
			VARIABLES & $\Delta \log \textrm{emp}_{07-16}$ & $\Delta \log \textrm{emp}_{07-16}$ & $\Delta \log \textrm{emp}_{07-16}$ & $\Delta \log \textrm{emp}_{07-16}$ \\
			\\[-1.5ex]
            \thickhline
			&  &  &  \\
			$ \textrm{concent}_{07} $ & -0.0223*** & -0.0160** & -0.0177*** & -0.0178** \\
			& (0.00667) & (0.00688) & (0.00682) & (0.00732) \\
			&  &  &  & \\
			$ \log \textrm{firms}_{07} $ &  & 0.00239*** & 0.00193*** & 0.00151 \\
			&  & (0.000705) & (0.000706) & (0.000983) \\
			&  &  &  & \\
			$\Delta \log \textrm{emp}_{03-07}$ &  &  & 0.0984*** & 0.0901*** \\
			&  &  & (0.0241) & (0.0247) \\
			&  &  &  &  \\
			Observations & 770 & 770 & 769 & 761 \\
			R-squared & 0.014 & 0.029 & 0.050 & 0.064 \\
			Sector FE & NO & NO & NO & YES \\ 
			\\[-2ex] \thickhline
			\\[-2ex]
			\multicolumn{5}{c}{ Standard errors in parentheses} \\
			\multicolumn{5}{c}{ *** p$<$0.01, ** p$<$0.05, * p$<$0.1} \\
\end{tabular} }
\caption{Change in Employment: 2007-2016\protect \\ {Note: \small{} the table shows the results of regressing the growth rate of sectoral employment between 2007 and 2016 on the measure of concentration in 2007. The table presents the results of progressively adding controls and, in the last column, sector fixed effects.}}
\label{tab:employment}
\end{center}
\end{table}

\begin{table}[H]
\setlength{\tabcolsep}{0.1cm}  \begin{center} 
\scalebox{.8}{\begin{tabular}{lcccc} 				\thickhline
			\\[-2ex]
			& (1) & (2) & (3) & (4) \\
			\\[-1.5ex]
			VARIABLES & $\Delta \log \textrm{payroll}_{07-16}$ & $\Delta \log \textrm{payroll}_{07-16}$ & $\Delta \log \textrm{payroll}_{07-16}$ & $\Delta \log \textrm{payroll}_{07-16}$ \\
			\\[-1.5ex]
            \thickhline
			&  &  &  \\
			$ \textrm{concent}_{07} $ & -0.0231*** & -0.0177** & -0.0189*** & -0.0194*** \\
		    & (0.00679) & (0.00702) & (0.00697) & (0.00749) \\
		    &  &  &  &  \\
			$ \log \textrm{firms}_{07} $ &  & 0.00203*** & 0.00164** & 0.000991 \\
			&  & (0.000724) & (0.000725) & (0.00101) \\
			&  &  &  &  \\
			$\Delta \log \textrm{payroll}_{03-07}$ &  &  & 0.0823*** & 0.0697*** \\
			&  &  & (0.0219) & (0.0225) \\
			&  &  &  &  \\
			Observations & 774 & 774 & 773 & 765 \\
			R-squared & 0.015 & 0.025 & 0.043 & 0.054 \\
			Sector FE & NO & NO & NO & YES \\ 
			\\[-2ex] \thickhline
			\\[-2ex]
			\multicolumn{5}{c}{ Standard errors in parentheses} \\
			\multicolumn{5}{c}{ *** p$<$0.01, ** p$<$0.05, * p$<$0.1} \\
\end{tabular} }
\end{center}
\caption{Change in Total Payroll: 2007-2016\protect \\ {Note: \small{} the table shows the results of regressing the growth rate of sectoral total payroll between 2007 and 2016 on the measure of concentration in 2007. The table presents the results of progressively adding controls and, in the last column, sector fixed effects.}}
\label{tab:payroll}
\end{table}

\begin{table}[H]
\setlength{\tabcolsep}{0.2cm}  \begin{center} 
\scalebox{.8}{\begin{tabular}{lcccc} 				\thickhline
			\\[-2ex]
			& (1) & (2) & (3) & (4) \\
			\\[-1.5ex]
			VARIABLES & $\Delta \log \textrm{firms}_{07-16}$ & $\Delta \log \textrm{firms}_{07-16}$ & $\Delta \log \textrm{firms}_{07-16}$ & $\Delta \log \textrm{firms}_{07-16}$ \\
			\\[-1.5ex]
            \thickhline
			&  &  &  \\
			$ \textrm{concent}_{07} $ & -0.0432*** & -0.0391*** & -0.0406*** & -0.0231*** \\
            & (0.00608) & (0.00637) & (0.00635) & (0.00666) \\
            &  &  &  &  \\
            $ \log \textrm{firms}_{07} $ &  & 0.00137** & 0.00119* & 0.00449*** \\
            &  & (0.000663) & (0.000661) & (0.000897) \\
            &  &  &  &  \\
            $\Delta \log \textrm{firms}_{03-07}$ &  &  & 0.0881*** & 0.0808*** \\
            &  &  & (0.0270) & (0.0273) \\
            &  &  &  &  \\
            Observations & 791 & 791 & 791 & 782 \\
            R-squared & 0.060 & 0.065 & 0.078 & 0.151 \\
			Sector FE & NO & NO & NO & YES \\ 
			\\[-2ex] \thickhline
			\\[-2ex]
			\multicolumn{5}{c}{ Standard errors in parentheses} \\
			\multicolumn{5}{c}{ *** p$<$0.01, ** p$<$0.05, * p$<$0.1} \\
\end{tabular} }
\end{center}
\caption{Change in Number of Firms: 2007-2016\protect \\ {Note: \small{} the table shows the results of regressing the growth rate of the industry number of firms between 2007 and 2016 on the measure of concentration in 2007. The table presents the results of progressively adding controls and, in the last column, sector fixed effects.}}
\label{tab:nfirms}
\end{table}

\begin{table}[H]
\setlength{\tabcolsep}{0.2cm}  \begin{center} 
\scalebox{.8}{\begin{tabular}{lcccc} 				\thickhline
			\\[-2ex]
			& (1) & (2) & (3) & (4) \\
			\\[-1.5ex]
			VARIABLES & $\Delta \textrm{lab\_share}_{07-16}$ & $\Delta \textrm{lab\_share}_{07-16}$ & $\Delta \textrm{lab\_share}_{07-16}$ & $\Delta \textrm{lab\_share}_{07-16}$ \\
			\\[-1.5ex]
            \thickhline
			&  &  &  \\
			$ \textrm{concent}_{07} $ & -0.0314* & -0.0319* & -0.0314* & -0.0301 \\
            & (0.0167) & (0.0168) & (0.0167) & (0.0196) \\
            &  &  &  &  \\
            $ \log \textrm{firms}_{07} $ &  & -0.00111 & -0.00120 & -0.00255 \\
            &  & (0.00240) & (0.00240) & (0.00335) \\
            &  &  &  &  \\
            $\Delta \textrm{lab\_share}_{03-07}$ &  &  & 0.169* & 0.146* \\
            &  &  & (0.0867) & (0.0871) \\
            &  &  &  &  \\
            Observations & 99 & 99 & 98 & 97 \\
            R-squared & 0.035 & 0.037 & 0.075 & 0.111 \\
			Sector FE & NO & NO & NO & YES \\ 
			\\[-2ex] \thickhline
			\\[-2ex]
			\multicolumn{5}{c}{ Standard errors in parentheses} \\
			\multicolumn{5}{c}{ *** p$<$0.01, ** p$<$0.05, * p$<$0.1} \\
\end{tabular} }
\end{center}
\caption{Change in Labor Share: 2007-2016\protect \\ {Note: \small{} the table shows the results of regressing the growth rate of sectoral labor share between 2007 and 2016 on the measure of concentration in 2007. The table presents the results of progressively adding controls and, in the last column, sector fixed effects.}}
\label{tab:labor_share}
\end{table}
