# Supplementary material for: Firm Heterogeneity, Market Power and Macroeconomic Fragility
Source: arXiv:2205.03908 source file (2024-05-10)
Supplement: Supplementary file 3 [file appendix_B.tex]

\newpage
\begin{center}
    
{\Huge {Appendix B} \\\normalsize Not for Publication}
\end{center}

\raggedright
\justify

\setcounter{page}{1}
\setcounter{section}{0}
\setcounter{figure}{0}
\setcounter{table}{0}
\setcounter{lemma}{0}

\makeatletter
\@addtoreset{section}{mysection}
\makeatother

\section{Number of Firms per Sector}
\label{sec:numberfirms}
\begin{figure}[ht!]
\begin{centering}
\includegraphics*[scale=0.9]{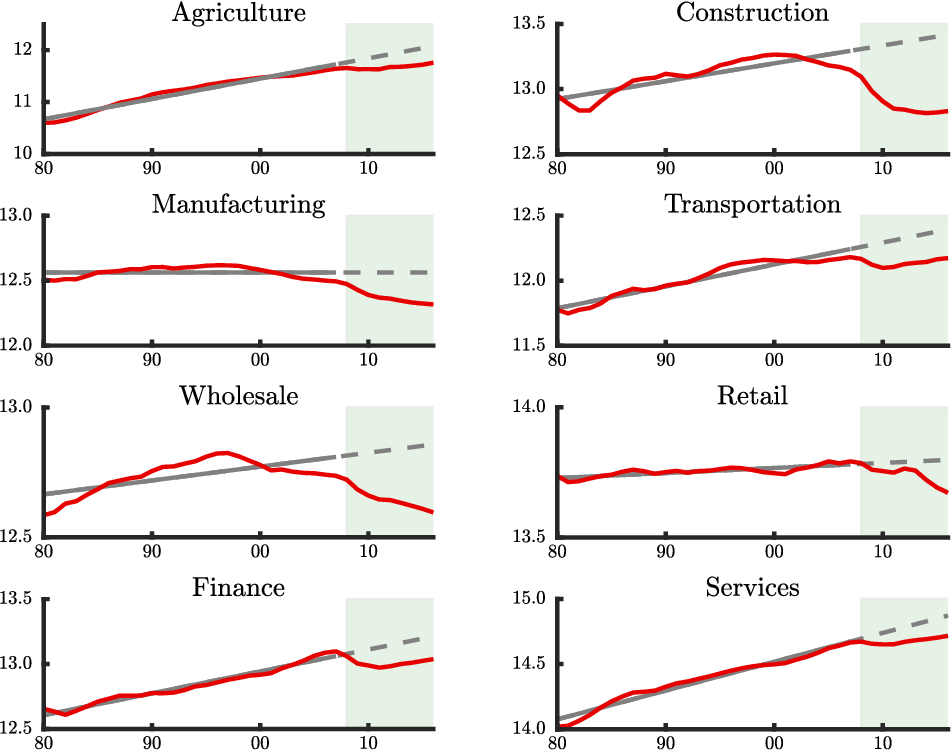} 
\par\end{centering}
\caption{\textbf{Number of Firms per Sector: 1980-2018}\protect \\
{\small{}Each panel shows the number of firms with at least one employee in each sector (in logs). For
each series, the dashed grey line shows a linear trend computed over the 1980-2007 period. Data is from the US Business Dynamics Statistics\label{fig:nfirms_sector}}}
\end{figure}

\section{Fixed Costs}\label{sec:fixed_costs_data}
\begin{figure}[ht!]
\centering{}%
\includegraphics*[scale=0.75]{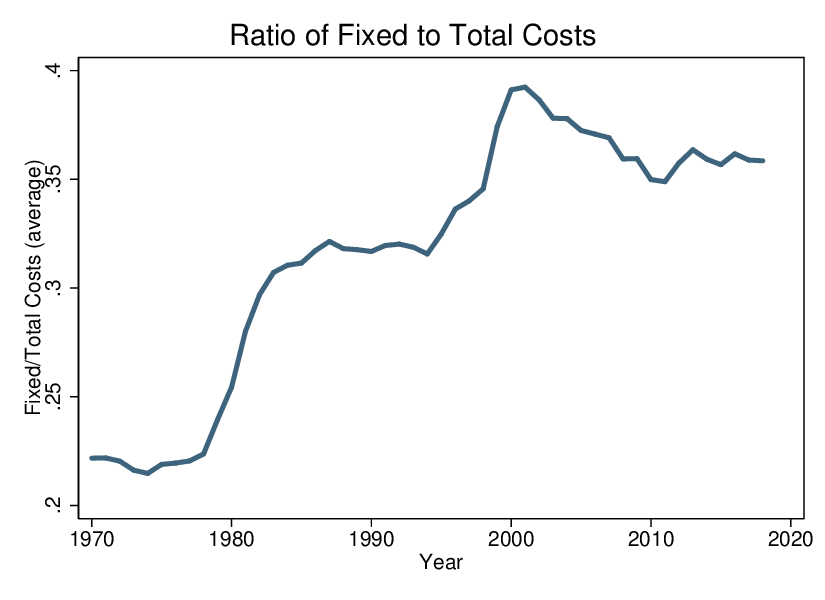}\tabularnewline
\caption{Ratio of fixed to total costs \\ This figure shows the average ratio of fixed to total costs for COMPUSTAT firms. Following \cite{GW}, we define fixed costs as the sum of 'Selling, General and Administrative Expenses' (COMPUSTAT item XSGA), 'Advertising Expenses'
(Compustat item XAD) and 'R\&D Expenditures'  (Compustat item XRD). Total costs are the sum of fixed costs and variable costs, where the latter correspond to the 'Cost of Goods Sold' (Compustat item COGS).
\label{fig:fixed_total_costs}}
\end{figure}

% \section{Labor Share: Alternative Measures \label{sec:alternative-labor-share}}

% As discussed by \cite{EHS}, measures of the aggregate labor share are sensitive to the treatment of the income of the self-employed. In its baseline measure, the BLS imputes to the self-employed the same hourly wage as that of payroll employees.

% In this section we construct two alternative measures. The first is the so called "economy-wide basis" measure; instead of imputing the same hourly wage to the self-employed, it inputs the same labor share as that for the overall economy (\cite{EHS}). The second is the labor share for the US corporate sector provided by the BEA (\cite{KN1}); by construction, this measure excludes by construction the noncorporate business sector.

% \begin{figure}[ht!]
% \begin{centering}
% \includegraphics*[scale=0.45]{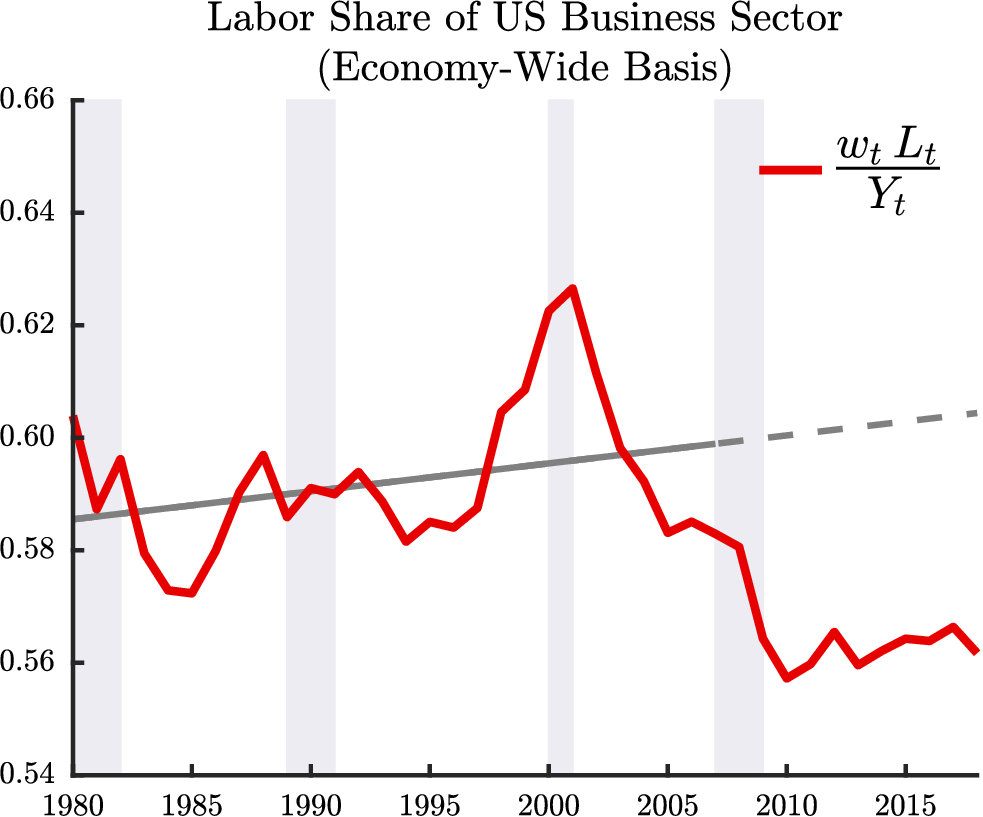} 
% \par\end{centering}
% \caption{\textbf{Labor Share (economy-wide basis): 1980-2018}\protect \\
% {\small{}  \label{fig:labor_share_ew}}}
% \end{figure}

% \begin{figure}[ht!]
% \begin{centering}
% \includegraphics*[scale=0.45]{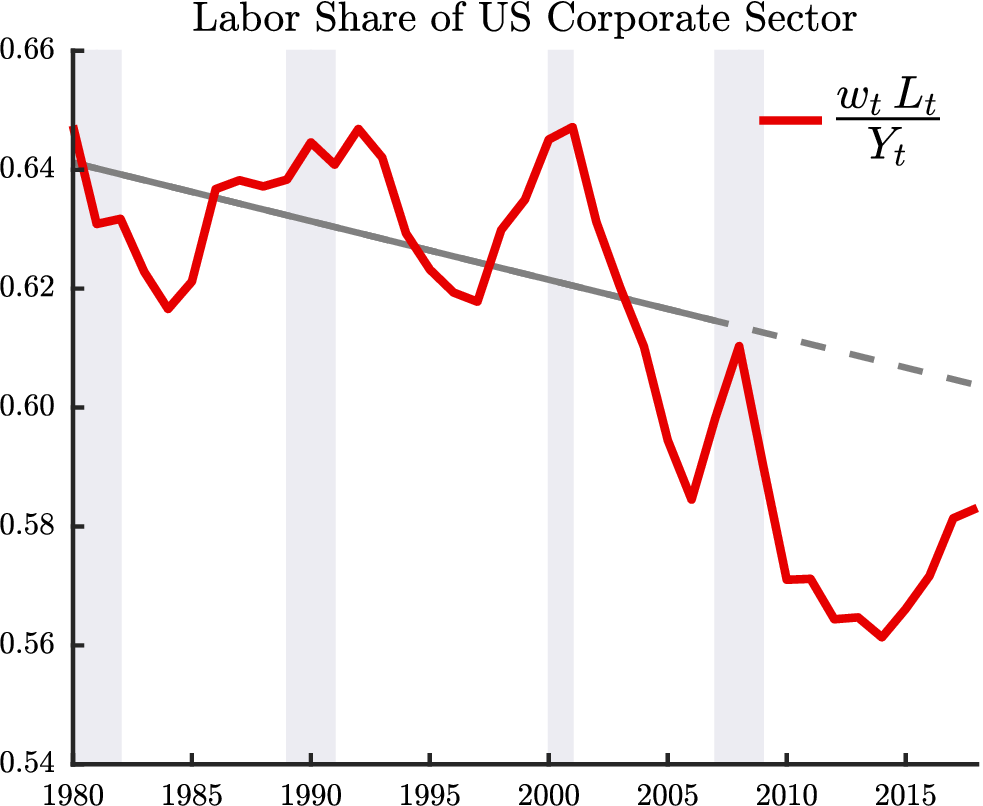} 
% \par\end{centering}
% \caption{\textbf{Labor Share (corporate sector): 1980-2018}\protect \\
% {\small{} \label{fig:labor_share_corporate}}}
% \end{figure}

% \newpage

\section[No Product Differentiation]{Industry Equilibrium with $\eta=1$}\label{proofs_appendixB}

\paragraph{Equilibrium Price and Output}
Suppose that $\eta=1$. When $n$ firms produce, we have a system of $n$ first order conditions
\begin{align}
p\left[1-\left(1-\rho\right)s_{j}\right]=\dfrac{\Theta}{\gamma_{j}}
\end{align}
Dividing the first order condition of firm $j$ by that of firm $1$
we obtain
\begin{align}
 %& \dfrac{1-\left(1-\rho\right)s_{j}}{1-\left(1-\rho\right)s_{1}}=\dfrac{\gamma_{1}}{\gamma_{j}}\\
%\Leftrightarrow & 1-\left(1-\rho\right)s_{j}=\dfrac{\gamma_{1}}{\gamma_{j}}\left[1-\left(1-\rho\right)s_{1}\right]\\
%\Leftrightarrow & 
s_{j}=\dfrac{1}{\left(1-\rho\right)}\left\{ 1-\dfrac{\gamma_{1}}{\gamma_{j}}\left[1-\left(1-\rho\right)s_{1}\right]\right\} 
\end{align}
Note that
\begin{align}
  \stackrel[k=1]{n}{\sum}s_{k}=1
 %\\
%\Leftrightarrow & \stackrel[k=1]{n}{\sum}\dfrac{1}{\left(1-\rho\right)}\left\{ 1-\dfrac{\gamma_{1}}{\gamma_{k}}\left[1-\left(1-\rho\right)s_{1}\right]\right\} =1\\
%\Leftrightarrow & n-\gamma_{1}\left[1-\left(1-\rho\right)s_{1}\right]\stackrel[k=1]{n}{\sum}\dfrac{1}{\gamma_{k}}=1-\rho\\
\Rightarrow  \dfrac{n-\left(1-\rho\right)}{\stackrel[k=1]{n}{\sum}\dfrac{1}{\gamma_{k}}}=\gamma_{1}\left[1-\left(1-\rho\right)s_{1}\right]
\end{align}
Plugging the last equation into the first order condition of firm
$1$ we obtain
\begin{align}
 %& p\dfrac{n-\left(1-\rho\right)}{\sum\limits_{k=1}^{n}\dfrac{1}{\gamma_{k}}}=\Theta\\
%\Leftrightarrow &
p=\dfrac{\sum\limits_{k=1}^{n}\dfrac{1}{\gamma_{k}}}{n-\left(1-\rho\right)}\Theta
\end{align}
Total output is hence equal to 
\begin{align}
 & y=p^{-\frac{1}{1-\rho}}Y=\left[\dfrac{\sum\limits_{k=1}^{n}\dfrac{1}{\gamma_{k}}}{n-\left(1-\rho\right)}\Theta\right]^{-\frac{1}{1-\rho}}Y
\end{align}

\paragraph{Market Shares}

Plugging the previous equation into the first order condition of firm
$j$ we have
\begin{align}
% & 1-\left(1-\rho\right)s_{j}=\dfrac{n-\left(1-\rho\right)}{\sum\limits_{k=1}^{n}\dfrac{1}{\gamma_{k}}}\dfrac{1}{\gamma_{j}}\\
%\Leftrightarrow & 
s_{j}=\dfrac{1}{1-\rho}\left[1-\dfrac{n-\left(1-\rho\right)}{\sum\limits_{k=1}^{n}\dfrac{1}{\gamma_{k}}}\dfrac{1}{\gamma_{j}}\right]
\end{align}
It is easy to verify that each firm's market share decreases in the
total number of active firms. To see this, suppose that the number
of firms increases from $n$ to $n+1$. The new entrant will have
a market share
\begin{align}
s_{n+1}=\dfrac{1}{1-\rho}\left[1-\dfrac{n+1-\left(1-\rho\right)}{\sum\limits_{k=1}^{n+1}\dfrac{1}{\gamma_{k}}}\dfrac{1}{\gamma_{n+1}}\right]
\end{align}
which is non-negative provided that
\begin{equation}
\gamma_{n+1}\sum_{k=1}^{n+1}\dfrac{1}{\gamma_{k}}>n+1-\left(1-\rho\right)\label{eq:cond_mg_1}
\end{equation}
and below one given that
\begin{equation}
\gamma_{n+1}\sum_{k=1}^{n+1}\dfrac{1}{\gamma_{k}}<\dfrac{1}{\rho}\left[n+1-\left(1-\rho\right)\right]\label{eq:cond_mg_2}
\end{equation}
If we compare the market share of firm $j$ when there $n$ and $n+1$
firms in the market, we have
\begin{align}
 & s_{j}\left|_{n+1}\right.<s_{j}\left|_n\right.
%\Leftrightarrow & \dfrac{1}{1-\rho}\left[1-\dfrac{n+1-\left(1-\rho\right)}{\sum\limits_{k=1}^{n+1}\dfrac{1}{\gamma_{k}}}\dfrac{1}{\gamma_{j}}\right]<\dfrac{1}{1-\rho}\left[1-\dfrac{n-\left(1-\rho\right)}{\sum\limits_{k=1}^{n}\dfrac{1}{\gamma_{k}}}\dfrac{1}{\gamma_{j}}\right]\\
%\Leftrightarrow & \dfrac{n-\left(1-\rho\right)}{\sum\limits_{k=1}^{n}\dfrac{1}{\gamma_{k}}}<\dfrac{n+1-\left(1-\rho\right)}{\sum\limits_{k=1}^{n+1}\dfrac{1}{\gamma_{k}}}\\
%\Leftrightarrow & \left[n-\left(1-\rho\right)\right]\left(\dfrac{1}{\gamma_{n+1}}+\sum\limits_{k=1}^{n}\dfrac{1}{\gamma_{k}}\right)<\left[n+1-\left(1-\rho\right)\right]\sum\limits_{k=1}^{n}\dfrac{1}{\gamma_{k}}\\
%\Leftrightarrow & \left[n-\left(1-\rho\right)\right]\dfrac{1}{\gamma_{n+1}}<\sum\limits_{k=1}^{n}\dfrac{1}{\gamma_{k}}\\
\Leftrightarrow  \gamma_{n+1}\sum\limits_{k=1}^{n+1}\dfrac{1}{\gamma_{k}}>n-\left(1-\rho\right)
\end{align}
Note that the last condition is implied by (\ref{eq:cond_mg_1}).

\paragraph{Profits}%\label{subsec:Profits}}

When there are $n$ active firms, type $\gamma_{j}$ makes production profits
\begin{align}
\Pi\left(\gamma_{j},n,\Gamma,\Theta,Y\right) %& =\left(p-\dfrac{\Theta}{\gamma_{j}}\right)s_{j}\:y_{j} \\
 & = \underbrace{\dfrac{1}{1-\rho}\left[1-\dfrac{n-\left(1-\rho\right)}{\sum\limits_{k=1}^{n}\dfrac{1}{\gamma_{k}}}\dfrac{1}{\gamma_{j}}\right]^{2}\left[\dfrac{n-\left(1-\rho\right)}{\sum\limits_{k=1}^{n}\dfrac{1}{\gamma_{k}}}\right]^{\frac{\rho}{1-\rho}}}_{\equiv \varLambda\left(\gamma_{j},n,\Gamma\right)}\Theta^{-\frac{\rho}{1-\rho}}Y
\end{align}
\begin{lemma}
\label{lemma:(Profit-Function)} When $\eta=1$, the profit function \textup{$\Pi\left(j,n_{it},\Gamma_{i},X_{t}\right)$}
satisfies
\begin{align} 
1) & \dfrac{\partial\Pi\left(j,n_{it},\Gamma_{i},X_{t}\right)}{\partial Y_{t}}\vphantom{\vphantom{\dfrac{\dfrac{1}{1}}{\frac{_{1}}{1}}}}>0  \qquad 
2) & \dfrac{\partial\Pi\left(j,n_{it},\Gamma_{i},X_{t}\right)}{\partial n_{it}}\vphantom{\vphantom{\dfrac{\dfrac{1}{1}}{\frac{_{1}}{1}}}}<0  \quad,\;n_{it}>j \\
3) & \dfrac{\partial\Pi\left(j,n_{it},\Gamma_{i},X_{t}\right)}{\partial\gamma_{ij}}\vphantom{\dfrac{\dfrac{1}{1}}{\frac{_{1}}{1}}}>0 \qquad
4) & \dfrac{\partial\Pi\left(j,n_{it},\Gamma_{i},X_{t}\right)}{\partial\gamma_{ik}}\vphantom{\vphantom{\dfrac{\dfrac{1}{1}}{\frac{_{1}}{1}}}}<0  \quad,\;\forall k\neq j.
\end{align}
\end{lemma}
\begin{proof} [Proof of Lemma \ref{lemma:(Profit-Function)}]
We start by showing that $\Pi\left(\cdot\right)$ increases in $\gamma_{j}$
\begin{align}
 & 2\left[1-\dfrac{n-\left(1-\rho\right)}{\sum\limits_{k=1}^{n}\dfrac{1}{\gamma_{k}}}\dfrac{1}{\gamma_{j}}\right]^{-1}\left\{ -\dfrac{-\left[n-\left(1-\rho\right)\right]\left[-\left(\dfrac{1}{\gamma_{j}}\right)^{2}\right]}{\left(\sum\limits_{k=1}^{n}\dfrac{1}{\gamma_{k}}\right)^{2}}\dfrac{1}{\gamma_{j}}+\dfrac{n-\left(1-\rho\right)}{\sum\limits_{k=1}^{n}\dfrac{1}{\gamma_{k}}}\left(\dfrac{1}{\gamma_{j}}\right)^{2}\right\} + \\
 & \dfrac{\rho}{1-\rho}\left[\dfrac{n-\left(1-\rho\right)}{\sum\limits_{k=1}^{n}\dfrac{1}{\gamma_{k}}}\right]^{-1}\dfrac{-\left[n-\left(1-\rho\right)\right]\left[-\left(\dfrac{1}{\gamma_{j}}\right)^{2}\right]}{\left(\sum\limits_{k=1}^{n}\dfrac{1}{\gamma_{k}}\right)^{2}}>0\\
%\Leftrightarrow & 2\left[1-\dfrac{n-\left(1-\rho\right)}{\sum\limits_{k=1}^{n}\dfrac{1}{\gamma_{k}}}\dfrac{1}{\gamma_{j}}\right]^{-1}\left\{ -\dfrac{1}{\left(\sum\limits_{k=1}^{n}\dfrac{1}{\gamma_{k}}\right)^{2}}\dfrac{1}{\gamma_{j}}+\dfrac{1}{\sum\limits_{k=1}^{n}\dfrac{1}{\gamma_{k}}}\right\} + \\
%& \dfrac{\rho}{1-\rho}\left[\dfrac{n-\left(1-\rho\right)}{\sum\limits_{k=1}^{n}\dfrac{1}{\gamma_{k}}}\right]^{-1}\dfrac{1}{\left(\sum\limits_{k=1}^{n}\dfrac{1}{\gamma_{k}}\right)^{2}}>0\\
%\Leftrightarrow & 2\left[1-\dfrac{n-\left(1-\rho\right)}{\sum\limits_{k=1}^{n}\dfrac{1}{\gamma_{k}}}\dfrac{1}{\gamma_{j}}\right]^{-1}\left\{ -\dfrac{1}{\gamma_{j}}+\sum\limits_{k=1}^{n}\dfrac{1}{\gamma_{k}}\right\} +\dfrac{\rho}{1-\rho}\left[\dfrac{n-\left(1-\rho\right)}{\sum\limits_{k=1}^{n}\dfrac{1}{\gamma_{k}}}\right]^{-1}\dfrac{1}{\left(\sum\limits_{k=1}^{n}\dfrac{1}{\gamma_{k}}\right)^{2}}>0\\
\Leftrightarrow & 2\left[1-\dfrac{n-\left(1-\rho\right)}{\sum\limits_{k=1}^{n}\dfrac{1}{\gamma_{k}}}\dfrac{1}{\gamma_{j}}\right]^{-1}\left(\sum\limits_{k\neq j}^{n}\dfrac{1}{\gamma_{k}}\right)+\dfrac{\rho}{1-\rho}\left[\dfrac{n-\left(1-\rho\right)}{\sum\limits_{k=1}^{n}\dfrac{1}{\gamma_{k}}}\right]^{-1}>0
\end{align}
To prove points (ii) and (iii) it suffices to show that $\varLambda\left(\cdot\right)$
is decreasing in $[{n-\left(1-\rho\right)}]/\left[{\sum\limits_{k=1}^{n}\dfrac{1}{\gamma_{k}}}\right]$
\begin{align}
 & 2\left[1-\dfrac{n-\left(1-\rho\right)}{\sum\limits_{k=1}^{n}\dfrac{1}{\gamma_{k}}}\dfrac{1}{\gamma_{j}}\right]^{-1}\left(-\dfrac{1}{\gamma_{j}}\right)+\dfrac{\rho}{1-\rho}\left[\dfrac{n-\left(1-\rho\right)}{\sum\limits_{k=1}^{n}\dfrac{1}{\gamma_{k}}}\right]^{-1}<0\\
%\Leftrightarrow & \dfrac{\rho}{1-\rho}\left[1-\dfrac{n-\left(1-\rho\right)}{\sum\limits_{k=1}^{n}\dfrac{1}{\gamma_{k}}}\dfrac{1}{\gamma_{j}}\right]<2\left[\dfrac{n-\left(1-\rho\right)}{\sum\limits_{k=1}^{n}\dfrac{1}{\gamma_{k}}}\right]\dfrac{1}{\gamma_{j}}\\
%\Leftrightarrow & \dfrac{\rho}{1-\rho}<\left(2+\frac{\rho}{1-\rho}\right)\left[\dfrac{n-\left(1-\rho\right)}{\sum\limits_{k=1}^{n}\dfrac{1}{\gamma_{k}}}\right]\dfrac{1}{\gamma_{j}}\\
%\Leftrightarrow & \rho<\left(2-\rho\right)\left[\dfrac{n-\left(1-\rho\right)}{\sum\limits_{k=1}^{n}\dfrac{1}{\gamma_{k}}}\right]\dfrac{1}{\gamma_{j}}\\
\Leftrightarrow & \gamma_{j}\sum\limits_{k=1}^{n}\dfrac{1}{\gamma_{k}}<\dfrac{2-\rho}{\rho}\left[n-\left(1-\rho\right)\right]
\end{align}
The last condition is implied by (\ref{eq:cond_mg_2}).
\end{proof}

\section{Derivations: General Equilibrium}\label{sec:GEderivations}

\subsection{Aggregate TFP \label{subsec:Aggregate-TFP} }
Aggregate TFP is given by
\begin{equation}
\Phi\left(\mathbf{\Gamma},\mathbf{N}_{t}\right)=\left[\sum_{i=1}^{I}\left(\sum_{j=1}^{n_{it}}\omega_{ijt}^{\eta}\right)^{\frac{\rho}{\eta}}\right]^{\frac{1}{\rho}}\left(\sum_{i=1}^{I}\sum_{j=1}^{n_{it}}\dfrac{\omega_{ijt}}{\tau_{ijt}}\right)^{-1},\label{eq:agg_tfp}
\end{equation}
where
\begin{align}
\omega_{ijt}\coloneqq\left[\sum_{k=1}^{n_{it}}\left(\dfrac{\mu_{ikt}}{\tau_{ikt}}\right)^{\frac{\eta}{1-\eta}}\right]^{\frac{\eta-\rho}{\eta}\frac{1}{1-\rho}}\left(\dfrac{\tau_{ijt}}{\mu_{ijt}}\right)^{\frac{1}{1-\eta}}.
\end{align}

\subsection{Factor Prices and Factor Shares \label{subsec:Factor-Prices} }
We can aggregate firms' best responses, given by equation (\ref{eq:firm_FOC}), to find an expression for the aggregate factor cost index. Given a $\left(I\times M\right)$
matrix of productivity draws $\mathbf{A}_{t}$ and a vector of active firms $\mathbf{N}_{t} \equiv \left\{ n_{it}\right\}_{i=1}^{I}$, the equilibrium factor cost index is equal to
\begin{equation}
\Theta\left(\mathbf{A}_{t},\mathbf{N}_{t}\right)=\left\{ \sum_{i=1}^{I}\left[\sum_{j=1}^{n_{it}}\left(\dfrac{\tau_{ijt}}{\mu_{ijt}}\right)^{\frac{\eta}{1-\eta}}\right]^{\frac{1-\eta}{\eta}\frac{\rho}{1-\rho}}\right\} ^{\frac{1-\rho}{\rho}}.
\end{equation}

The aggregate factor share $\Omega\left(\cdot\right) = \left(W_{t}\,L_{t} + R_{t}\,K_{t} \right)/Y_{t} $ is equal to
\begin{equation}
\Omega\left(\mathbf{A}_{t},\mathbf{N}_{t}\right) = \dfrac{\Theta\left(\mathbf{A}_{t},\mathbf{N}_{t}\right)}{\Phi\left(\mathbf{A}_{t},\mathbf{N}_{t}\right)} .
\end{equation}

\subsection{Asymmetric Equilibrium\label{subsec:Asymmetric Equilibrium}}

When
\begin{align}
\overline{K}\left(\Gamma,n\right) <  K < \underline{K}\left(\Gamma,n+1\right)
\end{align}
there will be an asymmetric equilibrium at time $t+1$:
some industries will contain $n$ firms, whereas some industries will
contain $n+1$ firms. The fraction of industries with $n+1$ will
be pinned down by a zero profit condition for the marginal entrant
in an industry with $n+1$ firms
\begin{align}
\varLambda\left(\Gamma,\gamma_{n+1},n+1\right)\Theta^{-\frac{\rho}{1-\rho}}Y=c_{i}
\end{align}

The equilibrium is characterized by 4 variables: 
the fraction of the industries
with $n+1$ firms ($\eta$), aggregate output ($Y$), aggregate productivity ($\Phi$) and the aggregate cost index ($\Theta$). These 4 variables are pinned down by the following 4 equations

\begin{align}
Y=\Phi\left[\left(1-\alpha\right)\Theta\right]^{\frac{1-\alpha}{\nu+\alpha}}K^{\alpha\frac{1+\nu}{\nu+\alpha}}\\
\Phi=\dfrac{\left\{ \left(1-\eta\right)\left[\dfrac{n-\left(1-\rho\right)}{\sum\limits_{k=1}^{n}\dfrac{1}{\gamma_{1k}}}\right]^{\frac{\rho}{1-\rho}}+\eta\left[\dfrac{n+1-\left(1-\rho\right)}{\sum\limits_{k=1}^{n+1}\dfrac{1}{\gamma_{2k}}}\right]^{\frac{\rho}{1-\rho}}\right\} ^{\frac{1}{\rho}}}{\left(1-\eta\right)\left[\dfrac{n-\left(1-\rho\right)}{\sum\limits_{k=1}^{n}\dfrac{1}{\gamma_{1k}}}\right]^{\frac{1}{1-\rho}}\left(\sum\limits_{k=1}^{n}\dfrac{s_{1k}}{\gamma_{1k}}\right)+\eta\left[\dfrac{n+1-\left(1-\rho\right)}{\sum\limits_{k=1}^{n+1}\dfrac{1}{\gamma_{2k}}}\right]^{\frac{1}{1-\rho}}\left(\sum\limits_{k=1}^{n+1}\dfrac{s_{2k}}{\gamma_{2k}}\right)\vphantom{\left[\dfrac{\dfrac{\sum\limits_{k}^{n}\dfrac{1}{\gamma}}{1}}{\dfrac{\sum\limits_{k}^{n}\dfrac{1}{\gamma}}{1}}\right]}}\\
\Theta=\left\{ \left(1-\eta\right)\left[\dfrac{n-\left(1-\rho\right)}{\sum\limits_{k=1}^{n}\dfrac{1}{\gamma_{k}}}\right]^{\frac{\rho}{1-\rho}}+\eta\left[\dfrac{n+1-\left(1-\rho\right)}{\sum\limits_{k=1}^{n+1}\dfrac{1}{\gamma_{k}}}\right]^{\frac{\rho}{1-\rho}}\right\} ^{\frac{1-\rho}{\rho}}\vphantom{\left[\dfrac{\dfrac{\sum\limits_{k}^{n}\dfrac{1}{\gamma}}{1}}{\dfrac{\sum_{k}^{n}\dfrac{1}{\gamma}}{1}}\right]}\\
\varLambda\left(\Gamma,\gamma_{n+1},n+1\right)\Theta^{-\frac{\rho}{1-\rho}}Y=c_{i}
\end{align}

$s_{1k}$ is the market share of firm $k$ in an industry with $n$ firms, whereas $s_{2k}$ is the market share of firm $k$ in an industry with $n+1$ firms. They are defined in Appendix
\ref{proofs_appendixB}.

\section{The Baseline Model}\label{appendix:baseline-model}

\subsection*{Comparative Statics with $\uparrow \gamma_{1}$ and $\leftrightarrow \gamma_{2}$ (mean-increasing spread)}
\begin{figure}[H]
\centering{}
\hspace{-0.2cm}
 \includegraphics*[scale=0.475]{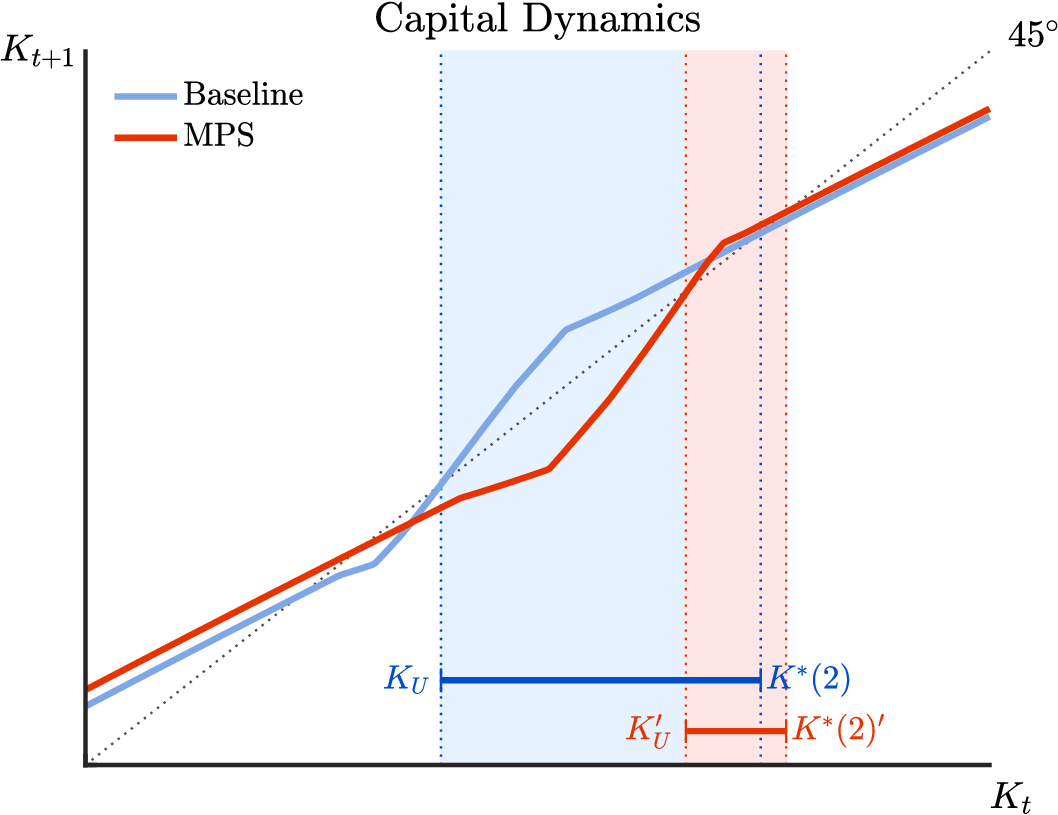}
 \hspace{0.4cm}
 \includegraphics*[scale=0.475]{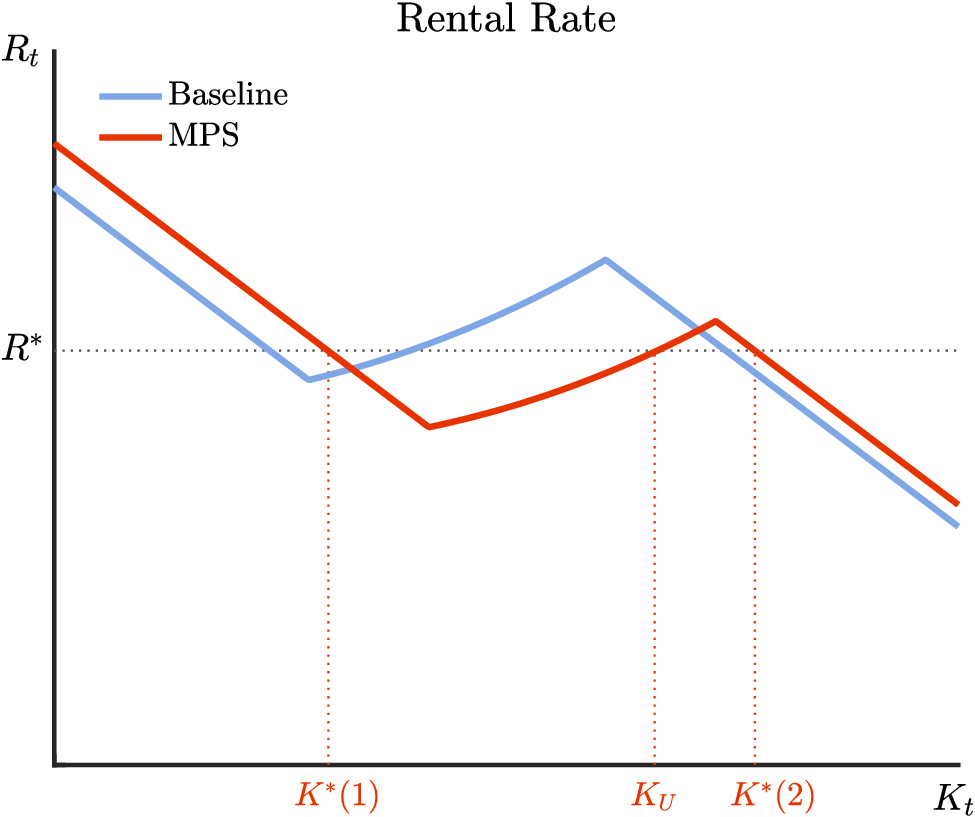}
\caption{Law of Motion and Rental Rate Map \label{fig:Law-of-Motion-MIS}
\protect \\ {This example features two stable steady states and an unstable one. We use $\psi \, = \, 1 \,$,  $\rho \, = \, 3/4 \,$, $\eta \, = \, 1 \,$, $\alpha \, = \, 1/3 \,$, $\delta \, = \, 1 \,$, $\nu \, = \, 2/5 \,$ and $ c_{i} \, = \, 0.015 \,$.}} 
\end{figure}

\subsection*{Steady-State Multiplicity}
\begin{figure}[H]
\centering{}
\hspace{-0.2cm}
 \includegraphics*[scale=0.475]{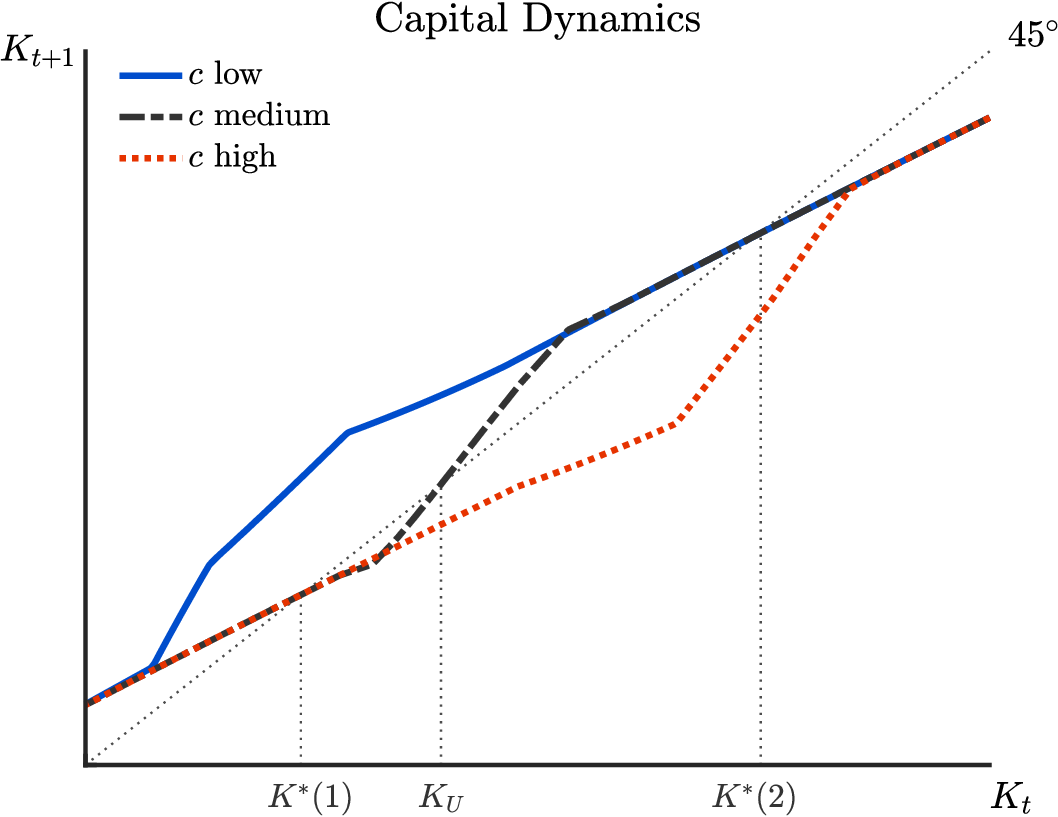}
 \hspace{0.4cm}
 \includegraphics*[scale=0.475]{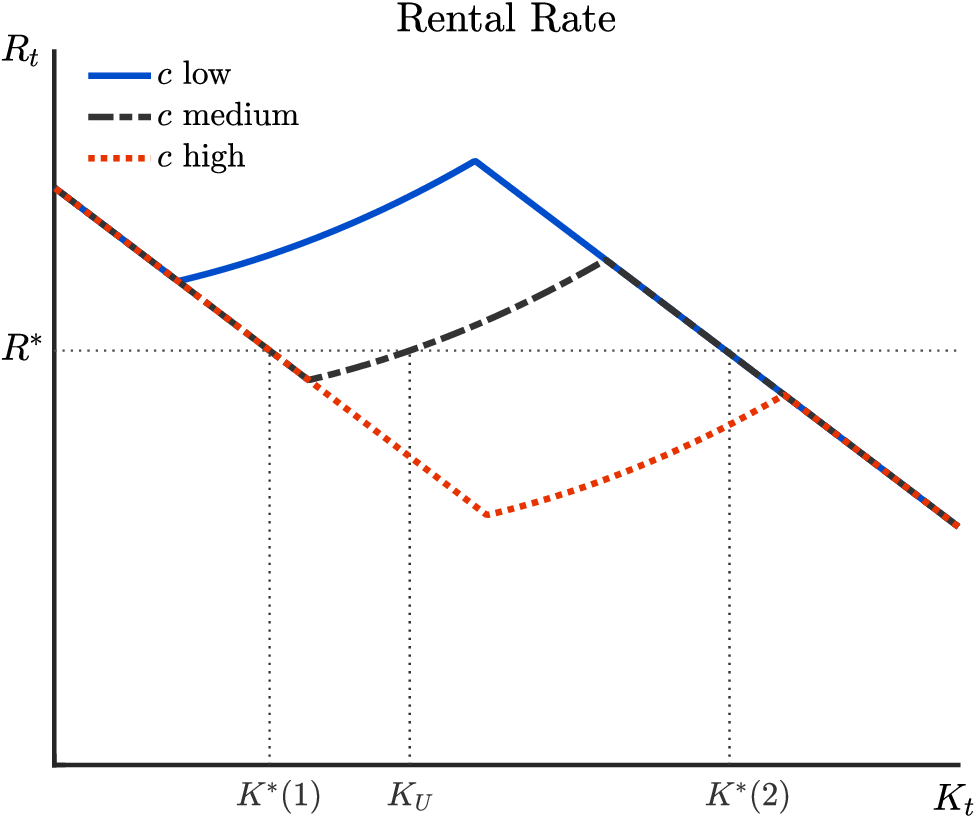}
\caption{Law of Motion and Rental Rate Map \label{fig:Law-of-Motion-existence}
\protect \\ {This example features two stable steady states and an unstable one. We use $\psi \, = \, 1 \,$,  $\rho \, = \, 3/4 \,$, $\eta \, = \, 1 \,$, $\alpha \, = \, 1/3 \,$, $\delta \, = \, 1 \,$ and $\nu \, = \, 2/5 $.}} 
\end{figure}

\section{Proofs and Additional Results for Section \ref{sec:Model} \label{Proofs-Additional-Results}}

\subsubsection*{Proof of Lemma \ref{aggregate_factor_share_lem}}
\begin{proof}
Using equation (\ref{eq:agg_factor_share_HHI}) and imposing $\eta=1$ and symmetry we obtain $\Omega(\Gamma_n, n)=1-(1-\rho)HHI_t$ where $HHI_t$ is the Herfindhal-Hirschman Index of the economy. As $\rho<1$ the aggregate factor share decreases in concentration, as measured by HHI. The latter is trivially decreasing in $n$, which proves the first part of the lemma.
Furthermore, a mean-preserving spread of productivity, holding $n$ fixed, implies a spread of the market shares distribution. Since HHI is a convex function of market shares, it necessarily increases after a spread of the productivity distribution. The statement follows. 
\end{proof}

% \begin{lemma}[Labor Response]\label{lemma:signL}
% If the labor supply is upward sloping and wages increase in $\Theta\left(\cdot\right)$ (for fixed $K$), the labor response to changes in the technology fundamental $\lambda$ has the same sign as the effect on the function $\Theta(\cdot): \sgn\{L_\lambda\}=\sgn\{\Theta_\lambda\}.$
% \end{lemma}

% \begin{proof}[Proof of Lemma \ref{lemma:signL}]
% We want to sign $L_\lambda$. We start by noting that $L_\lambda=L_w w_\lambda$. Note that we can write the equivalent of equation \ref{rmap} for the wage: $ w=\Theta(\Lambda,n)F_L$, where $F=F(K,L)$.  Further, $\sgn\{w_\lambda\}=\sgn\{\Theta_\lambda\}$. Therefore, provided that $L_w>0$ the statement follows.
% \end{proof}

\subsubsection*{Proof of Proposition \ref{A-symmetric-equilibrium}}

\begin{proof}
Suppose $\eta=1$.When there are $n$ active firms in a given industry, the profits of a firm with productivity $\gamma_{j}$ are equal to
\begin{align}
\Pi\left(\gamma_{j},n,\Gamma,\Theta,Y\right) = \varLambda\left(\gamma_{j},n,\Gamma\right) \Theta^{-\frac{\rho}{1-\rho}}Y
\end{align}
where
$\varLambda\left(\gamma_{j},n,\Gamma\right)$ has been defined in Appendix \ref{proofs_appendixB}. A symmetric equilibrium with $n$ firms per industry is possible provided that
\begin{align*}
    \varLambda\left(\gamma_{n},n,\Gamma\right) \Theta^{-\frac{\rho}{1-\rho}}Y & \geq c \\
    \varLambda\left(\gamma_{n+1},n+1,\Gamma\right) \Theta^{-\frac{\rho}{1-\rho}}Y & \leq c
\end{align*}
Using equation (\ref{eq:agg_output_capital}), we can write the above inequalities as 
\begin{align}
\underline{K}\left(\Gamma,n\right)\leq K_{t}\leq\overline{K}\left(\Gamma,n\right),
\end{align}
where
\begin{align}
\underline{K}\left(\Gamma,n\right) = \left\{ \dfrac{c}{\varLambda\left(\gamma_{n},n,\Gamma\right)}\left(1-\alpha\right)^{-\frac{1-\alpha}{\nu+\alpha}}\left[\Phi\left(\Gamma,n\right)\right]^{-1}\left[\Theta\left(\Gamma,n\right)\right]^{\frac{\rho}{1-\rho}-\frac{1-\alpha}{\nu+\alpha}}\right\} ^{\frac{\nu+\alpha}{\alpha\left(1+\nu\right)}} \\
\overline{K}\left(\Gamma,n\right) = \left\{ \dfrac{c}{\varLambda\left(\gamma_{n+1},n+1,\Gamma\right)}\left(1-\alpha\right)^{-\frac{1-\alpha}{\nu+\alpha}}\left[\Phi\left(\Gamma,n\right)\right]^{-1}\left[\Theta\left(\Gamma,n\right)\right]^{\frac{\rho}{1-\rho}-\frac{1-\alpha}{\nu+\alpha}}\right\} ^{\frac{\nu+\alpha}{\alpha\left(1+\nu\right)}}.
\end{align}

The condition on uniqueness can be derived by noting that it arises if and only if the following holds $\forall n$
\[
\begin{array}{cl}
 & \underline{K}\left(\Gamma,n+1\right)>\overline{K}\left(\Gamma,n\right)\\[2ex]
\Leftrightarrow & \left[\Phi\left(\Gamma,n+1\right)\right]^{-1}\left[\Theta\left(\Gamma,n+1\right)\right]^{\frac{\rho}{1-\rho}-\frac{1-\alpha}{\nu+\alpha}}>\left[\Phi\left(\Gamma,n\right)\right]^{-1}\left[\Theta\left(\Gamma,n\right)\right]^{\frac{\rho}{1-\rho}-\frac{1-\alpha}{\nu+\alpha}}\\[2ex]
\Leftrightarrow & \dfrac{\Phi\left(\Gamma,n\right)}{\Phi\left(\Gamma,n+1\right)}>\left[\dfrac{\Theta\left(\Gamma,n\right)}{\Theta\left(\Gamma,n+1\right)}\right]^{\frac{\rho}{1-\rho}-\frac{1-\alpha}{\nu+\alpha}}
\end{array}
\]
Therefore, when there are no productivity differences across firms, the condition becomes
\[
\begin{array}{cl}
 & \left[\dfrac{\Theta\left(\Gamma,n\right)}{\Theta\left(\Gamma,n+1\right)}\right]^{\frac{\rho}{1-\rho}-\frac{1-\alpha}{\nu+\alpha}}<1\\[2ex]
\Leftrightarrow & \dfrac{\rho}{1-\rho}-\dfrac{1-\alpha}{\nu+\alpha}>0\\[2ex]
\Leftrightarrow & \dfrac{\rho}{1-\rho}>\dfrac{1-\alpha}{\nu+\alpha}
\end{array}
\]
since $\Theta\left(\Gamma,n+1\right)>\Theta\left(\Gamma,n\right)$.
\end{proof}

%\subsection{Savings Rate Lemmas \label{subsec:Proof-prop}}

\subsubsection*{Proof of Lemma \ref{lemma:savings_rate}}

\begin{proof}
In a steady-state we have a constant rental rate
\begin{align}
R^{*} = \beta^{-1} - \left(1-\delta\right)
\end{align}
and
\begin{align}
\delta  K = s Y
\end{align}
Combining these two equations with equation (\ref{eq:factor_demand}) we obtain
\begin{align}\nonumber
 & \beta^{-1}-\left(1-\delta\right)=\alpha\;\Omega\left(\mathbf{\Gamma},\mathbf{N}\right)\;\dfrac{Y^{*}}{K^{*}}\\\nonumber
\Leftrightarrow & \beta^{-1}-\left(1-\delta\right)=\alpha\;\Omega\left(\mathbf{\Gamma},\mathbf{N}\right)\;\dfrac{\delta}{s^{*}}\\
\Leftrightarrow & s^{*}=\dfrac{\delta\;\alpha}{\beta^{-1}-\left(1-\delta\right)}\Omega\left(\mathbf{\Gamma},\mathbf{N}\right)
\end{align}
\end{proof}

\subsubsection*{Proof of Proposition \ref{prop:multiplicity}}
\begin{proof}
We have
\[
R_{t}\;=\;\alpha\;\left(1-\alpha\right)^{\frac{1-\alpha}{\nu+\alpha}}\;\Theta\left(\mathbf{\Gamma},\mathbf{N}_{t}\right)^{\frac{1+\nu}{\nu+\alpha}}\:K_{t}^{-\nu\frac{1-\alpha}{\nu+\alpha}}.
\]
Let $\underline{R}\left(\Gamma,n\right)$ and $\overline{R}\left(\Gamma,n\right)$ be the rental rates at $\underline{K}\left(\Gamma,n\right)$ and $\overline{K}\left(\Gamma,n\right)$ respectively. Then, multiplicity obtains if there exists an $n \in \mathbb{N}$ such that

\[
\begin{array}{rl}
 & \overline{R}\left(\Gamma,n\right)<\underbrace{\beta^{-1}-\left(1-\delta\right)}_{R^{*}}<\underline{R}\left(\Gamma,n+1\right)\\[1ex]
\Leftrightarrow & \;\Theta\left(\Gamma,n\right)^{\frac{1+\nu}{\nu+\alpha}}\:\overline{K}\left(\Gamma,n\right)^{-\nu\frac{1-\alpha}{\nu+\alpha}}<\dfrac{\beta^{-1}-\left(1-\delta\right)}{\alpha\;\left(1-\alpha\right)^{\frac{1-\alpha}{\nu+\alpha}}}<\;\Theta\left(\Gamma,n+1\right)^{\frac{1+\nu}{\nu+\alpha}}\:\underline{K}\left(\Gamma,n+1\right)^{-\nu\frac{1-\alpha}{\nu+\alpha}}.
\end{array}
\]

% Part 2: both bounds are strictly decreasing in the fixed cost so define c lowerbar and c upperbar such that the inequality stated becomes equality on either side
\end{proof}

\subsubsection*{Proof of Lemma \ref{lemma:MPS_theta}}

\begin{proof}
When all industries are identical and have $n$ firms, the factor price index is equal to
\begin{align}
\Theta\left(\Gamma_n,n\right)=\dfrac{n-\left(1-\rho\right)}{\sum\limits_{k=1}^{n}\dfrac{1}{\gamma_{k}}}
\end{align}
As $\Theta$ is a concave function of $\gamma_k$, by the definition of MPS, we have that if $\tilde \Gamma$ is a MPS of $\Gamma$, then $\Theta(\tilde \Gamma,n)<\Theta(\Gamma,n)$.
\end{proof}

\subsubsection*{Proof of Proposition \ref{prop:MPS}}

\begin{proof}
a) Let $K^{*}_n$ be a steady-state where all industries are have $n$ firms and common productivity distribution $\Gamma_n$. Using equation (\ref{eq:factor_demand}), we can define $K^{*}_n$ as
\begin{align}
R^{*}\:=\:\alpha\:\left(1-\alpha\right)^{\left(1-\alpha\right)/\left(\nu+\alpha\right)}\:\Theta\left(\Gamma_n,n\right)^{\left(\nu+1\right)/\left(\nu+\alpha\right)}\:\left(K^{*}_n\right)^{-\nu\left(1-\alpha\right)/\left(\nu+\alpha\right)}
\end{align}
Recall from Lemma \ref{lemma:MPS_theta} that $\Theta\left(\Gamma_n,n\right)$ declines after a MPS on $\Gamma_n$. Then $K^{*}_n$ must also decline.

b)
We provide a sufficient condition under which the unstable steady-state increases after an MPS. Note that the unstable steady-state increases whenever the increasing segment of the rental rate map lies strictly underneath the original one.

We know from the proof of Proposition \ref{prop:MPS}.a that the new rental rate at $\underline{K}\left(2\right)$ is strictly lower than before. The proof involves two steps

[A] We derive a sufficient condition under which the new rental rate at $\overline{K}\left(1\right)$ is lower than before

[B] We show that the increasing segment of the rental rate map after an MPS cannot cross the previous one more than once. Thus, if the new segment starts and ends below the previous one, it can never go above it.

\subsubsection*{Proof of Part A}

The free entry condition is
\begin{align}
\Lambda\left(n\right)\Theta\left(n-1\right)^{-\frac{\rho}{1-\rho}}\:\Phi\left(n-1\right)K^{\alpha}\:L^{1-\alpha}\;=\;c_{f}
\end{align}
Using
\begin{align}
L=\left[\left(1-\alpha\right)\Theta\left(n-1\right)\right]^{\frac{1}{\nu+\alpha}}K^{\frac{\alpha}{\nu+\alpha}}
\end{align}
we can rewrite the free-entry condition as
\begin{align}\nonumber
 & \Lambda\left(n\right)\Theta\left(n-1\right)^{-\frac{\rho}{1-\rho}}\:\Phi\left(n-1\right)\;K^{\alpha}\:\left[\left(1-\alpha\right)\Theta\left(n-1\right)\right]^{\frac{1-\alpha}{\nu+\alpha}}K^{\alpha\frac{1-\alpha}{\nu+\alpha}}\;=\;c_{f}\\\nonumber
\Leftrightarrow & \Lambda\left(n\right)\Theta\left(n-1\right)^{-\frac{\rho}{1-\rho}}\:\Phi\left(n-1\right)\left[\left(1-\alpha\right)\Theta\left(n-1\right)\right]^{\frac{1-\alpha}{\nu+\alpha}}K^{\alpha\frac{\nu+1}{\nu+\alpha}}\;=\;c_{f}\\
\Leftrightarrow & K\;=\;\left[\dfrac{c_{f}\left(1-\alpha\right)^{-\frac{1-\alpha}{\nu+\alpha}}}{\Lambda\left(n\right)\Theta\left(n-1\right)^{\frac{1-\alpha}{\nu+\alpha}-\frac{\rho}{1-\rho}}\:\Phi\left(n-1\right)}\right]^{\frac{1}{\alpha}\frac{\nu+\alpha}{\nu+1}}
\end{align}
The interest rate is
\begin{align}\nonumber
R= & \alpha\:\Theta\left(n-1\right)\:K^{\alpha-1}\:L^{1-\alpha}\\\nonumber
= & \alpha\:\Theta\left(n-1\right)\:K^{\alpha-1}\:\left[\left(1-\alpha\right)\Theta\left(n-1\right)\right]^{\frac{1-\alpha}{\nu+\alpha}}K^{\alpha\frac{1-\alpha}{\nu+\alpha}}\\
= & \alpha\:\left(1-\alpha\right)^{\frac{1-\alpha}{\nu+\alpha}}\:\Theta\left(\mathbf{\Gamma},\mathbf{N}_{t}\right)^{\frac{\nu+1}{\nu+\alpha}}\:K^{\nu\frac{\alpha-1}{\nu+\alpha}}
\end{align}
Putting the two together
\begin{equation}
R=\alpha\:\left(1-\alpha\right)^{\frac{1-\alpha}{\nu+\alpha}}\:\Theta\left(n-1\right)^{\frac{\nu+1}{\nu+\alpha}}\:\left(\dfrac{\Lambda\left(n\right)\Theta\left(n-1\right)^{\frac{1-\alpha}{\nu+\alpha}-\frac{\rho}{1-\rho}}\:\Phi\left(n-1\right)}{c_{f}\left(1-\alpha\right)^{-\frac{1-\alpha}{\nu+\alpha}}}\right)^{\frac{\nu}{\nu+1}\frac{1-\alpha}{\alpha}}\label{eq:R_1}
\end{equation}
implying
\begin{align}
R^{\frac{\nu+1}{\nu}\frac{\alpha}{1-\alpha}}=\propto\:\Theta\left(n-1\right)^{\frac{\nu+1}{\nu}\frac{\alpha}{1-\alpha}\frac{\nu+1}{\nu+\alpha}}\:\Lambda\left(n\right)\Theta\left(n-1\right)^{\frac{1-\alpha}{\nu+\alpha}-\frac{\rho}{1-\rho}}\:\Phi\left(n-1\right)
\end{align}
where
\begin{align}
\Theta\left(n\right)= & g\left(n\right)\\
\Phi\left(n\right)= & \dfrac{1}{\sum\limits _{j=1}^{n}\dfrac{s_{j}}{\pi_{j}}}\\
\Lambda\left(n\right)= & s_{n}^{2}\left[g\left(n\right)\right]^{\frac{\rho}{1-\rho}}
\end{align}
We can thus rewrite (\ref{eq:R_1}) as
\begin{equation}
R^{\frac{\nu+1}{\nu}\frac{\alpha}{1-\alpha}}=g\left(n-1\right)^{\frac{\nu+1}{\nu}\frac{\alpha}{1-\alpha}\frac{\nu+1}{\nu+\alpha}+\frac{1-\alpha}{\nu+\alpha}}\:\dfrac{s_{n}^{2}\left[\dfrac{g\left(n\right)}{g\left(n-1\right)}\right]^{\frac{\rho}{1-\rho}}}{\sum\limits _{j=1}^{n-1}\dfrac{\hat{s}_{j}}{\pi_{j}}}\label{eq:R_2}
\end{equation}
where $\hat{s}_{j}$ is the market share of firm $j$ in an industry
with $n-1$ firms and $s_{j}$ is the market share of that firm when
there are $n$ player in the industry. We want to show that the expression
in (\ref{eq:R_2}) goes down when we do an MPS on $n$ firms. The
challenge is in the fact that the expression involves terms that refer
to $n-1$ industries.

Under $n=2$, we have
\begin{align}
g\left(1\right)= & \rho\,\pi_{1}\\
g\left(2\right)= & \dfrac{1+\rho}{\dfrac{1}{\pi_{1}}+\dfrac{1}{\pi_{2}}}
\end{align}
so that
\begin{align}\nonumber
R^{\frac{\alpha}{1-\alpha}}= & \left(\rho\,\pi_{1}\right)^{\frac{\nu+1}{\nu}\frac{\alpha}{1-\alpha}\frac{\nu+1}{\nu+\alpha}+\frac{1-\alpha}{\nu+\alpha}-\frac{\rho}{1-\rho}}\:\left(\dfrac{1+\rho}{\dfrac{1}{\pi_{1}}+\dfrac{1}{\pi_{2}}}\right)^{\frac{\rho}{1-\rho}}\dfrac{\left[1-\dfrac{1+\rho}{\dfrac{1}{\pi_{1}}+\dfrac{1}{\pi_{2}}}\dfrac{1}{\pi_{2}}\right]^{2}}{\dfrac{1}{\pi_{1}}}\\
%= & \propto\:\pi_{1}^{\frac{\nu+1}{\nu}\frac{\alpha}{1-\alpha}\frac{\nu+1}{\nu+\alpha}+\frac{1-\alpha}{\nu+\alpha}-\frac{\rho}{1-\rho}}\:\pi_{1}\left[1-\dfrac{1+\rho}{\dfrac{1}{\pi_{1}}+\dfrac{1}{\pi_{2}}}\dfrac{1}{\pi_{2}}\right]^{2}\left[\dfrac{1+\rho}{\dfrac{1}{\pi_{1}}+\dfrac{1}{\pi_{2}}}\right]^{\frac{\rho}{1-\rho}}\\
%= & \propto\pi_{1}^{\frac{\nu+1}{\nu}\frac{\alpha}{1-\alpha}\frac{\nu+1}{\nu+\alpha}+\frac{1-\alpha}{\nu+\alpha}-\frac{\rho}{1-\rho}}\:\dfrac{\pi_{1}^{2}}{\pi_{1}}\left[1-\dfrac{1+\rho}{\dfrac{\pi_{2}}{\pi_{1}}+1}\right]^{2}\left[\dfrac{1+\rho}{\dfrac{1}{\pi_{1}}+\dfrac{1}{\pi_{2}}}\right]^{\frac{\rho}{1-\rho}}\\
%= & \propto\pi_{1}^{\frac{\nu+1}{\nu}\frac{\alpha}{1-\alpha}\frac{\nu+1}{\nu+\alpha}+\frac{1-\alpha}{\nu+\alpha}-\frac{\rho}{1-\rho}-1}\:\left[\pi_{1}-\pi_{1}\dfrac{1+\rho}{\dfrac{\pi_{2}}{\pi_{1}}+1}\right]^{2}\left[\dfrac{1+\rho}{\dfrac{1}{\pi_{1}}+\dfrac{1}{\pi_{2}}}\right]^{\frac{\rho}{1-\rho}}\\
%= & \propto\pi_{1}^{\frac{\nu+1}{\nu}\frac{\alpha}{1-\alpha}\frac{\nu+1}{\nu+\alpha}+\frac{1-\alpha}{\nu+\alpha}-\frac{\rho}{1-\rho}-1}\:\left[\pi_{1}-\pi_{1}\dfrac{1+\rho}{\dfrac{2x-\pi_{1}}{\pi_{1}}+1}\right]^{2}\left[\dfrac{1+\rho}{\dfrac{1}{\pi_{1}}+\dfrac{1}{\pi_{2}}}\right]^{\frac{\rho}{1-\rho}}\\
= & \propto\pi_{1}^{\frac{\nu+1}{\nu}\frac{\alpha}{1-\alpha}\frac{\nu+1}{\nu+\alpha}+\frac{1-\alpha}{\nu+\alpha}-\frac{\rho}{1-\rho}-1}\:\left[\pi_{1}-\pi_{1}\dfrac{1+\rho}{\dfrac{2x}{\pi_{1}}}\right]^{2}\left[\dfrac{1+\rho}{\dfrac{1}{\pi_{1}}+\dfrac{1}{2x-\pi_{1}}}\right]^{\frac{\rho}{1-\rho}}
\end{align}
The last term is decreasing on an MPS, since it is simply $g\left(2\right)$.
The first term is decreasing on an MPS provided that
\begin{align}
1+\dfrac{\rho}{1-\rho}>\dfrac{\nu+1}{\nu}\dfrac{\alpha}{1-\alpha}\dfrac{\nu+1}{\nu+\alpha}+\dfrac{1-\alpha}{\nu+\alpha}
%\Leftrightarrow & \dfrac{1}{1-\rho}>\dfrac{\alpha\left(\nu+1\right)^{2}+\left(1-\alpha\right)^{2}\nu}{\nu\left(1-\alpha\right)\left(\nu+\alpha\right)}\\
%\Leftrightarrow & \dfrac{1}{1-\rho}>\dfrac{\alpha\left(\nu+1\right)^{2}+\left(1-\alpha\right)^{2}\nu}{\nu\left(1-\alpha\right)\left(\nu+\alpha\right)}\\
%\Leftrightarrow & \rho>1-\dfrac{\nu\left(1-\alpha\right)\left(\nu+\alpha\right)}{\alpha\left(\nu+1\right)^{2}+\left(1-\alpha\right)^{2}\nu}\\
%\Leftrightarrow & \rho>1-\nu\dfrac{1-\alpha}{1+\nu\alpha}\\
\Leftrightarrow  \alpha<\dfrac{\nu+\rho-1}{\nu\left(2-\rho\right)}
\end{align}
since this MPS must result in higher $\pi_{1}$. We just need to evaluate
the term in the middle. Note that we can rewrite it as
\begin{align}
\pi_{1}-\pi_{1}^{2}\dfrac{1+\rho}{2x}
\end{align}
where $2x\equiv\pi_{1}+\pi_{2}$ is fixed by construction. The derivative
of the expression above is
\begin{align}
\dfrac{\partial}{\partial\pi_{1}}= & 1-2\pi_{1}\dfrac{1+\rho}{2x}\\
= & 1-\underbrace{\dfrac{\pi_{1}}{x}}_{>1}\left(1+\rho\right)<0
\end{align}
Therefore, for $n=2$, the interest rate is always declining on an
MPS provided that
\begin{align}
\rho>1-\nu\dfrac{1-\alpha}{1+\nu\alpha}
\end{align}

\subsubsection*{Proof of Part B}
Recall that the free entry condition is
\begin{align}
\Lambda_{j}\Theta^{-\frac{\rho}{1-\rho}}\:\Phi\:K^{\alpha}\:L^{1-\alpha}=c_{f}
\end{align}

Aggregate TFP can be written as
\hspace{-5cm}
\begin{align*}
\Phi= & \dfrac{\left\{ \left(1-m\right)\left[g\left(n-1\right)\right]^{\frac{\rho}{1-\rho}}+m\left[g\left(n\right)\right]^{\frac{\rho}{1-\rho}}\right\} ^{\frac{1}{\rho}}}{\left(1-m\right)\left[g\left(n-1\right)\right]^{\frac{1}{1-\rho}}h\left(n-1\right)+m\left[g\left(n\right)\right]^{\frac{1}{1-\rho}}h\left(n\right)} \\
& = \dfrac{\Theta^{\frac{1}{1-\rho}}}{\left(1-m\right)\left[g\left(n-1\right)\right]^{\frac{1}{1-\rho}}h\left(n-1\right)+m\left[g\left(n\right)\right]^{\frac{1}{1-\rho}}h\left(n\right)}
\end{align*}
where
\begin{align}
g\left(n\right)= & \dfrac{n-\left(1-\rho\right)}{\sum\limits _{j=1}^{n}\dfrac{1}{\pi_{j}}}\\
h\left(n\right)= & \sum\limits _{j=1}^{n}\dfrac{s_{j}}{\pi_{j}}
\end{align}
Now suppose that we do the MPS and have $\tilde{\Theta}=\Theta$ at
the same $K$.\footnote{We also have $\tilde{L}=L$, since $L$ is a function of $\Theta$
and $K$.} From the free entry condition and the expression for $\Phi$, this
is possible if
\begin{align}\nonumber
 & \dfrac{\Lambda_{j}}{\tilde{\Lambda}_{j}}=\dfrac{\left(1-{\color{red}m}\right)\left[g\left(n-1\right)\right]^{\frac{1}{1-\rho}}h\left(n-1\right)+{\color{red}m}\left[g\left(n\right)\right]^{\frac{1}{1-\rho}}h\left(n\right)}{\left(1-{\color{red}\tilde{m}}\right)\left[\tilde{g}\left(n-1\right)\right]^{\frac{1}{1-\rho}}\tilde{h}\left(n-1\right)+{\color{red}\tilde{m}}\left[\tilde{g}\left(n\right)\right]^{\frac{1}{1-\rho}}\tilde{h}\left(n\right)}\\
\Leftrightarrow & \dfrac{\Lambda_{j}}{\tilde{\Lambda}_{j}}=\dfrac{\left[g\left(n-1\right)\right]^{\frac{1}{1-\rho}}h\left(n-1\right)+{\color{red}m}\left\{ \left[g\left(n\right)\right]^{\frac{1}{1-\rho}}h\left(n\right)-\left[g\left(n-1\right)\right]^{\frac{1}{1-\rho}}h\left(n-1\right)\right\} }{\left[\tilde{g}\left(n-1\right)\right]^{\frac{1}{1-\rho}}\tilde{h}\left(n-1\right)+{\color{red}\tilde{m}}\left\{ \left[\tilde{g}\left(n\right)\right]^{\frac{1}{1-\rho}}\tilde{h}\left(n\right)-\left[\tilde{g}\left(n-1\right)\right]^{\frac{1}{1-\rho}}\tilde{h}\left(n-1\right)\right\} }
\end{align}
Rearranging this equation, we can write
\begin{equation}
\tilde{m}=a_{1}+b_{1}\cdot m\label{eq:eq_1}
\end{equation}
where $a_{1}$ and $b_{1}$ are some numbers (independent of $K$).

Furthermore, from $\tilde{\Theta}=\Theta$ we have
\begin{align}\nonumber
 & \left(1-{\color{red}m}\right)\left[g\left(n-1\right)\right]^{\frac{\rho}{1-\rho}}+{\color{red}m}\left[g\left(n\right)\right]^{\frac{\rho}{1-\rho}}=\left(1-{\color{red}\tilde{m}}\right)\left[\tilde{g}\left(n-1\right)\right]^{\frac{\rho}{1-\rho}}+{\color{red}\tilde{m}}\left[\tilde{g}\left(n\right)\right]^{\frac{\rho}{1-\rho}}\\
\Leftrightarrow & \left[g\left(n-1\right)\right]^{\frac{\rho}{1-\rho}}+{\color{red}m}\left\{ \left[g\left(n\right)\right]^{\frac{\rho}{1-\rho}}-\left[g\left(n-1\right)\right]^{\frac{\rho}{1-\rho}}\right\} =\left[\tilde{g}\left(n-1\right)\right]^{\frac{\rho}{1-\rho}}+{\color{red}\tilde{m}}\left\{ \left[\tilde{g}\left(n\right)\right]^{\frac{\rho}{1-\rho}}-\left[\tilde{g}\left(n-1\right)\right]^{\frac{\rho}{1-\rho}}\right\} 
\end{align}
Rearranging this equation, we can write
\begin{equation}
\tilde{m}=a_{2}+b_{2}\cdot m\label{eq:eq_2}
\end{equation}
Combining (\ref{eq:eq_1}) and (\ref{eq:eq_2}), there is at most
one pair $\left(m,\tilde{m}\right)$ such that $\tilde{\Theta}=\Theta$.
This establishes that $\tilde{\Theta}$ cannot cross $\Theta$ twice.
\end{proof}

\begin{prop}[Mean Preserving Spread and Fragility, general $n$] \label{prop:MPS_BA_n}

Let $\eta = 1$ and suppose that all industries are identical to start ($\gamma_{ij} = \gamma_{j} \; \forall i$). Let ${K}^{*}\left(n\right)$ be a steady-state with $n$ firms. Let $\lambda$ be a mean-preserving spread on the distribution $\left\{\gamma_1,\ldots,\gamma_n\right\}$ of active firms, such that for any $j=1,\ldots,n-1$, $\gamma_{1}/\gamma_{j}$ is unchanged. Then, if
\begin{align}
\rho>\dfrac{1+\nu\alpha}{1+\nu}\end{align}
we have that
\begin{align} \dfrac{\partial \underline{B}\left(n\right)}{\partial\lambda} > 0. \end{align}
\end{prop}

\begin{proof}[Proof of Proposition \ref{prop:MPS_BA_n}]

Let us now provide a sufficient condition for general $n$. First
note that we can write (\ref{eq:R_2}) as
\begin{align}
R^{\frac{\nu+1}{\nu}\frac{\alpha}{1-\alpha}}=\underbrace{g\left(n-1\right)^{\frac{\nu+1}{\nu}\frac{\alpha}{1-\alpha}\frac{\nu+1}{\nu+\alpha}+\frac{1-\alpha}{\nu+\alpha}-\frac{\rho}{1-\rho}}g\left(n\right)^{\frac{\rho}{1-\rho}}}_{v}\underbrace{\dfrac{1}{\sum\limits _{j=1}^{n-1}\dfrac{\hat{s}_{j}}{\pi_{j}}}s_{n}^{2}}_{z}
\end{align}
\begin{align}
R^{\frac{\alpha}{1-\alpha}}=\underbrace{g\left(n-1\right)^{\frac{\alpha}{1-\alpha}-\frac{\rho}{1-\rho}}g\left(n\right)^{\frac{\rho}{1-\rho}}}_{v}\underbrace{\dfrac{1}{\sum\limits _{j=1}^{n-1}\dfrac{\hat{s}_{j}}{\pi_{j}}}s_{n}^{2}}_{z}
\end{align}
The first term $v$ is always decreasing on an MPS provided that

\begin{align}
 \dfrac{\rho}{1-\rho}>\dfrac{\nu+1}{\nu}\dfrac{\alpha}{1-\alpha}\dfrac{\nu+1}{\nu+\alpha}+\dfrac{1-\alpha}{\nu+\alpha}
%\Leftrightarrow & \dfrac{\nu\left(1-\alpha\right)\left(\nu+\alpha\right)}{\alpha\left(\nu+1\right)^{2}+\left(1-\alpha\right)^{2}\nu}>\dfrac{1-\rho}{\rho}\\
%\Leftrightarrow & \dfrac{\nu\left(1-\alpha\right)\left(\nu+\alpha\right)}{\alpha\left(\nu+1\right)^{2}+\left(1-\alpha\right)^{2}\nu}>\dfrac{1}{\rho}-1\\
%\Leftrightarrow & \dfrac{1}{\rho}<\nu\dfrac{1-\alpha}{1+\nu\alpha}+1\\
%\Leftrightarrow & \rho>\dfrac{1+\nu\alpha}{1+\nu}\\
\Leftrightarrow  \alpha<\dfrac{\rho\left(1+\nu\right)-1}{\nu}
\end{align}
To see it note that $g\left(n\right)$ is decreasing on an MPS. If
$g\left(n-1\right)$ is increasing on an MPS, it immediately follows
that $v$ decreases on an MPS when the above condition is satisfied.
If $g\left(n-1\right)$ is instead decreasing on an MPS, just rewrite
$v$ as
\begin{align}
v=g\left(n-1\right)^{\frac{\nu+1}{\nu}\frac{\alpha}{1-\alpha}\frac{\nu+1}{\nu+\alpha}+\frac{1-\alpha}{\nu+\alpha}}\left[\dfrac{g\left(n\right)}{g\left(n-1\right)}\right]^{\frac{\rho}{1-\rho}}
\end{align}

and note that $\dfrac{g\left(n\right)}{g\left(n-1\right)}$ decreases
on an MPS.

Thus, all we need to show is that $z$ is also decreasing on an MPS.
Note that we can write $z$ as
\begin{align}
z=\dfrac{s_{n}^{2}}{\sum\limits _{j=1}^{n-1}\dfrac{\hat{s}_{j}}{\pi_{j}}}=\dfrac{1}{\sum\limits _{j=1}^{n-1}\dfrac{\hat{s}_{j}}{\pi_{j}}\dfrac{1}{s_{n}^{2}}}
\end{align}
We know that $s_{n}$ is decreasing on an MPS. A sufficient condition
for $z$ to be decreasing on an MPS is that
\begin{align}
\dfrac{\hat{s}_{j}}{\pi_{j}}\dfrac{1}{s_{n}^{2}}
\end{align}
is increasing on an MPS for every $j=1,2,\ldots,n-1$.

Consider an MPS such that
\begin{align}
\widetilde{\pi}_{j}=\gamma\,\pi_{j}\quad\forall j=1,2,\ldots,n-1
\end{align}
and 
\begin{align}
 & \gamma\sum\limits _{j=1}^{n-1}\pi_{j}+\widetilde{\pi}_{n}=\sum\limits _{j=1}^{n-1}\pi_{j}+\pi_{n}\\
\Leftrightarrow & \widetilde{\pi}_{n}=\pi_{n}-\left(\gamma-1\right)\sum\limits _{j=1}^{n-1}\pi_{j}
\end{align}
In this case we have
\begin{align}
\dfrac{1}{\gamma}\underbrace{\dfrac{\hat{s}_{j}}{\pi_{j}}}_{\text{const}}\dfrac{1}{\widetilde{s}_{n}^{2}}
\end{align}
We need to show that 
\begin{align}
\gamma\underbrace{\left[1-\dfrac{n-\left(1-\rho\right)}{\sum\limits _{j=1}^{n-1}\dfrac{1}{\gamma\pi_{j}}+1}\dfrac{1}{\pi_{n}-\left(\gamma-1\right)\sum\limits _{j=1}^{n-1}\pi_{j}}\right]^{2}}_{\widetilde{s}_{n}}
\end{align}
decreases in $\gamma$. Note that we can rewrite it as
\begin{align}
 \gamma\underbrace{\left[1-\dfrac{n-\left(1-\rho\right)}{\sum\limits _{j=1}^{n-1}\dfrac{\pi_{n}-\left(\gamma-1\right)\sum\limits _{j=1}^{n-1}\pi_{j}}{\gamma\,\pi_{j}}+1}\right]^{2}}_{\tilde{s}_{n}}
%= & \gamma\underbrace{\left[1-\dfrac{n-\left(1-\rho\right)}{\dfrac{\pi_{n}-\left(\gamma-1\right)\sum\limits _{j=1}^{n-1}\pi_{j}}{\gamma}\sum\limits _{j=1}^{n-1}\dfrac{1}{\pi_{j}}+1}\right]^{2}}_{\tilde{s}_{n}}\\
%= & \gamma\underbrace{\left[1-\dfrac{n-\left(1-\rho\right)}{\left[\dfrac{\pi_{n}}{\gamma}-\left(1-\dfrac{1}{\gamma}\right)\sum\limits _{j=1}^{n-1}\pi_{j}\right]\sum\limits _{j=1}^{n-1}\dfrac{1}{\pi_{j}}+1}\right]^{2}}_{\tilde{s}_{n}}\\
= \gamma\underbrace{\left[1-\dfrac{n-\left(1-\rho\right)}{\left[\dfrac{1}{\gamma}\left(\pi_{n}+\sum\limits _{j=1}^{n-1}\pi_{j}\right)-\sum\limits _{j=1}^{n-1}\pi_{j}\right]\sum\limits _{j=1}^{n-1}\dfrac{1}{\pi_{j}}+1}\right]^{2}}_{\tilde{s}_{n}}
\end{align}
The derivative with respect to $\gamma$ is
\begin{align}
\tilde{s}_{n}^{2}+\gamma2\tilde{s}_{n}\left\{ -\left(-1\right)\left[n-\left(1-\rho\right)\right]\dfrac{\left(\pi_{n}+\sum\limits _{j=1}^{n-1}\pi_{j}\right)\sum\limits _{j=1}^{n-1}\dfrac{1}{\pi_{j}}\left(-\dfrac{1}{\gamma^{2}}\right)}{\left(\left[\dfrac{1}{\gamma}\left(\pi_{n}+\sum\limits _{j=1}^{n-1}\pi_{j}\right)-\sum\limits _{j=1}^{n-1}\pi_{j}\right]\sum\limits _{j=1}^{n-1}\dfrac{1}{\pi_{j}}+1\right)^{2}}\right\} 
\end{align}
which is lower than zero if
\begin{align}
 & \tilde{s}_{n}-\dfrac{2}{\gamma}\left[\dfrac{n-\left(1-\rho\right)}{\sum\limits _{j=1}^{n}\dfrac{\tilde{\pi}_{n}}{\gamma\pi_{j}}}\dfrac{1}{\sum\limits _{j=1}^{n}\dfrac{\tilde{\pi}_{n}}{\gamma\pi_{j}}}\left(\pi_{n}+\sum\limits _{j=1}^{n-1}\pi_{j}\right)\sum\limits _{j=1}^{n-1}\dfrac{1}{\pi_{j}}\right]<0
%\Leftrightarrow & 1-\dfrac{n-\left(1-\rho\right)}{\sum\limits _{j=1}^{n}\dfrac{\tilde{\pi}_{n}}{\pi_{j}}}-2\gamma\left[\dfrac{n-\left(1-\rho\right)}{\sum\limits _{j=1}^{n}\dfrac{\tilde{\pi}_{n}}{\pi_{j}}}\dfrac{1}{\sum\limits _{j=1}^{n}\dfrac{\tilde{\pi}_{n}}{\pi_{j}}}\left(\sum\limits _{j=1}^{n}\pi_{j}\right)\sum\limits _{j=1}^{n-1}\dfrac{1}{\pi_{j}}\right]<0\\
\Leftrightarrow  1-\underbrace{\dfrac{n-\left(1-\rho\right)}{\sum\limits _{j=1}^{n}\dfrac{\tilde{\pi}_{n}}{\pi_{j}}}}_{\left(a\right)}\left[1+2\gamma\underbrace{\dfrac{\sum\limits _{j=1}^{n}\pi_{j}}{\tilde{\pi}_{n}}}_{>n}\underbrace{\dfrac{\sum\limits _{j=1}^{n-1}\dfrac{1}{\pi_{j}}}{\sum\limits _{j=1}^{n}\dfrac{1}{\pi_{j}}}}_{\left(b\right)}\right]<0
\end{align}

If suffices to prove that $\left(a\right)>1/3$ and that $\left(b\right)>1/n$.

To prove the first, note that
\begin{align}
\tilde{s}_{n}=\dfrac{1}{1-\rho}\left[1-\dfrac{n-\left(1-\rho\right)}{\sum\limits _{j=1}^{n}\dfrac{\tilde{\pi}_{n}}{\pi_{j}}}\right]<\dfrac{1}{3}
%\Leftrightarrow & 1-\dfrac{n-\left(1-\rho\right)}{\sum\limits _{j=1}^{n}\dfrac{\tilde{\pi}_{n}}{\pi_{j}}}<\dfrac{1-\rho}{3}\\
%\Leftrightarrow & \dfrac{3-1+\rho}{3}<\dfrac{n-\left(1-\rho\right)}{\sum\limits _{j=1}^{n}\dfrac{\tilde{\pi}_{n}}{\pi_{j}}}\\
\Leftrightarrow  \underbrace{\dfrac{n-\left(1-\rho\right)}{\sum\limits _{j=1}^{n}\dfrac{\tilde{\pi}_{n}}{\pi_{j}}}}_{\left(a\right)}>\dfrac{2+\rho}{3}>\dfrac{1}{3}
\end{align}
To prove the second, note that
\begin{align}
 \dfrac{\sum\limits _{j=1}^{n-1}\dfrac{1}{\pi_{j}}}{\sum\limits _{j=1}^{n}\dfrac{1}{\pi_{j}}}>\dfrac{1}{n}
%\Leftrightarrow & n\sum\limits _{j=1}^{n-1}\dfrac{1}{\pi_{j}}>\sum\limits _{j=1}^{n}\dfrac{1}{\pi_{j}}\\
%\Leftrightarrow & n\left(\sum\limits _{j=1}^{n}\dfrac{1}{\pi_{j}}-\dfrac{1}{\pi_{n}}\right)>\sum\limits _{j=1}^{n}\dfrac{1}{\pi_{j}}\\
%\Leftrightarrow & \left(n-1\right)\sum\limits _{j=1}^{n}\dfrac{1}{\pi_{j}}>n\dfrac{1}{\pi_{n}}\\
\Leftrightarrow  \sum\limits _{j=1}^{n}\dfrac{\pi_{n}}{\pi_{j}}>\dfrac{n}{n-1}
\end{align}
The last equation is implied by the fact that
\begin{align}
  1-\dfrac{n-\left(1-\rho\right)}{\sum\limits _{j=1}^{n}\dfrac{\pi_{n}}{\pi_{j}}}>0 \Leftrightarrow  \sum\limits _{j=1}^{n}\dfrac{\pi_{n}}{\pi_{j}}>\underbrace{n-\left(1-\rho\right)}_{>2\;\text{under}\;n\geq3}
\end{align}
which is needed for $s_{n}>0$. This completes the proof.
\end{proof}

\subsubsection*{Proof of Proposition \ref{prop:basin_attraction_cf}}

\begin{proof}

% In a steady-state with identical industries and $n$ firms per industry we have that
% \begin{align}
% \begin{array}{rl}
% R^{*}= & \alpha\left(1-\alpha\right)^{\frac{1-\alpha}{\nu+\alpha}}\;\left[\Theta\left(n\right)\right]^{\frac{1+\nu}{\nu+\alpha}}\;\left[K^{*}\left(n\right)\right]^{\left(1-\alpha\right)\frac{-\nu}{\nu+\alpha}}\\
% R^{*}= & \beta^{-1}+\left(1-\delta\right)
% \end{array}
% \end{align}
% The first equation describes capital demand by fimrs, whereas the second evaluates the Euler equation (in a steady-state).
% $K^{*}\left(n\right)$ is therefore independent of $c_f$ \textendash{} provided that all $n$ make strictly positive profits, a marginal increase in $c_f$ will not drive any of them out of the market.

% Note furthermore that $\underline{K}\left(n\right)$ is increasing in $n$ (Appendix \ref{subsec:numb-active-firms}).
% \begin{align}
% \underline{K}\left(n\right) = \left\{ \dfrac{c} {\varLambda\left(n,n\right)} \left(1-\alpha\right)^{-\frac{1-\alpha}{\nu+\alpha}}\left[\Phi\left(n\right)\right]^{-1}\left[\Theta\left(n\right)\right]^{\frac{\rho}{1-\rho}-\frac{1-\alpha}{\nu+\alpha}}\right\} ^{\frac{\nu+\alpha}{\alpha\left(1+\nu\right)}} 
% \end{align}

From equation (\ref{eq:factor_demand}) we can write
\begin{align}
R_{t}\:=\:\alpha\:\left(1-\alpha\right)^{\left(1-\alpha\right)/\left(\nu+\alpha\right)}\:\Theta\left(\mathbf{\Gamma},\mathbf{N}_{t}\right)^{\left(\nu+1\right)/\left(\nu+\alpha\right)}\:K_{t}^{-\nu\left(1-\alpha\right)/\left(\nu+\alpha\right)}
\end{align}
where $\Theta \left(\mathbf{\Gamma}, \mathbf{N}_{t}\right) $ is increasing in the number of active firms (as explained above). For a given steady-state $K^*$, the slackness free entry condition may or may not hold exactly. If it does hold exactly then, in response to a marginal increase in $c$, the number of firms will necessarily decrease and so will the level of capital at the steady-state. If it does not hold exactly then the level of capital will be unchanged as no firm will leave the market. The statement of part a) follows.

Second, at an unstable steady-state $K_{U}$, the rental rate is increasing in the capital stock. For this to happen, $\Theta\left(\mathbf{\Gamma}, \mathbf{N}_{t}\right)$ must be increasing in $K$ at that point. Assuming $I$ large, this only happens if some firm is exactly breaking even. Therefore, the rental rate at an unstable steady-state $K_{U}$ necessarily declines after an increase in $c$, as stated in part b).

\end{proof}

%\section{Derivation and Proofs: General Equilibrium}

% \subsection{Steady-State\label{subsec:Steady-State}}

% \subsubsection*{Example with Unique Steady-State}
% \begin{figure}[ht]
% \begin{centering}
% \includegraphics*[scale=0.5]{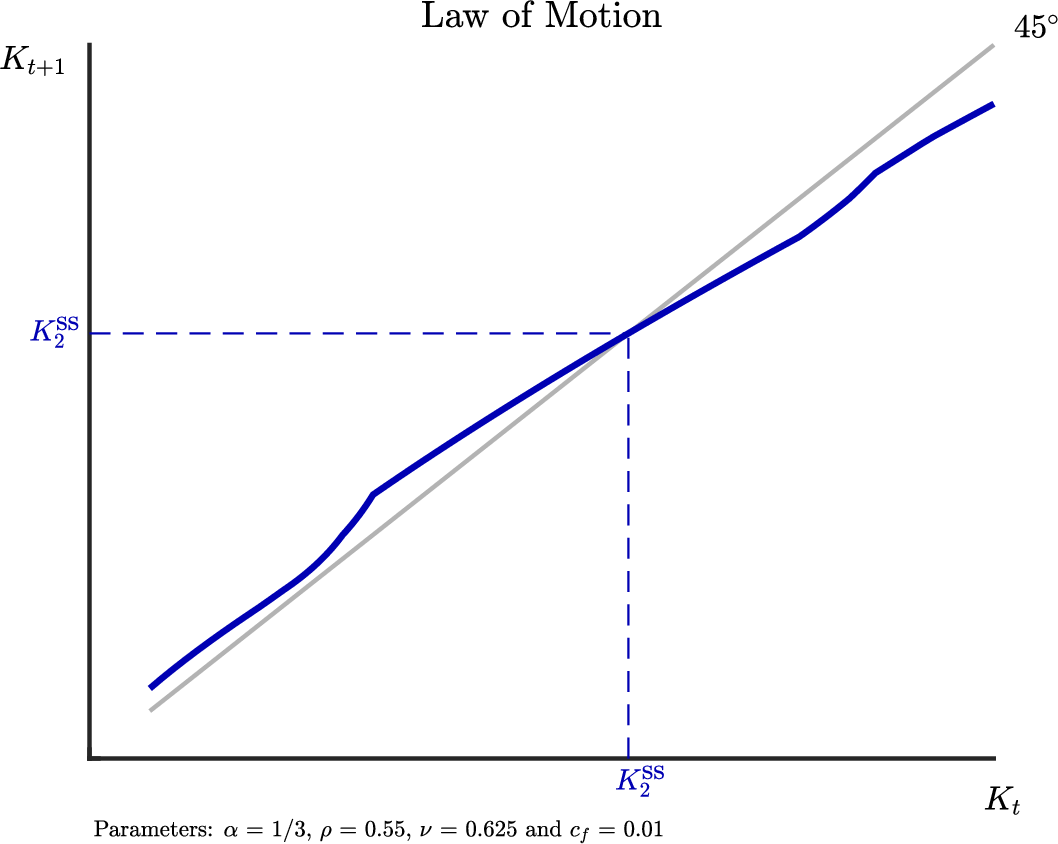}
% \par\end{centering}
% \caption{Economy with Unique Steady-State\label{fig:Unique_ss}}
% \end{figure}

% \subsubsection*{Example with Three Steady-State}
% \begin{figure}[ht]
% \begin{centering}
% \includegraphics*[scale=0.5]{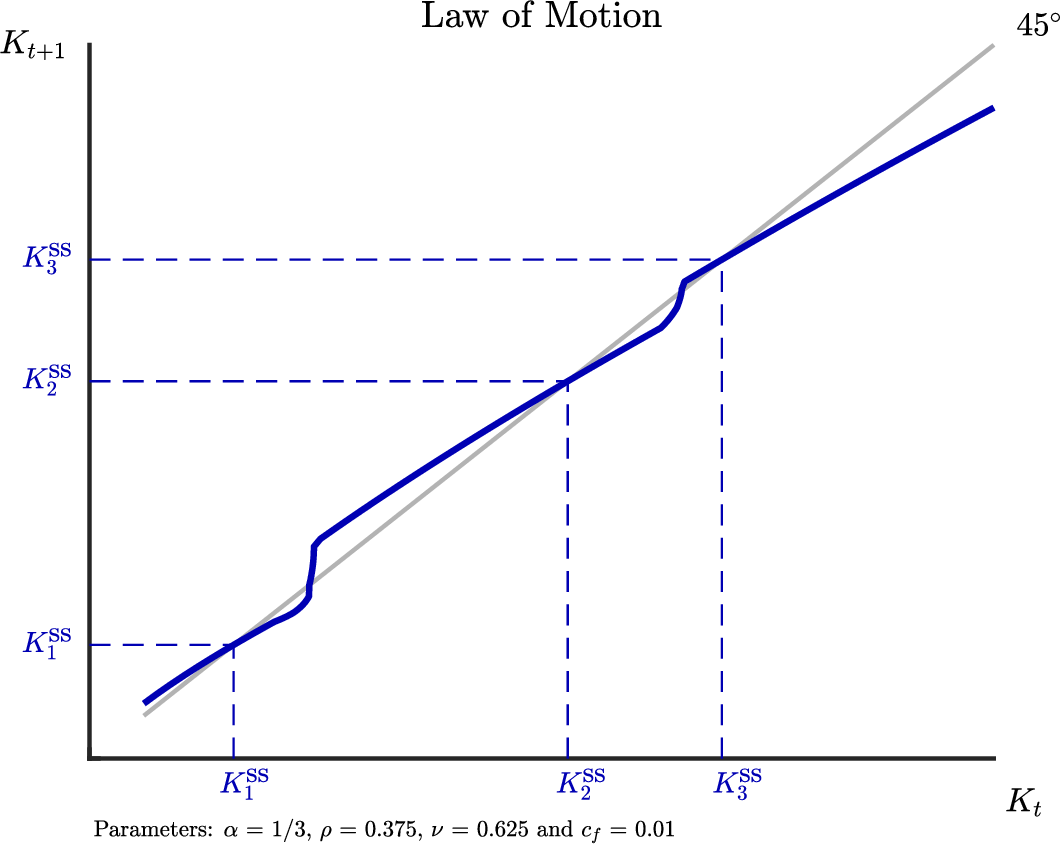}
% \par\end{centering}
% \caption{Economy with Three Steady-States\label{fig:Three_ss}}
% \end{figure}

\newpage

\section{Robustness: Different Elasticities of Substitution \label{subsec:new-calibration-ES}}

\subsubsection*{Calibration}
Parameters not reported are as in the baseline calibration (Table \ref{tab:parameter_values}).
\begin{table}[H]
\setlength{\tabcolsep}{0.2cm} \begin{center} \resizebox{14cm}{5cm} {  \begin{tabular}{lccl}
\thickhline
\\[-1ex]
{\large Description} & {\large Parameter} & {\large Value} & {\large Source/Target} \\[1ex] \thickhline
\\[-1ex]
Between-industry ES & $\sigma_{I}$ & 1.2 & \cite{de2021quantifying} \\
\\[-1ex]
Within-industry ES & $\sigma_{G}$ & 5.75 & \cite{de2021quantifying} \\
\\[-1ex]
\hline
\\[-1ex]
Calibrated Parameters: 2007 \\ \\[-1ex] \hline
\\[-2ex]
Standard deviation $\gamma$ & $\lambda$ & 0.280 & Sales-weighted average markup\\
\\[-1ex]
Fixed cost & $c$ & 0.0034 & Average ratio fixed/total costs \\
\\[-1ex]
Fraction of industries with $c_{i}>0$ & $f$ & 0.080 &  Emp share concentrated industries \\
\\[-1ex]
Persistence of $z_t$  & $\rho_{z}$ & 0.900 & Autocorrelation of log Y \\
\\[-1ex]
Standard deviation of $\varepsilon_t$ & $\sigma_{\varepsilon}$ & 0.0035 & Standard deviation of log Y \\ 
\\[-1ex]
\hline
\\[-1ex]
Calibrated Parameters: 1985 \\ \\[-1ex] \hline
\\[-2ex]
Standard deviation $\gamma$ & $\lambda$ & 0.140 & Sales-weighted average markup\\
\\[-1ex]
Fixed cost & $c$ & 0.0004 & Average ratio fixed/total costs \\
\\[-1ex]
Fraction of industries with $c_{i}>0$ & $f$ & 0.110 &  Emp share concentrated industries \\
\\[-1ex]
\thickhline
\end{tabular}  
} \end{center}
\caption{Parameter Values\label{tab:parameter_values_ES}}
\end{table}

\begin{table}[H]
\setlength{\tabcolsep}{0.35cm}  
\begin{center}
\begin{tabular}{lccccc} 		\thickhline 
\\[-2ex]
& \multicolumn{2}{c}{1985} & & \multicolumn{2}{c}{2007} \\
\\[-1ex] 
& Data & Model & & Data & Model
\\ \hline  
\\[-1ex] 
Sales-weighted average markup & 1.27 & 1.25 & & 1.46 & 1.43 \\
\\[-1ex]
Average fixed to total cost ratio & 0.343 & 0.370 & & 0.414 & 0.479 \\
\\[-1ex]
Employment share in \textit{concentrated} industries & - & 0.058 & & 0.063 & 0.037 \\
\\[-1ex] \hline 
\\[-1ex]
Autocorrelation log GDP  & 0.978* & 0.953 & & 0.978* & 0.956 \\
\\[-1ex]
Standard deviation log GDP & 0.061* & 0.040 & & 0.061* & 0.059 \\
\\[-1ex]
\thickhline
\\[-1ex]
\multicolumn{6}{l}{*computed over 1947:Q1-2019:Q4} \\
\end{tabular} \end{center}
\caption{Targeted moments and model counterparts}
\end{table}

\subsubsection*{Ergodic Distributions}

\begin{figure}[H]
\hspace{-1cm}
\begin{minipage}[b]{.55\linewidth}
\centering\includegraphics*[scale=0.5]{input/hist_1985_ES.eps}\subcaption{Output Distribution: 1985} \label{fig:y_dist_1985_ES}
\end{minipage}%
\hspace{-0.5cm}
\begin{minipage}[b]{.55\linewidth}
\centering\includegraphics*[scale=0.5]{input/hist_2007_ES.eps}\subcaption{Output Distribution: 2007} \label{fig:y_dist_2007_ES}
\end{minipage}
\caption{Ergodic distribution of output \protect \\ {\small{} This figure shows the distribution of log output for the 1985 and the 2007 economies. We simulate each economy for 10,000,000 periods and plot output in deviation from the high steady state.}}
\end{figure}

\subsubsection*{The 2008 Crisis}

\begin{figure}[H]
\begin{minipage}[b]{.5\linewidth}
\centering{}\includegraphics*[scale=0.55]{input/GR_transition_2007_ES.eps}\subcaption{2007 Model  \\ This figures replicates Figure \ref{fig:GR_model} \label{fig:GR_model_07_ES}}
\end{minipage}%
\hspace{0.5cm}
\begin{minipage}[b]{.5\linewidth}
\centering{}\includegraphics*[scale=0.55]{input/GR_transition_1985_ES.eps}\subcaption{1985 Model  \\ This figures replicates Figure \ref{fig:GR_data_model_85_1} \label{fig:GR_model_85_ES}}
\end{minipage}
\caption{The \textit{great recession} and its aftermath}\label{fig:GR_data_model_ES}
\end{figure}

\newpage

\section{Robustness: Variable Fixed Costs} \label{sec:var_fixed_costs}

We assume that, each period, a fixed amount $c_f$ of firms' output is lost
\begin{align*}
    c_f=k_c^\alpha l_c^{1-\alpha}
\end{align*}

Given these assumptions, firms need to pay a per per period fixed cost
\[
\Theta_{t} \cdot c_f
\]
where $\Theta_{t} $ is the factor price index.

Denoting by $L_{yt}$ and $K_{yt}$ the aggregate stocks of labor and capital used in the production, we have the following market clearing conditions for labor and capital
\begin{align*}
    L_{t} = L_{yt} + N^{c}_{t} \cdot l_c \\
    K_{t} = K_{yt} + N^{c}_{t} \cdot k_c
\end{align*}
where $N^{c}$ denotes the number of firms incurring $c_f$. Note that the optimal mix of $l_c$ and $k_c$ chosen by each individual firm satisfies
\begin{align*}
    \dfrac{k_c}{l_c} = \dfrac{K_{yt}}{L_{yt}}
\end{align*}

\newpage
\subsubsection*{Calibration}
Parameters not reported are as in the baseline calibration (Table \ref{tab:parameter_values}).
\begin{table}[H]
\setlength{\tabcolsep}{0.2cm} \begin{center} \resizebox{14cm}{4.25cm} {  \begin{tabular}{lccl}
\thickhline
\\[-1ex]
{\large Description} & {\large Parameter} & {\large Value} & {\large Source/Target} \\[1ex] \thickhline
\\[-1ex]
Calibrated Parameters: 2007 \\ \\[-1ex] \hline
\\[-2ex]
Standard deviation $\gamma$ & $\lambda$ & 0.300 & Sales-weighted average markup\\
\\[-1ex]
Fixed cost & $c$ & 0.0007 & Average ratio fixed/total costs \\
\\[-1ex]
Fraction of industries with $c_{i}>0$ & $f$ & 0.150 &  Emp share concentrated industries \\
\\[-1ex]
Persistence of $z_t$  & $\rho_{z}$ & 0.920 & Autocorrelation of log Y \\
\\[-1ex]
Standard deviation of $\varepsilon_t$ & $\sigma_{\varepsilon}$ & 0.0035 & Standard deviation of log Y \\ 
\\[-1ex]
\hline
\\[-1ex]
Calibrated Parameters: 1985 \\ \\[-1ex] \hline
\\[-2ex]
Standard deviation $\gamma$ & $\lambda$ & 0.160 & Sales-weighted average markup\\
\\[-1ex]
Fixed cost & $c$ & 0.0004 & Average ratio fixed/total costs \\
\\[-1ex]
Fraction of industries with $c_{i}>0$ & $f$ & 0.130 &  Emp share concentrated industries \\
\\[-1ex]
\thickhline
\end{tabular}  
} \end{center}
\caption{Parameter Values}
\end{table}

\begin{table}[H]
\setlength{\tabcolsep}{0.35cm}  
\begin{center}
\begin{tabular}{lccccc} 		\thickhline 
\\[-2ex]
& \multicolumn{2}{c}{1985} & & \multicolumn{2}{c}{2007} \\
\\[-1ex] 
& Data & Model & & Data & Model
\\ \hline  
\\[-1ex] 
Sales-weighted average markup & 1.27 & 1.28 & & 1.46 & 1.47 \\
\\[-1ex]
Average fixed to total cost ratio & 0.343 & 0.377 & & 0.414 & 0.431 \\
\\[-1ex]
Employment share in \textit{concentrated} industries & - & 0.068 & & 0.063 & 0.066 \\
\\[-1ex] \hline 
\\[-1ex]
Autocorrelation log GDP  & 0.978* & 0.980 & & 0.978* & 0.972 \\
\\[-1ex]
Standard deviation log GDP & 0.061* & 0.087 & & 0.061* & 0.059 \\
\\[-1ex]
\thickhline
\\[-1ex]
\multicolumn{6}{l}{*computed over 1947:Q1-2019:Q4} \\
\end{tabular} \end{center}
\caption{Targeted moments and model counterparts}
\end{table}

\subsubsection*{Ergodic Distributions}

\begin{figure}[H]
\hspace{-1cm}
\begin{minipage}[b]{.55\linewidth}
\centering\includegraphics*[scale=0.5]{input/hist_1985_CD.eps}\subcaption{Output Distribution: 1985} \label{fig:y_dist_1985_CD}
\end{minipage}%
\hspace{-0.5cm}
\begin{minipage}[b]{.55\linewidth}
\centering\includegraphics*[scale=0.5]{input/hist_2007_CD.eps}\subcaption{Output Distribution: 2007} \label{fig:y_dist_2007_CD}
\end{minipage}
\caption{Ergodic distribution of output \protect \\ {\small{} This figure shows the distribution of log output for the 1985 and the 2007 economies. We simulate each economy for 10,000,000 periods and plot output in deviation from the high steady state.}}
\end{figure}

\subsubsection*{The 2008 Crisis}

\begin{figure}[H]
\begin{minipage}[b]{.5\linewidth}
\centering{}\includegraphics*[scale=0.55]{input/GR_transition_2007_CD.eps}\subcaption{2007 Model  \\ This figures replicates Figure \ref{fig:GR_model} \label{fig:GR_model_07_CD}}
\end{minipage}%
\hspace{0.5cm}
\begin{minipage}[b]{.5\linewidth}
\centering{}\includegraphics*[scale=0.55]{input/GR_transition_1985_CD.eps}\subcaption{1985 Model  \\ This figures replicates Figure \ref{fig:GR_data_model_85_1} \label{fig:GR_model_85_CD}}
\end{minipage}
\caption{The \textit{great recession} and its aftermath}\label{fig:GR_data_model_CD}
\end{figure}
